# Supplementary material for: Nonlinearity in the sequential absorption of multiple photons
Source: arXiv:1612.07105 ancillary file (2017-09-13)
Supplement: Supplementary file 1 [file NitrogenRateEquations.pdf]

# Rate-equation model for a nitrogen atom in LCLS radiation

Christian Buth, 04 December 2011

Argonne National Laboratory, Argonne, Illinois 60439, USA

Max-Planck-Institut für Kernphysik, Saupfercheckweg 1, 69117 Heidelberg, Germany

The PULSE Institute for Ultrafast Energy Science, SLAC National Accelerator Laboratory, Menlo Park, California 94025, USA

---

## Initialize package

```
BeginPackage["NitrogenRateEquations`"]
```

---

## Public section

```
NitrogenRateEquations::usage="NitrogenRateEquations implements a rate-equation " <>
    "model for the interaction of x rays with a single nitrogen atom."
```

---

## System of coupled differential equations

Index of initial value for the specified rate equation in the vector grndvec:

Neutral:        req223 - 1

Minus one: req213 - 2 req222 - 3 req123 - 4

Minus two: req212 - 5 req203 - 6 req221 - 7 req113 - 8 req122 - 9 req023 - 10

Minus three: req202 - 11 req211 - 12 req220 - 13 req103 - 14 req112 - 15 req121 - 16 req013 - 17 req022 - 18

Minus four: req201 - 19 req210 - 20 req102 - 21 req111 - 22 req120 - 23 req003 - 24 req012 - 25 req021 - 26

Minus five: req200 - 27 req101 - 28 req110 - 29 req011 - 30 req020 - 31 req002 - 32

Minus six: req100 - 33 req010 - 34 req001 - 35

Minus seven: req000 - 36

```
unitgrndvec[]:=Module[{i},
  Join[{1},Table[0,{i,1,35}]]
]

zerogrndvec[]:=Module[{i},
  Table[0,{i,1,36}]
]
```

P223[t],  
P213[t], P222[t], P123[t],  
P212[t], P203[t], P221[t], P113[t], P122[t], P023[t],  
P202[t], P211[t], P220[t], P103[t], P112[t], P121[t], P013[t], P022[t],  
P201[t], P210[t], P102[t], P111[t], P120[t], P003[t], P012[t], P021[t],  
P200[t], P101[t], P110[t], P011[t], P020[t], P002[t],  
P100[t], P010[t], P001[t],  
P000[t]

```

solgrndvec[sol_,t1_]:=({
  (* Neutral *)
  Replace[P223[t],sol[[1]]],
  (* Minus one *)
  Replace[P213[t],sol[[1]]],Replace[P222[t],sol[[1]]],Replace[P123[t],sol[[1]]],
  (* Minus two *)
  Replace[P212[t],sol[[1]]],Replace[P203[t],sol[[1]]],Replace[P221[t],sol[[1]]],
  Replace[P113[t],sol[[1]]],Replace[P122[t],sol[[1]]],Replace[P023[t],sol[[1]]],
  (* Minus three *)
  Replace[P202[t],sol[[1]]],Replace[P211[t],sol[[1]]],Replace[P220[t],sol[[1]]],
  Replace[P103[t],sol[[1]]],Replace[P112[t],sol[[1]]],Replace[P121[t],sol[[1]]],
  Replace[P013[t],sol[[1]]],Replace[P022[t],sol[[1]]],
  (* Minus four *)
  Replace[P201[t],sol[[1]]],Replace[P210[t],sol[[1]]],Replace[P102[t],sol[[1]]],
  Replace[P111[t],sol[[1]]],Replace[P120[t],sol[[1]]],Replace[P003[t],sol[[1]]],
  Replace[P012[t],sol[[1]]],Replace[P021[t],sol[[1]]],
  (* Minus five *)
  Replace[P200[t],sol[[1]]],Replace[P101[t],sol[[1]]],Replace[P110[t],sol[[1]]],
  Replace[P011[t],sol[[1]]],Replace[P020[t],sol[[1]]],Replace[P002[t],sol[[1]]],
  (* Minus six *)
  Replace[P100[t],sol[[1]]],Replace[P010[t],sol[[1]]],Replace[P001[t],sol[[1]]],
  (* Minus seven *)
  Replace[P000[t],sol[[1]]]
  }/.{t->t1}
)

```

```

solveNitrogenRateEquations[en_,jxfunc_,neginf_,posinf_,maxstfr_,truth_]:=Module[{grndvec},
  grndvec=unitgrndvec[];
  solveNitrogenRateEquationsInitial[en,jxfunc,neginf,posinf,maxstfr,truth,grndvec]
]

```

```

solveNitrogenRateEquationsInitial[en_,jxfunc_,neginf_,posinf_,maxstfr_,truth_,grndvec_]:= (
  NDSolve[{req223[en,jxfunc      ],ieq223[neginf,grndvec[[ 1]]],
    req213[en,jxfunc      ],ieq213[neginf,grndvec[[ 2]]],
    req222[en,jxfunc      ],ieq222[neginf,grndvec[[ 3]]],
    req123[en,jxfunc,truth],ieq123[neginf,grndvec[[ 4]]],
    req212[en,jxfunc      ],ieq212[neginf,grndvec[[ 5]]],
    req203[en,jxfunc      ],ieq203[neginf,grndvec[[ 6]]],
    req221[en,jxfunc      ],ieq221[neginf,grndvec[[ 7]]],
    req113[en,jxfunc,truth],ieq113[neginf,grndvec[[ 8]]],
    req122[en,jxfunc,truth],ieq122[neginf,grndvec[[ 9]]],
    req023[en,jxfunc,truth],ieq023[neginf,grndvec[[10]]],
    req202[en,jxfunc      ],ieq202[neginf,grndvec[[11]]],
    req211[en,jxfunc      ],ieq211[neginf,grndvec[[12]]],
    req220[en,jxfunc      ],ieq220[neginf,grndvec[[13]]],
    req103[en,jxfunc,truth],ieq103[neginf,grndvec[[14]]],
    req112[en,jxfunc,truth],ieq112[neginf,grndvec[[15]]],
    req121[en,jxfunc,truth],ieq121[neginf,grndvec[[16]]],
    req013[en,jxfunc,truth],ieq013[neginf,grndvec[[17]]],
    req022[en,jxfunc,truth],ieq022[neginf,grndvec[[18]]],
    req201[en,jxfunc      ],ieq201[neginf,grndvec[[19]]],
    req210[en,jxfunc      ],ieq210[neginf,grndvec[[20]]],
    req102[en,jxfunc,truth],ieq102[neginf,grndvec[[21]]],
    req111[en,jxfunc,truth],ieq111[neginf,grndvec[[22]]],
    req120[en,jxfunc,truth],ieq120[neginf,grndvec[[23]]],
    req003[en,jxfunc,truth],ieq003[neginf,grndvec[[24]]],

```

```

req012[en,jxfunc,truth],ieq012[neginf,grndvec[[25]]],
req021[en,jxfunc,truth],ieq021[neginf,grndvec[[26]]],
req200[en,jxfunc],ieq200[neginf,grndvec[[27]]],
req101[en,jxfunc,truth],ieq101[neginf,grndvec[[28]]],
req110[en,jxfunc,truth],ieq110[neginf,grndvec[[29]]],
req011[en,jxfunc,truth],ieq011[neginf,grndvec[[30]]],
req020[en,jxfunc,truth],ieq020[neginf,grndvec[[31]]],
req002[en,jxfunc,truth],ieq002[neginf,grndvec[[32]]],
req100[en,jxfunc],ieq100[neginf,grndvec[[33]]],
req010[en,jxfunc,truth],ieq010[neginf,grndvec[[34]]],
req001[en,jxfunc,truth],ieq001[neginf,grndvec[[35]]],
req000[en,jxfunc],ieq000[neginf,grndvec[[36]]],
{P223[t],P213[t],P222[t],P123[t],P212[t],P203[t],P221[t],
P113[t],P122[t],P023[t],P202[t],P211[t],P220[t],P103[t],
P112[t],P121[t],P013[t],P022[t],P201[t],P210[t],P102[t],
P111[t],P120[t],P003[t],P012[t],P021[t],P200[t],P101[t],
P110[t],P011[t],P020[t],P002[t],P100[t],P010[t],P001[t],
P000[t]},
{t,neginf,posinf},MaxStepFraction->maxstfr]
)

```

```
solGround[sol_,t1_]:=Replace[P223[t],sol[[1]]]/.{t->t1}
```

```
solSingly[sol_,t1_]:= (Replace[P213[t],sol[[1]]]+Replace[P222[t],sol[[1]]] +
Replace[P123[t],sol[[1]]])/.{t->t1}
```

```
solDoubly[sol_,t1_]:= (Replace[P212[t],sol[[1]]]+Replace[P203[t],sol[[1]]] +
Replace[P221[t],sol[[1]]]+Replace[P113[t],sol[[1]]] +
Replace[P122[t],sol[[1]]]+Replace[P023[t],sol[[1]]])/.{t->t1}
```

```
solTriply[sol_,t1_]:= (Replace[P202[t],sol[[1]]]+Replace[P211[t],sol[[1]]] +
  Replace[P220[t],sol[[1]]]+Replace[P103[t],sol[[1]]] +
  Replace[P112[t],sol[[1]]]+Replace[P121[t],sol[[1]]] +
  Replace[P013[t],sol[[1]]]+Replace[P022[t],sol[[1]]])/.{t->t1}
```

```
solQuadruply[sol_,t1_]:= (Replace[P201[t],sol[[1]]]+Replace[P210[t],sol[[1]]] +
  Replace[P102[t],sol[[1]]]+Replace[P111[t],sol[[1]]] +
  Replace[P120[t],sol[[1]]]+Replace[P003[t],sol[[1]]] +
  Replace[P012[t],sol[[1]]]+Replace[P021[t],sol[[1]]])/.{t->t1}
```

```
solQuintuply[sol_,t1_]:= (Replace[P200[t],sol[[1]]]+Replace[P101[t],sol[[1]]] +
  Replace[P110[t],sol[[1]]]+Replace[P011[t],sol[[1]]] +
  Replace[P020[t],sol[[1]]]+Replace[P002[t],sol[[1]]])/.{t->t1}
```

```
solSextuply[sol_,t1_]:= (Replace[P100[t],sol[[1]]]+Replace[P010[t],sol[[1]]] +
  Replace[P001[t],sol[[1]]])/.{t->t1}
```

```
solSeptuply[sol_,t1_]:=Replace[P000[t],sol[[1]]]/.{t->t1}
```

Valence charge:

```

solValence[sol_,t1_]:=
(1*(Replace[P213[t],sol[[1]]]+Replace[P222[t],sol[[1]]] +
  Replace[P113[t],sol[[1]]]+Replace[P122[t],sol[[1]]] +
  Replace[P013[t],sol[[1]]]+Replace[P022[t],sol[[1]]]) +
2*(Replace[P212[t],sol[[1]]]+Replace[P203[t],sol[[1]]] +
  Replace[P221[t],sol[[1]]]+Replace[P103[t],sol[[1]]] +
  Replace[P112[t],sol[[1]]]+Replace[P121[t],sol[[1]]] +
  Replace[P003[t],sol[[1]]]+Replace[P012[t],sol[[1]]] +
  Replace[P021[t],sol[[1]]]) +
3*(Replace[P202[t],sol[[1]]]+Replace[P211[t],sol[[1]]] +
  Replace[P220[t],sol[[1]]]+Replace[P111[t],sol[[1]]] +
  Replace[P120[t],sol[[1]]]+Replace[P102[t],sol[[1]]] +
  Replace[P011[t],sol[[1]]]+Replace[P020[t],sol[[1]]] +
  Replace[P002[t],sol[[1]]]) +
4*(Replace[P201[t],sol[[1]]]+Replace[P210[t],sol[[1]]] +
  Replace[P101[t],sol[[1]]]+Replace[P110[t],sol[[1]]] +
  Replace[P010[t],sol[[1]]]+Replace[P001[t],sol[[1]]]) +
5*(Replace[P200[t],sol[[1]]]+Replace[P100[t],sol[[1]]] +
  Replace[P000[t],sol[[1]]]) /. {t->t1}

```

```

solProb[sol_,t1_,Pxxx_]:=Replace[Pxxx[t],sol[[1]]] /. {t->t1}

```

```

inclDCH[truth_]:=If[truth,1,0]

```

# One-photon absorption cross sections

## Interpolation functions

### No core holes

Zero

```
fsg123v223[en_]:=Module[{fxs},
fxs=Interpolation[{{412.76, 6.0393*^-19}, {448.51, 5.703*^-19}, {487.35, 4.6767*^-19},
{529.55, 3.812*^-19}, {575.41, 3.0982*^-19}, {625.24, 2.5117*^-19},
{679.39, 2.0313*^-19}, {738.22, 1.6389*^-19}, {802.16, 1.3189*^-19},
{871.62, 1.0585*^-19}, {947.11, 8.4708*^-20}, {1029.1, 6.7582*^-20},
{1118.3, 5.3756*^-20}, {1215.1, 4.264*^-20}, {1320.3, 3.3741*^-20},
{1434.7, 2.665*^-20}, {1558.9, 2.1021*^-20}, {1693.9, 1.6568*^-20},
{1840.6, 1.3049*^-20}, {2000., 1.0271*^-20}},Method->Spline];
fxs[en*HartreeToeV]*crossSectioncm2toAU*UnitStep[en*HartreeToeV-412.76]*
UnitStep[2000.-en*HartreeToeV]]
```

```
fsg213v223[en_]:=Module[{fxs},
fxs=Interpolation[{{25.283, 5.5561*^-19}, {31.822, 8.7022*^-19}, {40.053, 9.757*^-19},
{50.413, 9.2845*^-19}, {63.453, 7.9735*^-19}, {79.865, 6.3261*^-19},
{100.52, 4.7087*^-19}, {126.52, 3.3357*^-19}, {159.25, 2.2601*^-19},
{200.44, 1.468*^-19}, {252.28, 9.2196*^-20}, {317.53, 5.6045*^-20},
{399.66, 3.3202*^-20}, {503.03, 1.9201*^-20}, {633.15, 1.09*^-20},
{796.91, 6.0797*^-21}, {1003., 3.3379*^-21}, {1262.5, 1.806*^-21},
{1589., 9.632*^-22}, {2000., 5.0631*^-22}},Method->Spline];
fxs[en*HartreeToeV]*crossSectioncm2toAU*UnitStep[en*HartreeToeV-25.283]*
UnitStep[2000.-en*HartreeToeV]]
```



```
fsig222v223[en_]:=Module[{fxs},
fxs=Interpolation[{{13.048, 1.2435*^-17}, {17.005, 1.3946*^-17}, {22.161, 1.198*^-17},
{28.882, 8.8244*^-18}, {37.64, 5.8087*^-18}, {49.054, 3.4875*^-18},
{63.929, 1.933*^-18}, {83.315, 9.9721*^-19}, {108.58, 4.8196*^-19},
{141.51, 2.1978*^-19}, {184.42, 9.5375*^-20}, {240.34, 3.9827*^-20},
{313.22, 1.6205*^-20}, {408.2, 6.5031*^-21}, {531.99, 2.5971*^-21},
{693.31, 1.0363*^-21}, {903.55, 4.1247*^-22}, {1177.5, 1.6286*^-22},
{1534.6, 6.3316*^-23}, {2000., 2.4077*^-23}},Method->Spline];
fxs[en*HartreeToeV]*crossSectioncm2toAU*UnitStep[en*HartreeToeV-13.048]*
UnitStep[2000.-en*HartreeToeV]
```

Minus one

```
fsig113v213[en_]:=Module[{fxs},
fxs=Interpolation[{{432.26, 6.0441*^-19}, {468.55, 5.0911*^-19}, {507.9, 4.1768*^-19},
{550.54, 3.4145*^-19}, {596.77, 2.786*^-19}, {646.87, 2.2693*^-19},
{701.19, 1.8452*^-19}, {760.06, 1.4974*^-19}, {823.88, 1.2125*^-19},
{893.06, 9.7933*^-20}, {968.04, 7.8877*^-20}, {1049.3, 6.334*^-20},
{1137.4, 5.0714*^-20}, {1232.9, 4.0495*^-20}, {1336.5, 3.2262*^-20},
{1448.7, 2.5658*^-20}, {1570.3, 2.0383*^-20}, {1702.2, 1.6182*^-20},
{1845.1, 1.284*^-20}, {2000., 1.0182*^-20}},Method->Spline];
fxs[en*HartreeToeV]*crossSectioncm2toAU*UnitStep[en*HartreeToeV-432.26]*
UnitStep[2000.-en*HartreeToeV]
```

```
fsig203v213[en_]:=Module[{fxs},
fxs=Interpolation[{{41.9, 6.2014*^-19}, {51.354, 5.811*^-19}, {62.941, 4.9824*^-19},
{77.142, 4.0178*^-19}, {94.547, 3.0858*^-19}, {115.88, 2.2719*^-19},
{142.03, 1.6142*^-19}, {174.07, 1.1136*^-19}, {213.35, 7.4732*^-20},
{261.48, 4.8851*^-20}, {320.48, 3.1267*^-20}, {392.79, 1.962*^-20},
{481.41, 1.2099*^-20}, {590.03, 7.3559*^-21}, {723.16, 4.4112*^-21},
{886.33, 2.6141*^-21}, {1086.3, 1.5319*^-21}, {1331.4, 8.8725*^-22},
{1631.8, 5.0808*^-22}, {2000., 2.8765*^-22}},Method->Spline];
fxs[en*HartreeToeV]*crossSectioncm2toAU*UnitStep[en*HartreeToeV-41.9]*
UnitStep[2000.-en*HartreeToeV]
```

```
fsig212v213[en_]:=Module[{fxs},
fxs=Interpolation[{{27.462, 1.2418*^-17}, {34.415, 8.5269*^-18}, {43.128, 5.4421*^-18},
{54.048, 3.2943*^-18}, {67.732, 1.9104*^-18}, {84.881, 1.0668*^-18},
{106.37, 5.7532*^-19}, {133.3, 3.0032*^-19}, {167.05, 1.5207*^-19},
{209.35, 7.4939*^-20}, {262.35, 3.609*^-20}, {328.78, 1.7072*^-20},
{412.02, 7.9738*^-21}, {516.34, 3.6928*^-21}, {647.07, 1.7001*^-21},
{810.9, 7.7851*^-22}, {1016.2, 3.5397*^-22}, {1273.5, 1.5934*^-22},
{1595.9, 7.0763*^-23}, {2000., 3.0904*^-23}},Method->Spline];
fxs[en*HartreeToeV]*crossSectioncm2toAU*UnitStep[en*HartreeToeV-27.462]*
UnitStep[2000.-en*HartreeToeV]
```

```

fsig122v222[en_]:=Module[{fxs},
fxs=Interpolation[{{433.45, 5.8957*^-19}, {469.78, 5.0102*^-19}, {509.15, 4.1295*^-19},
{551.82, 3.386*^-19}, {598.06, 2.7681*^-19}, {648.19, 2.2572*^-19},
{702.51, 1.8363*^-19}, {761.38, 1.4903*^-19}, {825.19, 1.2067*^-19},
{894.35, 9.7457*^-20}, {969.31, 7.8505*^-20}, {1050.5, 6.307*^-20},
{1138.6, 5.0538*^-20}, {1234., 4.0398*^-20}, {1337.4, 3.2224*^-20},
{1449.5, 2.566*^-20}, {1571., 2.0407*^-20}, {1702.7, 1.6213*^-20},
{1845.3, 1.2871*^-20}, {2000., 1.021*^-20}},Method->Spline];
fxs[en*HartreeToeV]*crossSectioncm2toAU*UnitStep[en*HartreeToeV-433.45]*
UnitStep[2000.-en*HartreeToeV]]

```

```

fsig212v222[en_]:=Module[{fxs},
fxs=Interpolation[{{39.697, 1.3573*^-18}, {48.792, 1.2169*^-18}, {59.971, 1.0163*^-18},
{73.712, 8.0616*^-19}, {90.601, 6.1336*^-19}, {111.36, 4.5005*^-19},
{136.87, 3.1997*^-19}, {168.23, 2.2128*^-19}, {206.78, 1.4903*^-19},
{254.15, 9.7865*^-20}, {312.39, 6.2855*^-20}, {383.96, 3.9527*^-20},
{471.93, 2.4395*^-20}, {580.06, 1.4809*^-20}, {712.96, 8.8561*^-21},
{876.31, 5.2245*^-21}, {1077.1, 3.0444*^-21}, {1323.9, 1.7523*^-21},
{1627.2, 9.9655*^-22}, {2000., 5.6005*^-22}},Method->Spline];
fxs[en*HartreeToeV]*crossSectioncm2toAU*UnitStep[en*HartreeToeV-39.697]*
UnitStep[2000.-en*HartreeToeV]]

```

```
fsig221v222[en_]:=Module[{fxs},
fxs=Interpolation[{{28.956, 8.4307*^-18}, {36.186, 5.8344*^-18}, {45.222, 3.7219*^-18},
{56.514, 2.241*^-18}, {70.625, 1.2883*^-18}, {88.26, 7.1141*^-19},
{110.3, 3.7884*^-19}, {137.84, 1.9511*^-19}, {172.26, 9.7467*^-20},
{215.27, 4.7426*^-20}, {269.02, 2.2596*^-20}, {336.2, 1.0605*^-20},
{420.14, 4.9336*^-21}, {525.05, 2.2861*^-21}, {656.15, 1.0579*^-21},
{819.99, 4.8893*^-22}, {1024.7, 2.2507*^-22}, {1280.6, 1.0279*^-22},
{1600.4, 4.635*^-23}, {2000., 2.0558*^-23}},Method->Spline];
fxs[en*HartreeToeV]*crossSectioncm2toAU*UnitStep[en*HartreeToeV-28.956]*
UnitStep[2000.-en*HartreeToeV]
```

Minus two

```
fsig103v203[en_]:=Module[{fxs},
fxs=Interpolation[{{454.96, 5.4328*^-19}, {491.83, 4.4926*^-19}, {531.7, 3.6922*^-19},
{574.79, 3.0297*^-19}, {621.37, 2.4837*^-19}, {671.74, 2.0339*^-19},
{726.18, 1.6635*^-19}, {785.03, 1.3585*^-19}, {848.66, 1.1071*^-19},
{917.44, 9.002*^-20}, {991.8, 7.2999*^-20}, {1072.2, 5.903*^-20},
{1159.1, 4.76*^-20}, {1253., 3.8286*^-20}, {1354.6, 3.073*^-20},
{1464.4, 2.4628*^-20}, {1583.1, 1.9718*^-20}, {1711.4, 1.5778*^-20},
{1850.1, 1.2621*^-20}, {2000., 1.009*^-20}},Method->Spline];
fxs[en*HartreeToeV]*crossSectioncm2toAU*UnitStep[en*HartreeToeV-454.96]*
UnitStep[2000.-en*HartreeToeV]
```

```
fsig202v203[en_]:=Module[{fxs},
fxs=Interpolation[{{44.025, 6.3665*^-18}, {53.818, 3.9176*^-18}, {65.789, 2.3548*^-18},
{80.424, 1.3868*^-18}, {98.313, 8.015*^-19}, {120.18, 4.5496*^-19},
{146.92, 2.5375*^-19}, {179.6, 1.3911*^-19}, {219.54, 7.5004*^-20},
{268.38, 3.9815*^-20}, {328.08, 2.0839*^-20}, {401.06, 1.0773*^-20},
{490.27, 5.5099*^-21}, {599.33, 2.7923*^-21}, {732.64, 1.4032*^-21},
{895.61, 6.9929*^-22}, {1094.8, 3.4533*^-22}, {1338.4, 1.6878*^-22},
{1636.1, 8.1508*^-23}, {2000., 3.8835*^-23}},Method->Spline];
fxs[en*HartreeToeV]*crossSectioncm2toAU*UnitStep[en*HartreeToeV-44.025]*
UnitStep[2000.-en*HartreeToeV]]
```

```
fsig112v212[en_]:=Module[{fxs},
fxs=Interpolation[{{456.68, 5.3175*^-19}, {493.6, 4.425*^-19}, {533.49, 3.651*^-19},
{576.62, 3.0039*^-19}, {623.23, 2.4666*^-19}, {673.61, 2.0219*^-19},
{728.06, 1.6544*^-19}, {786.91, 1.3511*^-19}, {850.52, 1.1011*^-19},
{919.27, 8.9538*^-20}, {993.57, 7.2631*^-20}, {1073.9, 5.8769*^-20},
{1160.7, 4.7437*^-20}, {1254.5, 3.8203*^-20}, {1355.9, 3.0706*^-20},
{1465.5, 2.4642*^-20}, {1584., 1.9752*^-20}, {1712., 1.582*^-20},
{1850.4, 1.2662*^-20}, {2000., 1.0127*^-20}},Method->Spline];
fxs[en*HartreeToeV]*crossSectioncm2toAU*UnitStep[en*HartreeToeV-456.68]*
UnitStep[2000.-en*HartreeToeV]]
```

```
fsig202v212[en_] := Module[{fxs},
fxs = Interpolation[{{58.463, 6.5829*^-19}, {70.409, 5.3268*^-19}, {84.795, 4.152*^-19},
{102.12, 3.1386*^-19}, {122.99, 2.3096*^-19}, {148.12, 1.6591*^-19},
{178.38, 1.1666*^-19}, {214.83, 8.0483*^-20}, {258.73, 5.4534*^-20},
{311.59, 3.6322*^-20}, {375.26, 2.3833*^-20}, {451.93, 1.5424*^-20},
{544.27, 9.8522*^-21}, {655.48, 6.2242*^-21}, {789.42, 3.8889*^-21},
{950.72, 2.4064*^-21}, {1145., 1.474*^-21}, {1378.9, 8.9457*^-22},
{1660.7, 5.3756*^-22}, {2000., 3.1984*^-22}}, Method -> Spline];
fxs[en*HartreeToeV]*crossSectioncm2toAU*UnitStep[en*HartreeToeV-58.463]*
UnitStep[2000.-en*HartreeToeV]
```

```
fsig121v221[en_] := Module[{fxs},
fxs = Interpolation[{{459.05, 5.1934*^-19}, {496.02, 4.3478*^-19}, {535.97, 3.6014*^-19},
{579.14, 2.9711*^-19}, {625.78, 2.4441*^-19}, {676.18, 2.0055*^-19},
{730.64, 1.6419*^-19}, {789.48, 1.3411*^-19}, {853.07, 1.093*^-19},
{921.77, 8.8891*^-20}, {996.01, 7.2131*^-20}, {1076.2, 5.8405*^-20},
{1162.9, 4.7193*^-20}, {1256.6, 3.8059*^-20}, {1357.8, 3.0639*^-20},
{1467.1, 2.4628*^-20}, {1585.3, 1.977*^-20}, {1713., 1.5853*^-20},
{1850.9, 1.27*^-20}, {2000., 1.0164*^-20}}, Method -> Spline];
fxs[en*HartreeToeV]*crossSectioncm2toAU*UnitStep[en*HartreeToeV-459.05]*
UnitStep[2000.-en*HartreeToeV]
```

```
fsig211v221[en_]:=Module[{fxs},
fxs=Interpolation[{{56.632, 1.3589*^-18}, {68.318, 1.0762*^-18}, {82.415, 8.2692*^-19},
{99.421, 6.194*^-19}, {119.94, 4.5363*^-19}, {144.68, 3.2548*^-19},
{174.54, 2.2917*^-19}, {210.56, 1.5854*^-19}, {254., 1.0781*^-19},
{306.41, 7.2101*^-20}, {369.64, 4.7475*^-20}, {445.92, 3.0802*^-20},
{537.93, 1.9706*^-20}, {648.93, 1.2449*^-20}, {782.83, 7.7705*^-21},
{944.37, 4.7975*^-21}, {1139.2, 2.9304*^-21}, {1374.3, 1.772*^-21},
{1657.9, 1.0607*^-21}, {2000., 6.2859*^-22}},Method->Spline];
fxs[en*HartreeToeV]*crossSectioncm2toAU*UnitStep[en*HartreeToeV-56.632]*
UnitStep[2000.-en*HartreeToeV]
```

```
fsig220v221[en_]:=Module[{fxs},
fxs=Interpolation[{{48.079, 2.2922*^-18}, {58.502, 1.4053*^-18}, {71.184, 8.3587*^-19},
{86.616, 4.8456*^-19}, {105.39, 2.7446*^-19}, {128.24, 1.5217*^-19},
{156.04, 8.2732*^-20}, {189.87, 4.4188*^-20}, {231.03, 2.3229*^-20},
{281.12, 1.2055*^-20}, {342.06, 6.1978*^-21}, {416.21, 3.166*^-21},
{506.44, 1.6124*^-21}, {616.23, 8.2*^-22}, {749.82, 4.1672*^-22},
{912.37, 2.1135*^-22}, {1110.2, 1.0676*^-22}, {1350.8, 5.3524*^-23},
{1643.7, 2.6551*^-23}, {2000., 1.2999*^-23}},Method->Spline];
fxs[en*HartreeToeV]*crossSectioncm2toAU*UnitStep[en*HartreeToeV-48.079]*
UnitStep[2000.-en*HartreeToeV]
```

```
fsig211v212[en_]:=Module[{fxs},
fxs=Interpolation[{{45.891, 4.422*^-18}, {55.977, 2.7177*^-18}, {68.279, 1.6257*^-18},
{83.285, 9.5011*^-19}, {101.59, 5.4365*^-19}, {123.91, 3.0495*^-19},
{151.15, 1.6788*^-19}, {184.37, 9.0804*^-20}, {224.88, 4.8317*^-20},
{274.31, 2.5344*^-20}, {334.59, 1.3137*^-20}, {408.13, 6.7459*^-21},
{497.82, 3.4404*^-21}, {607.23, 1.7454*^-21}, {740.69, 8.8153*^-22},
{903.47, 4.4292*^-22}, {1102., 2.211*^-22}, {1344.2, 1.094*^-22},
{1639.6, 5.352*^-23}, {2000., 2.5836*^-23}},Method->Spline];
fxs[en*HartreeToeV]*crossSectioncm2toAU*UnitStep[en*HartreeToeV-45.891]*
UnitStep[2000.-en*HartreeToeV]
```

Minus three

```
fsig102v202[en_]:=Module[{fxs},
fxs=Interpolation[{{482.87, 4.6655*^-19}, {520.37, 3.87*^-19}, {560.79, 3.2021*^-19},
{604.34, 2.6459*^-19}, {651.28, 2.1839*^-19}, {701.86, 1.8004*^-19},
{756.37, 1.4822*^-19}, {815.12, 1.2184*^-19}, {878.42, 9.9975*^-20},
{946.65, 8.1869*^-20}, {1020.2, 6.6896*^-20}, {1099.4, 5.4535*^-20},
{1184.8, 4.4359*^-20}, {1276.8, 3.6008*^-20}, {1376., 2.9177*^-20},
{1482.8, 2.3609*^-20}, {1598., 1.9084*^-20}, {1722.1, 1.5414*^-20},
{1855.9, 1.2443*^-20}, {2000., 1.004*^-20}},Method->Spline];
fxs[en*HartreeToeV]*crossSectioncm2toAU*UnitStep[en*HartreeToeV-482.87]*
UnitStep[2000.-en*HartreeToeV]
```



```
fsig201v202[en_] := Module[{fxs},
fxs = Interpolation[{{64.809, 2.1825*^-18}, {77.629, 1.324*^-18}, {92.985, 7.9405*^-19},
{111.38, 4.7107*^-19}, {133.41, 2.7655*^-19}, {159.8, 1.607*^-19},
{191.41, 9.2448*^-20}, {229.28, 5.2662*^-20}, {274.63, 2.9714*^-20},
{328.96, 1.6614*^-20}, {394.03, 9.2098*^-21}, {471.97, 5.0648*^-21},
{565.33, 2.7647*^-21}, {677.17, 1.4985*^-21}, {811.12, 8.0648*^-22},
{971.57, 4.3084*^-22}, {1163.8, 2.2831*^-22}, {1394., 1.199*^-22},
{1669.7, 6.2326*^-23}, {2000., 3.2039*^-23}}, Method -> Spline];
fxs[en*HartreeToeV]*crossSectioncm2toAU*UnitStep[en*HartreeToeV-64.809]*
UnitStep[2000.-en*HartreeToeV]]
```

```
fsig111v211[en_] := Module[{fxs},
fxs = Interpolation[{{485.76, 4.5669*^-19}, {523.32, 3.8065*^-19}, {563.79, 3.1602*^-19},
{607.39, 2.6175*^-19}, {654.35, 2.1638*^-19}, {704.95, 1.7854*^-19},
{759.47, 1.4706*^-19}, {818.19, 1.2091*^-19}, {881.46, 9.9226*^-20},
{949.62, 8.1275*^-20}, {1023.1, 6.6444*^-20}, {1102.2, 5.4212*^-20},
{1187.4, 4.4149*^-20}, {1279.2, 3.5891*^-20}, {1378.1, 2.9131*^-20},
{1484.7, 2.3612*^-20}, {1599.5, 1.9116*^-20}, {1723.2, 1.546*^-20},
{1856.4, 1.2492*^-20}, {2000., 1.0086*^-20}}, Method -> Spline];
fxs[en*HartreeToeV]*crossSectioncm2toAU*UnitStep[en*HartreeToeV-485.76]*
UnitStep[2000.-en*HartreeToeV]]
```

```

fsig201v211[en_]:=Module[{fxs},
fxs=Interpolation[{{77.381, 5.6546*^-19}, {91.827, 4.3389*^-19}, {108.97, 3.2614*^-19},
{129.31, 2.4072*^-19}, {153.45, 1.7475*^-19}, {182.1, 1.2495*^-19},
{216.1, 8.8102*^-20}, {256.44, 6.1326*^-20}, {304.32, 4.2168*^-20},
{361.13, 2.8657*^-20}, {428.55, 1.9266*^-20}, {508.55, 1.2822*^-20},
{603.5, 8.4497*^-21}, {716.16, 5.5181*^-21}, {849.86, 3.5725*^-21},
{1008.5, 2.2929*^-21}, {1196.8, 1.4597*^-21}, {1420.2, 9.2137*^-22},
{1685.4, 5.768*^-22}, {2000., 3.5805*^-22}},Method->Spline];
fxs[en*HartreeToeV]*crossSectioncm2toAU*UnitStep[en*HartreeToeV-77.381]*
UnitStep[2000.-en*HartreeToeV]]

```

```

fsig210v211[en_]:=Module[{fxs},
fxs=Interpolation[{{67.373, 1.139*^-18}, {80.536, 6.8752*^-19}, {96.27, 4.0941*^-19},
{115.08, 2.4071*^-19}, {137.56, 1.3981*^-19}, {164.44, 8.028*^-20},
{196.56, 4.5612*^-20}, {234.96, 2.5665*^-20}, {280.87, 1.4315*^-20},
{335.74, 7.9241*^-21}, {401.34, 4.3604*^-21}, {479.75, 2.3875*^-21},
{573.47, 1.3019*^-21}, {685.51, 7.0754*^-22}, {819.44, 3.8298*^-22},
{979.54, 2.0636*^-22}, {1170.9, 1.105*^-22}, {1399.7, 5.8722*^-23},
{1673.1, 3.0903*^-23}, {2000., 1.6085*^-23}},Method->Spline];
fxs[en*HartreeToeV]*crossSectioncm2toAU*UnitStep[en*HartreeToeV-67.373]*
UnitStep[2000.-en*HartreeToeV]]

```

```
fsig120v220[en_]:=Module[{fxs},
fxs=Interpolation[{{489.31, 4.4619*^-19}, {526.95, 3.7363*^-19}, {567.48, 3.1125*^-19},
{611.12, 2.5843*^-19}, {658.13, 2.1399*^-19}, {708.75, 1.7676*^-19},
{763.26, 1.4567*^-19}, {821.97, 1.198*^-19}, {885.19, 9.8334*^-20},
{953.27, 8.0567*^-20}, {1026.6, 6.5898*^-20}, {1105.6, 5.3813*^-20},
{1190.6, 4.3878*^-20}, {1282.2, 3.5727*^-20}, {1380.8, 2.9051*^-20},
{1487., 2.3592*^-20}, {1601.3, 1.9135*^-20}, {1724.5, 1.55*^-20},
{1857.2, 1.2541*^-20}, {2000., 1.0136*^-20}},Method->Spline];
fxs[en*HartreeToeV]*crossSectioncm2toAU*UnitStep[en*HartreeToeV-489.31]*
UnitStep[2000.-en*HartreeToeV]
```

```
fsig210v220[en_]:=Module[{fxs},
fxs=Interpolation[{{75.926, 1.1346*^-18}, {90.191, 8.5996*^-19}, {107.14, 6.4105*^-19},
{127.26, 4.7077*^-19}, {151.17, 3.4103*^-19}, {179.57, 2.4389*^-19},
{213.31, 1.723*^-19}, {253.39, 1.2029*^-19}, {300.99, 8.3006*^-20},
{357.54, 5.6628*^-20}, {424.71, 3.8202*^-20}, {504.51, 2.5493*^-20},
{599.29, 1.6833*^-20}, {711.88, 1.1003*^-20}, {845.62, 7.1229*^-21},
{1004.5, 4.5684*^-21}, {1193.2, 2.9038*^-21}, {1417.4, 1.8297*^-21},
{1683.7, 1.1429*^-21}, {2000., 7.0785*^-22}},Method->Spline];
fxs[en*HartreeToeV]*crossSectioncm2toAU*UnitStep[en*HartreeToeV-75.926]*
UnitStep[2000.-en*HartreeToeV]
```

Minus four

```
fsig101v201[en_]:=Module[{fxs},
fxs=Interpolation[{{515.28, 3.9624*^-19}, {553.4, 3.3071*^-19}, {594.35, 2.756*^-19},
{638.32, 2.2936*^-19}, {685.55, 1.9064*^-19}, {736.27, 1.5825*^-19},
{790.75, 1.3119*^-19}, {849.26, 1.0859*^-19}, {912.09, 8.9752*^-20},
{979.57, 7.4061*^-20}, {1052., 6.1011*^-20}, {1129.9, 5.0174*^-20},
{1213.5, 4.1194*^-20}, {1303.3, 3.3769*^-20}, {1399.7, 2.7642*^-20},
{1503.3, 2.26*^-20}, {1614.5, 1.8458*^-20}, {1733.9, 1.5061*^-20},
{1862.2, 1.228*^-20}, {2000., 1.0005*^-20}},Method->Spline];
fxs[en*HartreeToeV]*crossSectioncm2toAU*UnitStep[en*HartreeToeV-515.28]*
UnitStep[2000.-en*HartreeToeV]
```

```
fsig200v201[en_]:=Module[{fxs},
fxs=Interpolation[{{88.319, 5.9953*^-19}, {104.08, 3.6769*^-19}, {122.65, 2.2394*^-19},
{144.54, 1.3549*^-19}, {170.34, 8.1461*^-20}, {200.74, 4.8681*^-20},
{236.56, 2.8924*^-20}, {278.78, 1.7091*^-20}, {328.53, 1.0045*^-20},
{387.15, 5.8726*^-21}, {456.25, 3.4158*^-21}, {537.67, 1.9765*^-21},
{633.62, 1.1376*^-21}, {746.69, 6.511*^-22}, {879.95, 3.7042*^-22},
{1037., 2.0935*^-22}, {1222., 1.1746*^-22}, {1440.1, 6.5381*^-23},
{1697.1, 3.6071*^-23}, {2000., 1.9712*^-23}},Method->Spline];
fxs[en*HartreeToeV]*crossSectioncm2toAU*UnitStep[en*HartreeToeV-88.319]*
UnitStep[2000.-en*HartreeToeV]
```

```
fsig110v210[en_]:=Module[{fxs},
fxs=Interpolation[{{519.34, 3.8784*^-19}, {557.53, 3.2499*^-19}, {598.54, 2.7163*^-19},
{642.56, 2.2655*^-19}, {689.81, 1.8858*^-19}, {740.54, 1.5669*^-19},
{795.01, 1.2996*^-19}, {853.48, 1.0761*^-19}, {916.24, 8.8969*^-20},
{983.63, 7.3444*^-20}, {1056., 6.0542*^-20}, {1133.6, 4.9837*^-20},
{1217., 4.0972*^-20}, {1306.5, 3.3641*^-20}, {1402.6, 2.759*^-20},
{1505.7, 2.2601*^-20}, {1616.5, 1.8493*^-20}, {1735.4, 1.5115*^-20},
{1863., 1.2341*^-20}, {2000., 1.0066*^-20}},Method->Spline];
fxs[en*HartreeToeV]*crossSectioncm2toAU*UnitStep[en*HartreeToeV-519.34]*
UnitStep[2000.-en*HartreeToeV]]
```

```
fsig200v210[en_]:=Module[{fxs},
fxs=Interpolation[{{98.327, 4.5458*^-19}, {115.22, 3.4185*^-19}, {135.02, 2.5375*^-19},
{158.22, 1.8614*^-19}, {185.4, 1.3505*^-19}, {217.26, 9.6993*^-20},
{254.59, 6.8999*^-20}, {298.33, 4.8644*^-20}, {349.59, 3.4002*^-20},
{409.66, 2.3573*^-20}, {480.04, 1.6214*^-20}, {562.53, 1.1068*^-20},
{659.18, 7.4983*^-21}, {772.44, 5.0429*^-21}, {905.16, 3.3669*^-21},
{1060.7, 2.2316*^-21}, {1242.9, 1.4684*^-21}, {1456.5, 9.5922*^-22},
{1706.7, 6.2201*^-22}, {2000., 4.0037*^-22}},Method->Spline];
fxs[en*HartreeToeV]*crossSectioncm2toAU*UnitStep[en*HartreeToeV-98.327]*
UnitStep[2000.-en*HartreeToeV]]
```

Minus five

```
fsig100v200[en_] := Module[{fxs},
fxs = Interpolation[{{552.08, 3.3432*^-19}, {590.78, 2.8106*^-19}, {632.19, 2.3596*^-19},
{676.5, 1.9782*^-19}, {723.92, 1.6562*^-19}, {774.67, 1.3848*^-19},
{828.97, 1.1563*^-19}, {887.07, 9.6421*^-20}, {949.25, 8.0307*^-20},
{1015.8, 6.6805*^-20}, {1087., 5.5508*^-20}, {1163.2, 4.6069*^-20},
{1244.7, 3.8193*^-20}, {1332., 3.163*^-20}, {1425.3, 2.6168*^-20},
{1525.2, 2.1628*^-20}, {1632.2, 1.7857*^-20}, {1746.6, 1.4728*^-20},
{1869., 1.2137*^-20}, {2000., 9.992*^-21}}, Method -> Spline];
fxs[en*HartreeToeV]*crossSectioncm2toAU*UnitStep[en*HartreeToeV-552.08]*
UnitStep[2000.-en*HartreeToeV]
```

## Single core holes

Minus one

```
fsig023v123[en_] := Module[{fxs},
fxs = Interpolation[{{502.57, 2.5563*^-19}, {540.46, 2.2232*^-19}, {581.22, 1.8579*^-19},
{625.04, 1.5427*^-19}, {672.17, 1.2776*^-19}, {722.85, 1.056*^-19},
{777.35, 8.7125*^-20}, {835.96, 7.1763*^-20}, {899., 5.9009*^-20},
{966.78, 4.8433*^-20}, {1039.7, 3.9673*^-20}, {1118.1, 3.2431*^-20},
{1202.4, 2.6452*^-20}, {1293., 2.1529*^-20}, {1390.5, 1.7486*^-20},
{1495.4, 1.4176*^-20}, {1608.1, 1.1474*^-20}, {1729.4, 9.2755*^-21},
{1859.8, 7.4915*^-21}, {2000., 6.047*^-21}}, Method -> Spline];
fxs[en*HartreeToeV]*crossSectioncm2toAU*UnitStep[en*HartreeToeV-502.57]*
UnitStep[2000.-en*HartreeToeV]
```

```
fsig113v123[en_]:=Module[{fxs},
fxs=Interpolation[{{44.8, 1.6135*^-18}, {54.715, 1.3884*^-18}, {66.825, 1.132*^-18},
{81.614, 8.8591*^-19}, {99.677, 6.6997*^-19}, {121.74, 4.9118*^-19},
{148.68, 3.5009*^-19}, {181.59, 2.4329*^-19}, {221.77, 1.6503*^-19},
{270.86, 1.0927*^-19}, {330.8, 7.0764*^-20}, {404.02, 4.4908*^-20},
{493.43, 2.7945*^-20}, {602.64, 1.7107*^-20}, {736.01, 1.0308*^-20},
{898.9, 6.1323*^-21}, {1097.8, 3.6027*^-21}, {1340.8, 2.0938*^-21},
{1637.6, 1.2045*^-21}, {2000., 6.8588*^-22}},Method->Spline];
fxs[en*HartreeToeV]*crossSectioncm2toAU*UnitStep[en*HartreeToeV-44.8]*
UnitStep[2000.-en*HartreeToeV]
```

```
fsig122v123[en_]:=Module[{fxs},
fxs=Interpolation[{{33.757, 1.0194*^-17}, {41.847, 7.8327*^-18}, {51.875, 5.4053*^-18},
{64.307, 3.4732*^-18}, {79.718, 2.1141*^-18}, {98.822, 1.2301*^-18},
{122.5, 6.879*^-19}, {151.86, 3.7113*^-19}, {188.26, 1.9371*^-19},
{233.37, 9.8116*^-20}, {289.3, 4.8433*^-20}, {358.63, 2.3404*^-20},
{444.57, 1.1131*^-20}, {551.11, 5.2358*^-21}, {683.19, 2.4456*^-21},
{846.91, 1.1366*^-21}, {1049.9, 5.2575*^-22}, {1301.5, 2.4172*^-22},
{1613.4, 1.1016*^-22}, {2000., 4.9642*^-23}},Method->Spline];
fxs[en*HartreeToeV]*crossSectioncm2toAU*UnitStep[en*HartreeToeV-33.757]*
UnitStep[2000.-en*HartreeToeV]
```

Minus two

```
fsig013v113[en_]:=Module[{fxs},
fxs=Interpolation[{{526.57, 2.3485*^-19}, {564.88, 1.9821*^-19}, {605.99, 1.6549*^-19},
{650.08, 1.3778*^-19}, {697.38, 1.1456*^-19}, {748.13, 9.515*^-20},
{802.56, 7.8945*^-20}, {860.96, 6.5422*^-20}, {923.61, 5.414*^-20},
{990.81, 4.4732*^-20}, {1062.9, 3.689*^-20}, {1140.2, 3.0361*^-20},
{1223.2, 2.4932*^-20}, {1312.2, 2.043*^-20}, {1407.7, 1.6706*^-20},
{1510.1, 1.3636*^-20}, {1620., 1.1114*^-20}, {1737.9, 9.0489*^-21},
{1864.3, 7.3617*^-21}, {2000., 5.9871*^-21}},Method->Spline];
fxs[en*HartreeToeV]*crossSectioncm2toAU*UnitStep[en*HartreeToeV-526.57]*
UnitStep[2000.-en*HartreeToeV]
```

```
fsig103v113[en_]:=Module[{fxs},
fxs=Interpolation[{{64.597, 7.2055*^-19}, {77.389, 5.7626*^-19}, {92.713, 4.4697*^-19},
{111.07, 3.3783*^-19}, {133.07, 2.4942*^-19}, {159.42, 1.8017*^-19},
{190.98, 1.2755*^-19}, {228.8, 8.8666*^-20}, {274.11, 6.0576*^-20},
{328.39, 4.0679*^-20}, {393.42, 2.6889*^-20}, {471.32, 1.7528*^-20},
{564.65, 1.127*^-20}, {676.47, 7.1607*^-21}, {810.42, 4.5015*^-21},
{970.9, 2.8009*^-21}, {1163.2, 1.7276*^-21}, {1393.5, 1.0561*^-21},
{1669.4, 6.4025*^-22}, {2000., 3.8504*^-22}},Method->Spline];
fxs[en*HartreeToeV]*crossSectioncm2toAU*UnitStep[en*HartreeToeV-64.597]*
UnitStep[2000.-en*HartreeToeV]
```



```

fsig112v113[en_]:=Module[{fxs},
fxs=Interpolation[{{51.883, 6.4057*^-18}, {62.878, 4.1798*^-18}, {76.203, 2.6332*^-18},
{92.352, 1.6122*^-18}, {111.92, 9.6272*^-19}, {135.64, 5.6182*^-19},
{164.39, 3.2084*^-19}, {199.22, 1.7949*^-19}, {241.44, 9.8456*^-20},
{292.61, 5.3027*^-20}, {354.62, 2.8098*^-20}, {429.77, 1.468*^-20},
{520.85, 7.5793*^-21}, {631.23, 3.8769*^-21}, {765., 1.9676*^-21},
{927.12, 9.9203*^-22}, {1123.6, 4.968*^-22}, {1361.7, 2.4702*^-22},
{1650.3, 1.218*^-22}, {2000., 5.948*^-23}},Method->Spline];
fxs[en*HartreeToeV]*crossSectioncm2toAU*UnitStep[en*HartreeToeV-51.883]*
UnitStep[2000.-en*HartreeToeV]]

```

```

fsig022v122[en_]:=Module[{fxs},
fxs=Interpolation[{{529.83, 2.2886*^-19}, {568.2, 1.9455*^-19}, {609.34, 1.6325*^-19},
{653.47, 1.3641*^-19}, {700.79, 1.137*^-19}, {751.54, 9.4578*^-20},
{805.96, 7.8529*^-20}, {864.32, 6.5093*^-20}, {926.91, 5.3864*^-20},
{994.04, 4.4497*^-20}, {1066., 3.6696*^-20}, {1143.2, 3.021*^-20},
{1226., 2.4825*^-20}, {1314.8, 2.0365*^-20}, {1410., 1.6679*^-20},
{1512.1, 1.3638*^-20}, {1621.6, 1.1137*^-20}, {1739., 9.0831*^-21},
{1864.9, 7.4008*^-21}, {2000., 6.0256*^-21}},Method->Spline];
fxs[en*HartreeToeV]*crossSectioncm2toAU*UnitStep[en*HartreeToeV-529.83]*
UnitStep[2000.-en*HartreeToeV]]

```

```

fsig112v122[en_] := Module[{fxs},
fxs = Interpolation[{{62.926, 1.4789*^-18}, {75.491, 1.1627*^-18}, {90.564, 8.9133*^-19},
{108.65, 6.6847*^-19}, {130.34, 4.9136*^-19}, {156.37, 3.5438*^-19},
{187.59, 2.5105*^-19}, {225.05, 1.7486*^-19}, {269.98, 1.1978*^-19},
{323.89, 8.0698*^-20}, {388.56, 5.3512*^-20}, {466.15, 3.4965*^-20},
{559.23, 2.2519*^-20}, {670.89, 1.4317*^-20}, {804.85, 8.9956*^-21},
{965.56, 5.5902*^-21}, {1158.4, 3.4401*^-21}, {1389.6, 2.0974*^-21},
{1667.1, 1.2675*^-21}, {2000., 7.5964*^-22}}, Method -> Spline];
fxs[en*HartreeToeV]*crossSectioncm2toAU*UnitStep[en*HartreeToeV-62.926]*
UnitStep[2000.-en*HartreeToeV]

```

```

fsig121v122[en_] := Module[{fxs},
fxs = Interpolation[{{54.552, 4.3848*^-18}, {65.938, 2.8573*^-18}, {79.701, 1.7915*^-18},
{96.337, 1.0892*^-18}, {116.44, 6.4478*^-19}, {140.75, 3.7254*^-19},
{170.13, 2.1048*^-19}, {205.64, 1.1649*^-19}, {248.56, 6.3241*^-20},
{300.44, 3.3743*^-20}, {363.15, 1.7747*^-20}, {438.95, 9.2268*^-21},
{530.57, 4.7545*^-21}, {641.31, 2.4361*^-21}, {775.16, 1.2426*^-21},
{936.96, 6.318*^-22}, {1132.5, 3.1988*^-22}, {1368.9, 1.6116*^-22},
{1654.6, 8.0597*^-23}, {2000., 3.9942*^-23}}, Method -> Spline];
fxs[en*HartreeToeV]*crossSectioncm2toAU*UnitStep[en*HartreeToeV-54.552]*
UnitStep[2000.-en*HartreeToeV]

```

Minus three

```
fsig003v103[en_]:=Module[{fxs},
fxs=Interpolation[{{553.53, 2.0834*^-19}, {592.25, 1.7476*^-19}, {633.67, 1.4619*^-19},
{678., 1.2219*^-19}, {725.42, 1.0209*^-19}, {776.16, 8.5267*^-20},
{830.46, 7.1177*^-20}, {888.54, 5.9366*^-20}, {950.7, 4.9459*^-20},
{1017.2, 4.1145*^-20}, {1088.3, 3.4169*^-20}, {1164.5, 2.8318*^-20},
{1245.9, 2.3419*^-20}, {1333.1, 1.9326*^-20}, {1426.3, 1.5918*^-20},
{1526.1, 1.3088*^-20}, {1632.8, 1.0747*^-20}, {1747., 8.8162*^-21},
{1869.3, 7.2287*^-21}, {2000., 5.926*^-21}},Method->Spline];
fxs[en*HartreeToeV]*crossSectioncm2toAU*UnitStep[en*HartreeToeV-553.53]*
UnitStep[2000.-en*HartreeToeV]
```

```
fsig102v103[en_]:=Module[{fxs},
fxs=Interpolation[{{71.933, 3.449*^-18}, {85.691, 2.1832*^-18}, {102.08, 1.3613*^-18},
{121.6, 8.3704*^-19}, {144.86, 5.0786*^-19}, {172.57, 3.0413*^-19},
{205.57, 1.7978*^-19}, {244.89, 1.0491*^-19}, {291.72, 6.0441*^-20},
{347.52, 3.4389*^-20}, {413.98, 1.9333*^-20}, {493.16, 1.0747*^-20},
{587.48, 5.912*^-21}, {699.84, 3.2214*^-21}, {833.69, 1.7401*^-21},
{993.14, 9.3236*^-22}, {1183.1, 4.9565*^-22}, {1409.4, 2.6144*^-22},
{1678.9, 1.3679*^-22}, {2000., 7.0973*^-23}},Method->Spline];
fxs[en*HartreeToeV]*crossSectioncm2toAU*UnitStep[en*HartreeToeV-71.933]*
UnitStep[2000.-en*HartreeToeV]
```

```
fsig012v112[en_]:=Module[{fxs},
fxs=Interpolation[{{557.18, 2.0368*^-19}, {595.95, 1.7186*^-19}, {637.41, 1.4438*^-19},
{681.76, 1.2105*^-19}, {729.2, 1.0135*^-19}, {779.93, 8.4753*^-20},
{834.2, 7.0789*^-20}, {892.24, 5.9052*^-20}, {954.32, 4.9196*^-20},
{1020.7, 4.0925*^-20}, {1091.7, 3.3991*^-20}, {1167.7, 2.8184*^-20},
{1248.9, 2.3329*^-20}, {1335.8, 1.9277*^-20}, {1428.8, 1.5904*^-20},
{1528.2, 1.3101*^-20}, {1634.5, 1.0778*^-20}, {1748.3, 8.8573*^-21},
{1869.9, 7.273*^-21}, {2000., 5.9687*^-21}},Method->Spline];
fxs[en*HartreeToeV]*crossSectioncm2toAU*UnitStep[en*HartreeToeV-557.18]*
UnitStep[2000.-en*HartreeToeV]
```

```
fsig102v112[en_]:=Module[{fxs},
fxs=Interpolation[{{84.647, 5.9874*^-19}, {99.976, 4.5983*^-19}, {118.08, 3.4689*^-19},
{139.47, 2.5746*^-19}, {164.72, 1.8818*^-19}, {194.55, 1.3555*^-19},
{229.79, 9.6308*^-20}, {271.4, 6.7551*^-20}, {320.55, 4.6796*^-20},
{378.6, 3.2023*^-20}, {447.16, 2.1661*^-20}, {528.14, 1.4498*^-20},
{623.78, 9.6054*^-21}, {736.75, 6.3027*^-21}, {870.17, 4.1005*^-21},
{1027.8, 2.6454*^-21}, {1213.9, 1.6936*^-21}, {1433.7, 1.0762*^-21},
{1693.3, 6.7896*^-22}, {2000., 4.2525*^-22}},Method->Spline];
fxs[en*HartreeToeV]*crossSectioncm2toAU*UnitStep[en*HartreeToeV-84.647]*
UnitStep[2000.-en*HartreeToeV]
```

```

fsig111v112[en_] := Module[{fxs},
fxs = Interpolation[{{74.963, 2.3787*^-18}, {89.106, 1.4994*^-18}, {105.92, 9.2926*^-19},
{125.9, 5.6705*^-19}, {149.66, 3.4097*^-19}, {177.89, 2.0215*^-19},
{211.46, 1.1824*^-19}, {251.35, 6.8279*^-20}, {298.78, 3.8949*^-20},
{355.15, 2.1966*^-20}, {422.15, 1.2264*^-20}, {501.8, 6.7874*^-21},
{596.48, 3.7278*^-21}, {709.02, 2.0343*^-21}, {842.79, 1.1041*^-21},
{1001.8, 5.9588*^-22}, {1190.8, 3.199*^-22}, {1415.5, 1.7065*^-22},
{1682.5, 9.0413*^-23}, {2000., 4.7515*^-23}}, Method -> Spline];
fxs[en*HartreeToeV]*crossSectioncm2toAU*UnitStep[en*HartreeToeV-74.963]*
UnitStep[2000.-en*HartreeToeV]

```

```

fsig021v121[en_] := Module[{fxs},
fxs = Interpolation[{{561.59, 1.9885*^-19}, {600.41, 1.6874*^-19}, {641.92, 1.4237*^-19},
{686.3, 1.1974*^-19}, {733.75, 1.0048*^-19}, {784.48, 8.414*^-20},
{838.71, 7.0331*^-20}, {896.69, 5.8688*^-20}, {958.69, 4.8895*^-20},
{1025., 4.0674*^-20}, {1095.8, 3.3788*^-20}, {1171.6, 2.8028*^-20},
{1252.6, 2.3219*^-20}, {1339.2, 1.921*^-20}, {1431.8, 1.5874*^-20},
{1530.7, 1.3102*^-20}, {1636.6, 1.0802*^-20}, {1749.7, 8.8954*^-21},
{1870.7, 7.318*^-21}, {2000., 6.0147*^-21}}, Method -> Spline];
fxs[en*HartreeToeV]*crossSectioncm2toAU*UnitStep[en*HartreeToeV-561.59]*
UnitStep[2000.-en*HartreeToeV]

```

```
fsig111v121[en_]:=Module[{fxs},
fxs=Interpolation[{{83.337, 1.2*^-18}, {98.51, 9.1219*^-19}, {116.45, 6.8329*^-19},
{137.65, 5.0487*^-19}, {162.71, 3.6821*^-19}, {192.33, 2.6517*^-19},
{227.35, 1.8865*^-19}, {268.74, 1.3262*^-19}, {317.67, 9.2127*^-20},
{375.5, 6.3245*^-20}, {443.87, 4.2915*^-20}, {524.68, 2.8798*^-20},
{620.21, 1.9117*^-20}, {733.13, 1.256*^-20}, {866.61, 8.1746*^-21},
{1024.4, 5.2724*^-21}, {1210.9, 3.3724*^-21}, {1431.4, 2.1401*^-21},
{1692., 1.3479*^-21}, {2000., 8.4275*^-22}},Method->Spline];
fxs[en*HartreeToeV]*crossSectioncm2toAU*UnitStep[en*HartreeToeV-83.337]*
UnitStep[2000.-en*HartreeToeV]]
```

```
fsig120v121[en_]:=Module[{fxs},
fxs=Interpolation[{{78.342, 1.224*^-18}, {92.907, 7.6776*^-19}, {110.18, 4.7286*^-19},
{130.66, 2.864*^-19}, {154.96, 1.7074*^-19}, {183.77, 1.0028*^-19},
{217.93, 5.8078*^-20}, {258.45, 3.3216*^-20}, {306.5, 1.8779*^-20},
{363.48, 1.0507*^-20}, {431.06, 5.83*^-21}, {511.2, 3.2153*^-21},
{606.25, 1.7645*^-21}, {718.96, 9.6489*^-22}, {852.62, 5.2649*^-22},
{1011.1, 2.8639*^-22}, {1199.1, 1.5535*^-22}, {1422.1, 8.3854*^-23},
{1686.5, 4.5013*^-23}, {2000., 2.3971*^-23}},Method->Spline];
fxs[en*HartreeToeV]*crossSectioncm2toAU*UnitStep[en*HartreeToeV-78.342]*
UnitStep[2000.-en*HartreeToeV]]
```

Minus four

```
fsig002v102[en_]:=Module[{fxs},
fxs=Interpolation[{{587.39, 1.7836*^-19}, {626.52, 1.5051*^-19}, {668.25, 1.2684*^-19},
{712.76, 1.0683*^-19}, {760.24, 8.9914*^-20}, {810.87, 7.5632*^-20},
{864.89, 6.3573*^-20}, {922.5, 5.3389*^-20}, {983.94, 4.4788*^-20},
{1049.5, 3.7524*^-20}, {1119.4, 3.1394*^-20}, {1194., 2.6223*^-20},
{1273.5, 2.1868*^-20}, {1358.3, 1.8206*^-20}, {1448.8, 1.5134*^-20},
{1545.3, 1.2563*^-20}, {1648.2, 1.0417*^-20}, {1758., 8.6288*^-21},
{1875.1, 7.1433*^-21}, {2000., 5.9109*^-21}},Method->Spline];
fxs[en*HartreeToeV]*crossSectioncm2toAU*UnitStep[en*HartreeToeV-587.39]*
UnitStep[2000.-en*HartreeToeV]
```

```
fsig101v102[en_]:=Module[{fxs},
fxs=Interpolation[{{97.216, 1.3179*^-18}, {113.99, 8.3543*^-19}, {133.65, 5.2486*^-19},
{156.71, 3.2686*^-19}, {183.75, 2.0182*^-19}, {215.45, 1.2355*^-19},
{252.62, 7.4996*^-20}, {296.2, 4.5141*^-20}, {347.3, 2.6944*^-20},
{407.21, 1.595*^-20}, {477.47, 9.3668*^-21}, {559.84, 5.4581*^-21},
{656.43, 3.1568*^-21}, {769.67, 1.8129*^-21}, {902.46, 1.0339*^-21},
{1058.2, 5.8576*^-22}, {1240.7, 3.2965*^-22}, {1454.8, 1.8427*^-22},
{1705.7, 1.023*^-22}, {2000., 5.6379*^-23}},Method->Spline];
fxs[en*HartreeToeV]*crossSectioncm2toAU*UnitStep[en*HartreeToeV-97.216]*
UnitStep[2000.-en*HartreeToeV]
```

```
fsig011v111[en_]:=Module[{fxs},
fxs=Interpolation[{{592.17, 1.7459*^-19}, {631.34, 1.4804*^-19}, {673.11, 1.2522*^-19},
{717.64, 1.0574*^-19}, {765.12, 8.917*^-20}, {815.73, 7.5095*^-20},
{869.7, 6.3161*^-20}, {927.23, 5.3058*^-20}, {988.57, 4.4516*^-20},
{1054., 3.7301*^-20}, {1123.7, 3.1217*^-20}, {1198., 2.6091*^-20},
{1277.3, 2.178*^-20}, {1361.8, 1.8158*^-20}, {1451.9, 1.512*^-20},
{1547.9, 1.2577*^-20}, {1650.3, 1.0449*^-20}, {1759.5, 8.6736*^-21},
{1875.9, 7.1935*^-21}, {2000., 5.9616*^-21}},Method->Spline];
fxs[en*HartreeToeV]*crossSectioncm2toAU*UnitStep[en*HartreeToeV-592.17]*
UnitStep[2000.-en*HartreeToeV]]
```

```
fsig101v111[en_]:=Module[{fxs},
fxs=Interpolation[{{106.91, 4.7614*^-19}, {124.73, 3.5983*^-19}, {145.52, 2.6877*^-19},
{169.77, 1.9854*^-19}, {198.07, 1.4512*^-19}, {231.08, 1.05*^-19},
{269.59, 7.524*^-20}, {314.52, 5.3412*^-20}, {366.95, 3.7575*^-20},
{428.1, 2.62*^-20}, {499.46, 1.8113*^-20}, {582.7, 1.2421*^-20},
{679.82, 8.4517*^-21}, {793.13, 5.7073*^-21}, {925.32, 3.8266*^-21},
{1079.5, 2.5482*^-21}, {1259.5, 1.6855*^-21}, {1469.4, 1.1078*^-21},
{1714.3, 7.2344*^-22}, {2000., 4.6953*^-22}},Method->Spline];
fxs[en*HartreeToeV]*crossSectioncm2toAU*UnitStep[en*HartreeToeV-106.91]*
UnitStep[2000.-en*HartreeToeV]]
```



```

fsig110v111[en_]:=Module[{fxs},
fxs=Interpolation[{{100.96, 6.7908*^-19}, {118.14, 4.2814*^-19}, {138.25, 2.6721*^-19},
{161.78, 1.6514*^-19}, {189.31, 1.0108*^-19}, {221.53, 6.1304*^-20},
{259.23, 3.6855*^-20}, {303.35, 2.1978*^-20}, {354.98, 1.3007*^-20},
{415.39, 7.643*^-21}, {486.09, 4.463*^-21}, {568.82, 2.5923*^-21},
{665.63, 1.4984*^-21}, {778.91, 8.6219*^-22}, {911.48, 4.9411*^-22},
{1066.6, 2.8197*^-22}, {1248.1, 1.6013*^-22}, {1460.5, 9.0487*^-23},
{1709.1, 5.0812*^-23}, {2000., 2.8349*^-23}},Method->Spline];
fxs[en*HartreeToeV]*crossSectioncm2toAU*UnitStep[en*HartreeToeV-100.96]*
UnitStep[2000.-en*HartreeToeV]]

```

```

fsig020v120[en_]:=Module[{fxs},
fxs=Interpolation[{{597.71, 1.7069*^-19}, {636.94, 1.4541*^-19}, {678.74, 1.2346*^-19},
{723.29, 1.0455*^-19}, {770.76, 8.8344*^-20}, {821.35, 7.4499*^-20},
{875.25, 6.2711*^-20}, {932.7, 5.2702*^-20}, {993.92, 4.4226*^-20},
{1059.1, 3.7065*^-20}, {1128.7, 3.1027*^-20}, {1202.7, 2.5947*^-20},
{1281.7, 2.1678*^-20}, {1365.8, 1.8097*^-20}, {1455.4, 1.5095*^-20},
{1551., 1.2581*^-20}, {1652.8, 1.0476*^-20}, {1761.2, 8.7158*^-21},
{1876.8, 7.2439*^-21}, {2000., 6.0151*^-21}},Method->Spline];
fxs[en*HartreeToeV]*crossSectioncm2toAU*UnitStep[en*HartreeToeV-597.71]*
UnitStep[2000.-en*HartreeToeV]]

```

```
fsig110v120[en_]:=Module[{fxs},
fxs=Interpolation[{{105.96, 9.4122*^-19}, {123.68, 7.0675*^-19}, {144.36, 5.2561*^-19},
{168.5, 3.8731*^-19}, {196.68, 2.8286*^-19}, {229.56, 2.0478*^-19},
{267.95, 1.4698*^-19}, {312.76, 1.0459*^-19}, {365.05, 7.3783*^-20},
{426.1, 5.1605*^-20}, {497.35, 3.5786*^-20}, {580.52, 2.4606*^-20},
{677.59, 1.6778*^-20}, {790.89, 1.1348*^-20}, {923.15, 7.6162*^-21},
{1077.5, 5.0735*^-21}, {1257.7, 3.3556*^-21}, {1468., 2.2043*^-21},
{1713.5, 1.4385*^-21}, {2000., 9.3281*^-22}},Method->Spline];
fxs[en*HartreeToeV]*crossSectioncm2toAU*UnitStep[en*HartreeToeV-105.96]*
UnitStep[2000.-en*HartreeToeV]
```

Minus five

```
fsig001v101[en_]:=Module[{fxs},
fxs=Interpolation[{{625.53, 1.5177*^-19}, {664.99, 1.2902*^-19}, {706.94, 1.0958*^-19},
{751.54, 9.2994*^-20}, {798.95, 7.8861*^-20}, {849.35, 6.6823*^-20},
{902.93, 5.6574*^-20}, {959.89, 4.7855*^-20}, {1020.4, 4.0439*^-20},
{1084.8, 3.4137*^-20}, {1153.2, 2.8785*^-20}, {1226., 2.4243*^-20},
{1303.3, 2.0394*^-20}, {1385.6, 1.7136*^-20}, {1473., 1.4382*^-20},
{1565.9, 1.2058*^-20}, {1664.7, 1.01*^-20}, {1769.7, 8.4522*^-21},
{1881.3, 7.0681*^-21}, {2000., 5.9077*^-21}},Method->Spline];
fxs[en*HartreeToeV]*crossSectioncm2toAU*UnitStep[en*HartreeToeV-625.53]*
UnitStep[2000.-en*HartreeToeV]
```

```

fsig100v101[en_]:=Module[{fxs},
fxs=Interpolation[{{125.13, 3.9757*^-19}, {144.78, 2.5538*^-19}, {167.52, 1.6304*^-19},
{193.83, 1.0346*^-19}, {224.27, 6.5263*^-20}, {259.49, 4.093*^-20},
{300.24, 2.5524*^-20}, {347.39, 1.5828*^-20}, {401.95, 9.7618*^-21},
{465.07, 5.9879*^-21}, {538.11, 3.6534*^-21}, {622.62, 2.2172*^-21},
{720.4, 1.3384*^-21}, {833.54, 8.0365*^-22}, {964.44, 4.7995*^-22},
{1115.9, 2.8506*^-22}, {1291.2, 1.6834*^-22}, {1493.9, 9.8839*^-23},
{1728.5, 5.7681*^-23}, {2000., 3.345*^-23}},Method->Spline];
fxs[en*HartreeToeV]*crossSectioncm2toAU*UnitStep[en*HartreeToeV-125.13]*
UnitStep[2000.-en*HartreeToeV]]

```

```

fsig010v110[en_]:=Module[{fxs},
fxs=Interpolation[{{631.4, 1.4873*^-19}, {670.9, 1.2695*^-19}, {712.87, 1.0816*^-19},
{757.47, 9.2017*^-20}, {804.86, 7.8167*^-20}, {855.21, 6.6312*^-20},
{908.72, 5.6183*^-20}, {965.57, 4.7544*^-20}, {1026., 4.0188*^-20},
{1090.2, 3.3935*^-20}, {1158.4, 2.8628*^-20}, {1230.8, 2.4128*^-20},
{1307.8, 2.0318*^-20}, {1389.7, 1.7095*^-20}, {1476.6, 1.4373*^-20},
{1569., 1.2075*^-20}, {1667.1, 1.0136*^-20}, {1771.4, 8.5011*^-21},
{1882.2, 7.1243*^-21}, {2000., 5.9656*^-21}},Method->Spline];
fxs[en*HartreeToeV]*crossSectioncm2toAU*UnitStep[en*HartreeToeV-631.4]*
UnitStep[2000.-en*HartreeToeV]]

```

```
fsig100v101[en_] := Module[{fxs},
fxs = Interpolation[{{125.13, 3.9757*^-19}, {144.78, 2.5538*^-19}, {167.52, 1.6304*^-19},
{193.83, 1.0346*^-19}, {224.27, 6.5263*^-20}, {259.49, 4.093*^-20},
{300.24, 2.5524*^-20}, {347.39, 1.5828*^-20}, {401.95, 9.7618*^-21},
{465.07, 5.9879*^-21}, {538.11, 3.6534*^-21}, {622.62, 2.2172*^-21},
{720.4, 1.3384*^-21}, {833.54, 8.0365*^-22}, {964.44, 4.7995*^-22},
{1115.9, 2.8506*^-22}, {1291.2, 1.6834*^-22}, {1493.9, 9.8839*^-23},
{1728.5, 5.7681*^-23}, {2000., 3.345*^-23}}, Method -> Spline];
fxs[en*HartreeToeV]*crossSectioncm2toAU*UnitStep[en*HartreeToeV-125.13]*
UnitStep[2000.-en*HartreeToeV]]
```

```
fsig100v110[en_] := Module[{fxs},
fxs = Interpolation[{{131.08, 3.7376*^-19}, {151.3, 2.813*^-19}, {174.63, 2.0998*^-19},
{201.56, 1.5551*^-19}, {232.64, 1.1429*^-19}, {268.52, 8.339*^-20},
{309.94, 6.0413*^-20}, {357.73, 4.3467*^-20}, {412.9, 3.1066*^-20},
{476.58, 2.2059*^-20}, {550.08, 1.5564*^-20}, {634.92, 1.0914*^-20},
{732.83, 7.6065*^-21}, {845.85, 5.2698*^-21}, {976.3, 3.6296*^-21},
{1126.9, 2.4856*^-21}, {1300.7, 1.6924*^-21}, {1501.2, 1.1459*^-21},
{1732.8, 7.7153*^-22}, {2000., 5.166*^-22}}, Method -> Spline];
fxs[en*HartreeToeV]*crossSectioncm2toAU*UnitStep[en*HartreeToeV-131.08]*
UnitStep[2000.-en*HartreeToeV]]
```

Minus six

```
fsig000v100[en_]:=Module[{fxs},
fxs=Interpolation[{{667.14, 1.2856*^-19}, {706.83, 1.1016*^-19}, {748.87, 9.431*^-20},
{793.42, 8.0667*^-20}, {840.62, 6.8936*^-20}, {890.62, 5.8858*^-20},
{943.6, 5.0208*^-20}, {999.74, 4.2792*^-20}, {1059.2, 3.644*^-20},
{1122.2, 3.1005*^-20}, {1189., 2.6358*^-20}, {1259.7, 2.239*^-20},
{1334.6, 1.9004*^-20}, {1414., 1.6118*^-20}, {1498.1, 1.366*^-20},
{1587.3, 1.1569*^-20}, {1681.7, 9.7898*^-21}, {1781.7, 8.2787*^-21},
{1887.7, 6.996*^-21}, {2000., 5.9084*^-21}},Method->Spline];
fxs[en*HartreeToeV]*crossSectioncm2toAU*UnitStep[en*HartreeToeV-667.14]*
UnitStep[2000.-en*HartreeToeV]
```

## Double core holes

Minus two

```
fsig013v023[en_]:=Module[{fxs},
fxs=Interpolation[{{68.795, 1.5759*^-18}, {82.145, 1.2317*^-18}, {98.086, 9.4244*^-19},
{117.12, 7.0747*^-19}, {139.85, 5.2166*^-19}, {166.99, 3.7803*^-19},
{199.39, 2.6936*^-19}, {238.08, 1.8885*^-19}, {284.29, 1.3031*^-19},
{339.45, 8.8471*^-20}, {405.33, 5.9111*^-20}, {483.98, 3.8911*^-20},
{577.9, 2.5246*^-20}, {690.05, 1.6159*^-20}, {823.96, 1.022*^-20},
{983.85, 6.3911*^-21}, {1174.8, 3.9586*^-21}, {1402.7, 2.4297*^-21},
{1675., 1.4797*^-21}, {2000., 8.9419*^-22}},Method->Spline];
fxs[en*HartreeToeV]*crossSectioncm2toAU*UnitStep[en*HartreeToeV-68.795]*
UnitStep[2000.-en*HartreeToeV]
```

```
fsig022v023[en_] := Module[{fxs},
fxs = Interpolation[{{61.01, 6.1248*^-18}, {73.311, 4.2154*^-18}, {88.093, 2.7661*^-18},
{105.85, 1.751*^-18}, {127.2, 1.0759*^-18}, {152.84, 6.4379*^-19},
{183.66, 3.7602*^-19}, {220.69, 2.1476*^-19}, {265.19, 1.201*^-19},
{318.66, 6.5855*^-20}, {382.91, 3.5473*^-20}, {460.12, 1.8822*^-20},
{552.89, 9.8587*^-21}, {664.37, 5.1111*^-21}, {798.33, 2.6297*^-21},
{959.29, 1.3441*^-21}, {1152.7, 6.8363*^-22}, {1385.1, 3.4577*^-22},
{1664.4, 1.7393*^-22}, {2000., 8.6911*^-23}}, Method -> Spline];
fxs[en*HartreeToeV]*crossSectioncm2toAU*UnitStep[en*HartreeToeV-61.01]*
UnitStep[2000.-en*HartreeToeV]
```

Minus three

```
fsig003v013[en_] := Module[{fxs},
fxs = Interpolation[{{91.558, 6.2617*^-19}, {107.69, 4.8086*^-19}, {126.67, 3.6361*^-19},
{148.99, 2.71*^-19}, {175.25, 1.9917*^-19}, {206.14, 1.4439*^-19},
{242.46, 1.0331*^-19}, {285.19, 7.2984*^-20}, {335.45, 5.0933*^-20},
{394.56, 3.511*^-20}, {464.1, 2.3913*^-20}, {545.88, 1.6107*^-20},
{642.08, 1.0737*^-20}, {755.24, 7.0847*^-21}, {888.33, 4.633*^-21},
{1044.9, 3.0051*^-21}, {1229., 1.9338*^-21}, {1445.6, 1.2361*^-21},
{1700.4, 7.8468*^-22}, {2000., 4.9516*^-22}}, Method -> Spline];
fxs[en*HartreeToeV]*crossSectioncm2toAU*UnitStep[en*HartreeToeV-91.558]*
UnitStep[2000.-en*HartreeToeV]
```

```

fsig012v013[en_]:=Module[{fxs},
fxs=Interpolation[{{82.493, 3.6079*^-18}, {97.564, 2.3608*^-18}, {115.39, 1.5139*^-18},
{136.47, 9.5361*^-19}, {161.4, 5.9078*^-19}, {190.89, 3.6024*^-19},
{225.77, 2.1633*^-19}, {267.02, 1.2801*^-19}, {315.8, 7.4673*^-20},
{373.5, 4.2964*^-20}, {441.73, 2.4402*^-20}, {522.44, 1.3699*^-20},
{617.89, 7.6099*^-21}, {730.78, 4.1879*^-21}, {864.29, 2.2866*^-21},
{1022.2, 1.2398*^-21}, {1208.9, 6.6783*^-22}, {1429.8, 3.5764*^-22},
{1691., 1.9034*^-22}, {2000., 1.0069*^-22}},Method->Spline];
fxs[en*HartreeToeV]*crossSectioncm2toAU*UnitStep[en*HartreeToeV-82.493]*
UnitStep[2000.-en*HartreeToeV]]

```

```

fsig012v022[en_]:=Module[{fxs},
fxs=Interpolation[{{90.278, 1.2516*^-18}, {106.27, 9.5324*^-19}, {125.09, 7.1663*^-19},
{147.24, 5.3211*^-19}, {173.31, 3.9033*^-19}, {204.01, 2.829*^-19},
{240.14, 2.026*^-19}, {282.67, 1.434*^-19}, {332.73, 1.0031*^-19},
{391.65, 6.9334*^-20}, {461.01, 4.7356*^-20}, {542.66, 3.1976*^-20},
{638.76, 2.1356*^-20}, {751.89, 1.4111*^-20}, {885.04, 9.2344*^-21},
{1041.8, 5.9892*^-21}, {1226.3, 3.8521*^-21}, {1443.5, 2.4595*^-21},
{1699.1, 1.5592*^-21}, {2000., 9.823*^-22}},Method->Spline];
fxs[en*HartreeToeV]*crossSectioncm2toAU*UnitStep[en*HartreeToeV-90.278]*
UnitStep[2000.-en*HartreeToeV]]

```

```
fsig021v022[en_] := Module[{fxs},
fxs = Interpolation[{{86.317, 2.4609*^-18}, {101.84, 1.6027*^-18}, {120.16, 1.0217*^-18},
{141.78, 6.3921*^-19}, {167.28, 3.9301*^-19}, {197.37, 2.3767*^-19},
{232.88, 1.4151*^-19}, {274.77, 8.3033*^-20}, {324.19, 4.8063*^-20},
{382.51, 2.7464*^-20}, {451.32, 1.5512*^-20}, {532.5, 8.6776*^-21},
{628.29, 4.8158*^-21}, {741.31, 2.6539*^-21}, {874.66, 1.4552*^-21},
{1032., 7.9457*^-22}, {1217.6, 4.3193*^-22}, {1436.7, 2.3396*^-22},
{1695.1, 1.2606*^-22}, {2000., 6.7602*^-23}}, Method -> Spline];
fxs[en*HartreeToeV]*crossSectioncm2toAU*UnitStep[en*HartreeToeV-86.317]*
UnitStep[2000.-en*HartreeToeV]
```

Minus four

```
fsig002v003[en_] := Module[{fxs},
fxs = Interpolation[{{105.8, 2.0934*^-18}, {123.5, 1.3665*^-18}, {144.16, 8.8246*^-19},
{168.28, 5.6395*^-19}, {196.44, 3.5672*^-19}, {229.31, 2.2335*^-19},
{267.67, 1.3842*^-19}, {312.46, 8.4903*^-20}, {364.74, 5.154*^-20},
{425.76, 3.0965*^-20}, {496.99, 1.8415*^-20}, {580.15, 1.0844*^-20},
{677.21, 6.3249*^-21}, {790.52, 3.6563*^-21}, {922.78, 2.0961*^-21},
{1077.2, 1.1924*^-21}, {1257.4, 6.7348*^-22}, {1467.8, 3.7787*^-22},
{1713.3, 2.1069*^-22}, {2000., 1.1678*^-22}}, Method -> Spline];
fxs[en*HartreeToeV]*crossSectioncm2toAU*UnitStep[en*HartreeToeV-105.8]*
UnitStep[2000.-en*HartreeToeV]
```



```

fsig011v021[en_]:=Module[{fxs},
fxs=Interpolation[{{113.92, 9.7304*^-19}, {132.46, 7.3443*^-19}, {154.03, 5.4947*^-19},
{179.1, 4.0754*^-19}, {208.25, 2.9965*^-19}, {242.15, 2.1842*^-19},
{281.56, 1.5783*^-19}, {327.4, 1.1305*^-19}, {380.69, 8.0262*^-20},
{442.66, 5.6477*^-20}, {514.71, 3.9385*^-20}, {598.49, 2.7224*^-20},
{695.91, 1.8658*^-20}, {809.19, 1.2681*^-20}, {940.91, 8.5501*^-21},
{1094.1, 5.7228*^-21}, {1272.2, 3.8039*^-21}, {1479.2, 2.5121*^-21},
{1720., 1.6492*^-21}, {2000., 1.0765*^-21}},Method->Spline];
fxs[en*HartreeToeV]*crossSectioncm2toAU*UnitStep[en*HartreeToeV-113.92]*
UnitStep[2000.-en*HartreeToeV]]

```

```

fsig002v012[en_]:=Module[{fxs},
fxs=Interpolation[{{114.87, 4.9265*^-19}, {133.51, 3.738*^-19}, {155.17, 2.8067*^-19},
{180.35, 2.0861*^-19}, {209.62, 1.535*^-19}, {243.63, 1.1184*^-19},
{283.17, 8.0706*^-20}, {329.12, 5.7691*^-20}, {382.52, 4.0861*^-20},
{444.6, 2.8675*^-20}, {516.74, 1.9942*^-20}, {600.59, 1.375*^-20},
{698.05, 9.404*^-21}, {811.32, 6.3809*^-21}, {942.97, 4.2974*^-21},
{1096., 2.8749*^-21}, {1273.8, 1.9107*^-21}, {1480.5, 1.2621*^-21},
{1720.8, 8.2908*^-22}, {2000., 5.4154*^-22}},Method->Spline];
fxs[en*HartreeToeV]*crossSectioncm2toAU*UnitStep[en*HartreeToeV-114.87]*
UnitStep[2000.-en*HartreeToeV]]

```

```
fsig011v012[en_] := Module[{fxs},
fxs = Interpolation[{{109.96, 1.4296*^-18}, {128.1, 9.2855*^-19}, {149.23, 5.9609*^-19},
{173.84, 3.7839*^-19}, {202.51, 2.3756*^-19}, {235.92, 1.4755*^-19},
{274.83, 9.0686*^-20}, {320.16, 5.5177*^-20}, {372.97, 3.3247*^-20},
{434.49, 1.9846*^-20}, {506.16, 1.1741*^-20}, {589.64, 6.8911*^-21},
{686.9, 4.0156*^-21}, {800.2, 2.3244*^-21}, {932.19, 1.3374*^-21},
{1086., 7.6559*^-22}, {1265.1, 4.3597*^-22}, {1473.7, 2.4703*^-22},
{1716.8, 1.393*^-22}, {2000., 7.8116*^-23}}, Method -> Spline];
fxs[en*HartreeToeV]*crossSectioncm2toAU*UnitStep[en*HartreeToeV-109.96]*
UnitStep[2000.-en*HartreeToeV]
```

```
fsig020v021[en_] := Module[{fxs},
fxs = Interpolation[{{114.47, 7.2876*^-19}, {133.07, 4.7086*^-19}, {154.69, 3.0052*^-19},
{179.83, 1.8955*^-19}, {209.04, 1.1818*^-19}, {243.01, 7.2858*^-20},
{282.49, 4.4438*^-20}, {328.39, 2.6839*^-20}, {381.75, 1.6064*^-20},
{443.78, 9.5338*^-21}, {515.89, 5.6145*^-21}, {599.71, 3.2857*^-21},
{697.15, 1.9137*^-21}, {810.42, 1.1097*^-21}, {942.1, 6.4098*^-22},
{1095.2, 3.6929*^-22}, {1273.1, 2.1211*^-22}, {1480., 1.2138*^-22},
{1720.5, 6.9249*^-23}, {2000., 3.9305*^-23}}, Method -> Spline];
fxs[en*HartreeToeV]*crossSectioncm2toAU*UnitStep[en*HartreeToeV-114.47]*
UnitStep[2000.-en*HartreeToeV]
```

Minus five

```

fsig001v002[en_]:=Module[{fxs},
fxs=Interpolation[{{135.36, 8.6316*^-19}, {155.97, 5.6798*^-19}, {179.72, 3.7102*^-19},
{207.09, 2.4061*^-19}, {238.62, 1.5491*^-19}, {274.96, 9.9013*^-20},
{316.82, 6.2825*^-20}, {365.07, 3.9571*^-20}, {420.66, 2.4742*^-20},
{484.71, 1.5357*^-20}, {558.52, 9.4624*^-21}, {643.56, 5.789*^-21},
{741.56, 3.517*^-21}, {854.48, 2.1224*^-21}, {984.59, 1.2726*^-21},
{1134.5, 7.5835*^-22}, {1307.3, 4.4926*^-22}, {1506.3, 2.6468*^-22},
{1735.7, 1.551*^-22}, {2000., 9.0414*^-23}},Method->Spline];
fxs[en*HartreeToeV]*crossSectioncm2toAU*UnitStep[en*HartreeToeV-135.36]*
UnitStep[2000.-en*HartreeToeV]]

```

```

fsig001v011[en_]:=Module[{fxs},
fxs=Interpolation[{{140.27, 3.856*^-19}, {161.33, 2.9178*^-19}, {185.54, 2.1912*^-19},
{213.4, 1.6334*^-19}, {245.43, 1.2086*^-19}, {282.27, 8.8774*^-20},
{324.64, 6.4738*^-20}, {373.38, 4.6876*^-20}, {429.42, 3.3706*^-20},
{493.89, 2.4069*^-20}, {568.03, 1.707*^-20}, {653.29, 1.2026*^-20},
{751.36, 8.4186*^-21}, {864.15, 5.8569*^-21}, {993.87, 4.0502*^-21},
{1143.1, 2.785*^-21}, {1314.6, 1.9046*^-21}, {1512., 1.2957*^-21},
{1739., 8.7707*^-22}, {2000., 5.9084*^-22}},Method->Spline];
fxs[en*HartreeToeV]*crossSectioncm2toAU*UnitStep[en*HartreeToeV-140.27]*
UnitStep[2000.-en*HartreeToeV]]

```

```

fsig010v011[en_]:=Module[{fxs},
fxs=Interpolation[{{140.2, 4.3976*^-19}, {161.25, 2.8791*^-19}, {185.46, 1.87*^-19},
{213.31, 1.2052*^-19}, {245.33, 7.7062*^-20}, {282.17, 4.8898*^-20},
{324.53, 3.0798*^-20}, {373.26, 1.9262*^-20}, {429.3, 1.1967*^-20},
{493.76, 7.3874*^-21}, {567.89, 4.5326*^-21}, {653.16, 2.7656*^-21},
{751.22, 1.6793*^-21}, {864.01, 1.015*^-21}, {993.74, 6.108*^-22},
{1142.9, 3.6604*^-22}, {1314.5, 2.1854*^-22}, {1511.9, 1.2993*^-22},
{1738.9, 7.6914*^-23}, {2000., 4.5344*^-23}},Method->Spline];
fxs[en*HartreeToeV]*crossSectioncm2toAU*UnitStep[en*HartreeToeV-140.2]*
UnitStep[2000.-en*HartreeToeV]]

```

```

fsig010v020[en_]:=Module[{fxs},
fxs=Interpolation[{{139.65, 7.5582*^-19}, {160.65, 5.7*^-19}, {184.81, 4.2715*^-19},
{212.6, 3.1807*^-19}, {244.57, 2.3534*^-19}, {281.35, 1.7301*^-19},
{323.66, 1.2637*^-19}, {372.33, 9.1695*^-20}, {428.32, 6.6091*^-20},
{492.74, 4.7317*^-20}, {566.83, 3.3646*^-20}, {652.08, 2.3764*^-20},
{750.13, 1.6671*^-20}, {862.94, 1.1619*^-20}, {992.71, 8.0459*^-21},
{1142., 5.5378*^-21}, {1313.7, 3.7892*^-21}, {1511.3, 2.5784*^-21},
{1738.6, 1.7454*^-21}, {2000., 1.1755*^-21}},Method->Spline];
fxs[en*HartreeToeV]*crossSectioncm2toAU*UnitStep[en*HartreeToeV-139.65]*
UnitStep[2000.-en*HartreeToeV]]

```

Minus six

```
fsig000v010[en_] := Module[{fxs},
fxs = Interpolation[{{166.82, 3.0119*^-19}, {190.12, 2.2878*^-19}, {216.67, 1.7276*^-19},
{246.93, 1.2971*^-19}, {281.42, 9.6825*^-20}, {320.73, 7.187*^-20},
{365.52, 5.3049*^-20}, {416.58, 3.8942*^-20}, {474.76, 2.8431*^-20},
{541.07, 2.0647*^-20}, {616.63, 1.4915*^-20}, {702.76, 1.0719*^-20},
{800.91, 7.6642*^-21}, {912.77, 5.4529*^-21}, {1040.3, 3.8608*^-21},
{1185.5, 2.7205*^-21}, {1351.1, 1.9081*^-21}, {1539.8, 1.3323*^-21},
{1754.9, 9.261*^-22}, {2000., 6.4096*^-22}}, Method -> Spline];
fxs[en*HartreeToeV]*crossSectioncm2toAU*UnitStep[en*HartreeToeV-166.82]*
UnitStep[2000.-en*HartreeToeV]]
```

```
fsig000v001[en_] := Module[{fxs},
fxs = Interpolation[{{166.74, 2.7673*^-19}, {190.03, 1.8497*^-19}, {216.58, 1.2294*^-19},
{246.83, 8.1249*^-20}, {281.32, 5.3398*^-20}, {320.62, 3.49*^-20},
{365.4, 2.2685*^-20}, {416.45, 1.4665*^-20}, {474.63, 9.4299*^-21},
{540.93, 6.0312*^-21}, {616.49, 3.8371*^-21}, {702.62, 2.4284*^-21},
{800.77, 1.529*^-21}, {912.63, 9.5777*^-22}, {1040.1, 5.9697*^-22},
{1185.4, 3.7026*^-22}, {1351., 2.2853*^-22}, {1539.8, 1.4039*^-22},
{1754.9, 8.5848*^-23}, {2000., 5.2254*^-23}}, Method -> Spline];
fxs[en*HartreeToeV]*crossSectioncm2toAU*UnitStep[en*HartreeToeV-166.74]*
UnitStep[2000.-en*HartreeToeV]]
```

## Total ionization cross sections

### No core holes

```
fsigTot200[en_] := fsig100v200[en]
fsigTot201[en_] := fsig200v201[en] + fsig101v201[en]
fsigTot202[en_] := fsig201v202[en] + fsig102v202[en]
fsigTot203[en_] := fsig202v203[en] + fsig103v203[en]
fsigTot210[en_] := fsig200v210[en] + fsig110v210[en]
fsigTot211[en_] := fsig201v211[en] + fsig210v211[en] + fsig111v211[en]
fsigTot212[en_] := fsig202v212[en] + fsig211v212[en] + fsig112v212[en]
fsigTot213[en_] := fsig212v213[en] + fsig203v213[en] + fsig113v213[en]
fsigTot220[en_] := fsig210v220[en] + fsig120v220[en]
fsigTot221[en_] := fsig220v221[en] + fsig121v221[en] + fsig211v221[en]
fsigTot222[en_] := fsig212v222[en] + fsig221v222[en] + fsig122v222[en]
fsigTot223[en_] := fsig123v223[en] + fsig213v223[en] + fsig222v223[en]
```

## Single core holes

```

fsigTot100[en_] := fsig000v100[en] (* Exception: no inclDCH[truth] *)
fsigTot110[en_, truth_] := fsig100v110[en] + inclDCH[truth] * fsig010v110[en]
fsigTot101[en_, truth_] := fsig100v101[en] + inclDCH[truth] * fsig001v101[en]
fsigTot102[en_, truth_] := fsig101v102[en] + inclDCH[truth] * fsig002v102[en]
fsigTot103[en_, truth_] := fsig102v103[en] + inclDCH[truth] * fsig003v103[en]
fsigTot111[en_, truth_] := fsig101v111[en] + fsig110v111[en] + inclDCH[truth] * fsig011v111[en]
fsigTot112[en_, truth_] := fsig102v112[en] + fsig111v112[en] + inclDCH[truth] * fsig012v112[en]
fsigTot113[en_, truth_] := fsig103v113[en] + fsig112v113[en] + inclDCH[truth] * fsig013v113[en]
fsigTot120[en_, truth_] := fsig110v120[en] + inclDCH[truth] * fsig020v120[en]
fsigTot121[en_, truth_] := fsig111v121[en] + fsig120v121[en] + inclDCH[truth] * fsig021v121[en]
fsigTot122[en_, truth_] := fsig112v122[en] + fsig121v122[en] + inclDCH[truth] * fsig022v122[en]
fsigTot123[en_, truth_] := fsig113v123[en] + fsig122v123[en] + inclDCH[truth] * fsig023v123[en]

```

## Double core holes

```

fsigTot010[en_, truth_] := inclDCH[truth] * fsig000v010[en]
fsigTot020[en_, truth_] := inclDCH[truth] * fsig010v020[en]
fsigTot001[en_, truth_] := inclDCH[truth] * fsig000v001[en]
fsigTot002[en_, truth_] := inclDCH[truth] * fsig001v002[en]
fsigTot003[en_, truth_] := inclDCH[truth] * fsig002v003[en]
fsigTot011[en_, truth_] := inclDCH[truth] * (fsig010v011[en] + fsig001v011[en])
fsigTot012[en_, truth_] := inclDCH[truth] * (fsig011v012[en] + fsig002v012[en])
fsigTot013[en_, truth_] := inclDCH[truth] * (fsig003v013[en] + fsig012v013[en])
fsigTot021[en_, truth_] := inclDCH[truth] * (fsig011v021[en] + fsig020v021[en])
fsigTot022[en_, truth_] := inclDCH[truth] * (fsig012v022[en] + fsig021v022[en])
fsigTot023[en_, truth_] := inclDCH[truth] * (fsig013v023[en] + fsig022v023[en])

```

## Rate equations

### Neutral

#### No core holes

```
req223[en_,jxpulse_]:=P223'[t]==-fsigTot223[en]*P223[t]*jxpulse[t]
(* the state does not decay *)
ieq223[neginf_,inival_]:=P223[neginf]==inival
```

### Minus one

#### No core holes

```
req213[en_,jxpulse_]:=P213'[t]==(fsig213v223[en]*P223[t]-fsigTot213[en]*P213[t]) *
jxpulse[t]-GamR222v213*P213[t]
ieq213[neginf_,inival_]:=P213[neginf]==inival

req222[en_,jxpulse_]:=P222'[t]==(fsig222v223[en]*P223[t]-fsigTot222[en]*P222[t]) *
jxpulse[t]+GamR222v213*P213[t] (* the state does not decay *)
ieq222[neginf_,inival_]:=P222[neginf]==inival
```

#### Single core hole

```
req123[en_,jxpulse_,truth_]:=P123'[t]==(fsig123v223[en]*P223[t]-fsigTot123[en,truth] *
P123[t])*jxpulse[t]-GamATot123*P123[t]
ieq123[neginf_,inival_]:=P123[neginf]==inival
```



## Minus two

### No core holes

```

req203[en_,jxpulse_] := P203'[t] == (fsig203v213[en]*P213[t] - fsigTot203[en]*P203[t]) *
    jxpulse[t] + GamA203v123*P123[t] - GamR212v203*P203[t]
ieq203[neginf_,inival_] := P203[neginf] == inival

req212[en_,jxpulse_] := P212'[t] == (fsig212v222[en]*P222[t] + fsig212v213[en]*P213[t] -
    fsigTot212[en]*P212[t]) * jxpulse[t] + GamA212v123*P123[t] + GamR212v203*P203[t] -
    GamR221v212*P212[t]
ieq212[neginf_,inival_] := P212[neginf] == inival

req221[en_,jxpulse_] := P221'[t] == (fsig221v222[en]*P222[t] - fsigTot221[en]*P221[t]) *
    jxpulse[t] + GamA221v123*P123[t] + GamR221v212*P212[t]
    (* the state does not decay *)
ieq221[neginf_,inival_] := P221[neginf] == inival

```

### Single core hole

```

req113[en_,jxpulse_,truth_] := P113'[t] == (fsig113v213[en]*P213[t] + fsig113v123[en]*P123[t] -
    fsigTot113[en,truth]*P113[t]) * jxpulse[t] - GamATot113*P113[t]
ieq113[neginf_,inival_] := P113[neginf] == inival

req122[en_,jxpulse_,truth_] := P122'[t] == (fsig122v222[en]*P222[t] + fsig122v123[en]*P123[t] -
    fsigTot122[en,truth]*P122[t]) * jxpulse[t] - GamATot122*P122[t]
ieq122[neginf_,inival_] := P122[neginf] == inival

```

## Double core hole

```
req023[en_,jxpulse_,truth_]:=P023'[t]==inclDCH[truth]*((fsig023v123[en]*P123[t] -
    fsigTot023[en,truth]*P023[t])*jxpulse[t]-GamATot023*P023[t])
ieq023[neginf_,inival_]:=P023[neginf]==inival
```

## Minus three

### No core holes

```
req202[en_,jxpulse_]:=P202'[t]==(fsig202v203[en]*P203[t]+fsig202v212[en]*P212[t] -
    fsigTot202[en]*P202[t])*jxpulse[t]+GamA202v113*P113[t]+GamA202v122*P122[t] -
    GamR211v202*P202[t]
ieq202[neginf_,inival_]:=P202[neginf]==inival

req211[en_,jxpulse_]:=P211'[t]==(fsig211v212[en]*P212[t]+fsig211v221[en]*P221[t] -
    fsigTot211[en]*P211[t])*jxpulse[t]+GamA211v113*P113[t]+GamA211v122*P122[t] +
    GamR211v202*P202[t]-GamR220v211*P211[t]
ieq211[neginf_,inival_]:=P211[neginf]==inival

req220[en_,jxpulse_]:=P220'[t]==(fsig220v221[en]*P221[t]-fsigTot220[en]*P220[t]) *
    jxpulse[t]+GamA220v122*P122[t]+GamR220v211*P211[t]
    (* the state does not decay *)
ieq220[neginf_,inival_]:=P220[neginf]==inival
```

## Single core hole

```

req103[en_,jxpulse_,truth_]:=P103'[t]==(fsig103v203[en]*P203[t]+fsig103v113[en]*P113[t] -
      fsigTot103[en,truth]*P103[t])*jxpulse[t]+GamA103v023*P023[t]-GamATot103*P103[t]
ieq103[neginf_,inival_]:=P103[neginf]==inival

req112[en_,jxpulse_,truth_]:=P112'[t]==(fsig112v212[en]*P212[t]+fsig112v113[en]*P113[t] +
      fsig112v122[en]*P122[t]-fsigTot112[en,truth]*P112[t])*jxpulse[t] +
      GamA112v023*P023[t]-GamATot112*P112[t]
ieq112[neginf_,inival_]:=P112[neginf]==inival

req121[en_,jxpulse_,truth_]:=P121'[t]==(fsig121v221[en]*P221[t]+fsig121v122[en]*P122[t] -
      fsigTot121[en,truth]*P121[t])*jxpulse[t]+GamA121v023*P023[t]-GamATot121*P121[t]
ieq121[neginf_,inival_]:=P121[neginf]==inival

```

## Double core hole

```

req013[en_,jxpulse_,truth_]:=P013'[t]==inclDCH[truth]*( (fsig013v113[en]*P113[t] +
      fsig013v023[en]*P023[t]-fsigTot013[en,truth]*P013[t])*jxpulse[t] -
      GamATot013*P013[t])
ieq013[neginf_,inival_]:=P013[neginf]==inival

req022[en_,jxpulse_,truth_]:=P022'[t]==inclDCH[truth]*( (fsig022v122[en]*P122[t] +
      fsig022v023[en]*P023[t]-fsigTot022[en,truth]*P022[t])*jxpulse[t] -
      GamATot022*P022[t])
ieq022[neginf_,inival_]:=P022[neginf]==inival

```

## Minus four

### No core holes

```

req201[en_,jxpulse_] := P201'[t] == (fsig201v211[en]*P211[t] + fsig201v202[en]*P202[t] -
    fsigTot201[en]*P201[t])*jxpulse[t] + GamA201v112*P112[t] + GamA201v103*P103[t] +
    GamA201v121*P121[t] - GamR210v201*P201[t]
ieq201[neginf_,inival_] := P201[neginf] == inival

req210[en_,jxpulse_] := P210'[t] == (fsig210v211[en]*P211[t] + fsig210v220[en]*P220[t] -
    fsigTot210[en]*P210[t])*jxpulse[t] + GamA210v112*P112[t] + GamA210v121*P121[t] +
    GamR210v201*P201[t] (* the state does not decay *)
ieq210[neginf_,inival_] := P210[neginf] == inival

```

### Single core hole

```

req102[en_,jxpulse_,truth_] := P102'[t] == (fsig102v202[en]*P202[t] + fsig102v103[en]*P103[t] +
    fsig102v112[en]*P112[t] - fsigTot102[en,truth]*P102[t])*jxpulse[t] +
    GamA102v022*P022[t] + GamA102v013*P013[t] - GamATot102*P102[t]
ieq102[neginf_,inival_] := P102[neginf] == inival

req111[en_,jxpulse_,truth_] := P111'[t] == (fsig111v211[en]*P211[t] + fsig111v121[en]*P121[t] +
    fsig111v112[en]*P112[t] - fsigTot111[en,truth]*P111[t])*jxpulse[t] +
    GamA111v022*P022[t] + GamA111v013*P013[t] - GamATot111*P111[t]
ieq111[neginf_,inival_] := P111[neginf] == inival

req120[en_,jxpulse_,truth_] := P120'[t] == (fsig120v220[en]*P220[t] + fsig120v121[en]*P121[t] -
    fsigTot120[en,truth]*P120[t])*jxpulse[t] + GamA120v022*P022[t] - GamATot120*P120[t]
ieq120[neginf_,inival_] := P120[neginf] == inival

```

## Double core hole

```

req003[en_,jxpulse_,truth_]:=P003'[t]==inclDCH[truth]*((fsig003v103[en]*P103[t] +
    fsig003v013[en]*P013[t]-fsigTot003[en,truth]*P003[t])*jxpulse[t] -
    GamATot003*P003[t])
ieq003[neginf_,inival_]:=P003[neginf]==inival

req012[en_,jxpulse_,truth_]:=P012'[t]==inclDCH[truth]*((fsig012v112[en]*P112[t] +
    fsig012v013[en]*P013[t]+fsig012v022[en]*P022[t]-fsigTot012[en,truth]*P012[t]) *
    jxpulse[t]-GamATot012*P012[t])
ieq012[neginf_,inival_]:=P012[neginf]==inival

req021[en_,jxpulse_,truth_]:=P021'[t]==inclDCH[truth]*((fsig021v121[en]*P121[t] +
    fsig021v022[en]*P022[t]-fsigTot021[en,truth]*P021[t])*jxpulse[t] -
    GamATot021*P021[t])
ieq021[neginf_,inival_]:=P021[neginf]==inival

```

## Minus five

### No core holes

```

req200[en_,jxpulse_]:=P200'[t]==(fsig200v201[en]*P201[t]+fsig200v210[en]*P210[t] -
    fsigTot200[en]*P200[t])*jxpulse[t]+GamA200v111*P111[t]+GamA200v102*P102[t] +
    GamA200v120*P120[t]+GamR200v110*P110[t]+GamR200v101*P101[t]
(* the state does not decay *)
ieq200[neginf_,inival_]:=P200[neginf]==inival

```

## Single core hole

```

req101[en_,jxpulse_,truth_]:=P101'[t]==(fsig101v201[en]*P201[t]+fsig101v102[en] *
      P102[t]+fsig101v111[en]*P111[t]-fsigTot101[en,truth]*P101[t])*jxpulse[t] +
      GamA101v003*P003[t]+GamA101v012*P012[t]+GamA101v021*P021[t]-GamR200v101*P101[t]
ieq101[neginf_,inival_]:=P101[neginf]==inival

req110[en_,jxpulse_,truth_]:=P110'[t]==(fsig110v210[en]*P210[t]+fsig110v111[en] *
      P111[t]+fsig110v120[en]*P120[t]-fsigTot110[en,truth]*P110[t])*jxpulse[t] +
      GamA110v012*P012[t]+GamA110v021*P021[t]-GamR200v110*P110[t]
ieq110[neginf_,inival_]:=P110[neginf]==inival

```

## Double core hole

```

req002[en_,jxpulse_,truth_]:=P002'[t]==inclDCH[truth]*( (fsig002v102[en]*P102[t] +
      fsig002v012[en]*P012[t]+fsig002v003[en]*P003[t]-fsigTot002[en,truth] *
      P002[t])*jxpulse[t]-GamATot002*P002[t])
ieq002[neginf_,inival_]:=P002[neginf]==inival

req011[en_,jxpulse_,truth_]:=P011'[t]==inclDCH[truth]*( (fsig011v021[en]*P021[t] +
      fsig011v111[en]*P111[t]+fsig011v012[en]*P012[t]-fsigTot011[en,truth]*P011[t]) *
      jxpulse[t]-GamATot011*P011[t])
ieq011[neginf_,inival_]:=P011[neginf]==inival

req020[en_,jxpulse_,truth_]:=P020'[t]==inclDCH[truth]*( (fsig020v120[en]*P120[t] +
      fsig020v021[en]*P021[t]-fsigTot020[en,truth]*P020[t])*jxpulse[t] -
      GamATot020*P020[t])
ieq020[neginf_,inival_]:=P020[neginf]==inival

```

## Minus six

### Single core hole

```
req100[en_,jxpulse_]:=P100'[t]==(fsig100v200[en]*P200[t]+fsig100v101[en]*P101[t] +
    fsig100v110[en]*P110[t]-fsigTot100[en]*P100[t])*jxpulse[t]+GamA100v011 *
    P011[t]+GamA100v002*P002[t]+GamA100v020*P020[t]+GamR100v010*P010[t] +
    GamR100v001*P001[t] (* the state does not decay *)
ieq100[neginf_,inival_]:=P100[neginf]==inival
```

### Double core hole

```
req010[en_,jxpulse_,truth_]:=P010'[t]==inclDCH[truth]*( (fsig010v110[en]*P110[t] +
    fsig010v011[en]*P011[t]+fsig010v020[en]*P020[t]-fsigTot010[en,truth]*P010[t]) *
    jxpulse[t]-GamR100v010*P010[t])
ieq010[neginf_,inival_]:=P010[neginf]==inival

req001[en_,jxpulse_,truth_]:=P001'[t]==inclDCH[truth]*( (fsig001v101[en]*P101[t] +
    fsig001v002[en]*P002[t]+fsig001v011[en]*P011[t]-fsigTot001[en,truth]*P001[t]) *
    jxpulse[t]-GamR100v001*P001[t])
ieq001[neginf_,inival_]:=P001[neginf]==inival
```

## Minus seven

### Double core hole

```
req000[en_,jxpulse_]:=P000'[t]==(fsig000v100[en]*P100[t]+fsig000v010[en]*P010[t] +
      fsig000v001[en]*P001[t])*jxpulse[t] (* the state does not decay *)
ieq000[neginf_,inival_]:=P000[neginf]==inival
```

## Private section

```
Begin["`Private`"]
```

## Unit conversions

```
HartreeToeV:=27.2113845
eVToHartree:=1/HartreeToeV
BohrToAngstroem:=0.5291772083
crossSectionAtoBarn:=1*^8*BohrToAngstroem^2
crossSectionAtocm2:=crossSectionAtoBarn*1*^-24
crossSectioncm2toAU:=1/crossSectionAtocm2
```



## Decay widths

### No core holes

#### X-ray fluorescence

```
GamR222v213:=9.96819*^-7*eVToHartree  
GamR221v212:=3.82671*^-7*eVToHartree  
GamR220v211:=8.27037*^-8*eVToHartree  
GamR212v203:=2.80961*^-6*eVToHartree  
GamR211v202:=1.06412*^-6*eVToHartree  
GamR210v201:=2.29608*^-7*eVToHartree
```

### Single core holes

#### Auger decay

```
GamA203v123:=0.0253196*eVToHartree  
GamA212v123:=0.0374206*eVToHartree  
GamA221v123:=0.0351225*eVToHartree  
GamATot123 :=GamA203v123+GamA212v123+GamA221v123
```

```
GamA202v122:=0.0311014*eVToHartree  
GamA211v122:=0.0321728*eVToHartree  
GamA220v122:=0.0159179*eVToHartree  
GamATot122 :=GamA202v122+GamA211v122+GamA220v122
```

```
GamA201v121:=0.0384013*eVToHartree  
GamA210v121:=0.0203038*eVToHartree  
GamATot121 :=GamA201v121+GamA210v121
```

```
GamA200v120:=0.046625*eVToHartree  
GamATot120 :=GamA200v120
```

```
GamA202v113:=0.0233715*eVToHartree  
GamA211v113:=0.0454153*eVToHartree  
GamATot113 :=GamA202v113+GamA211v113
```

```
GamA201v112:=0.0197002*eVToHartree  
GamA210v112:=0.0199868*eVToHartree  
GamATot112 :=GamA201v112+GamA210v112
```

```
GamA200v111:=0.0123705*eVToHartree  
GamATot111 :=GamA200v111
```

```
GamA201v103:=0.0570107*eVToHartree  
GamATot103 :=GamA201v103
```

```
GamA200v102:=0.0244382*eVToHartree  
GamATot102 :=GamA200v102
```

## X-ray fluorescence

```
( * GamR222v123:=0.000456874*eVToHartree
GamR221v122:=0.000360918*eVToHartree
GamR220v121:=0.00021214*eVToHartree
GamR210v120:=2.08086*^-13*eVToHartree
GamR212v113:=0.000533202*eVToHartree
GamR211v112:=0.000417305*eVToHartree
GamR210v111:=0.000243354*eVToHartree *)
GamR200v110:=1.24592*^-13*eVToHartree
( * GamR202v103:=0.000616842*eVToHartree
GamR201v102:=0.000479494*eVToHartree *)
GamR200v101:=0.000278634*eVToHartree
```

## Double core holes

### Auger decay

```

GamA103v023:=0.0677287*eVToHartree
GamA112v023:=0.115572*eVToHartree
GamA121v023:=0.121624*eVToHartree
GamATot023 :=GamA103v023+GamA112v023+GamA121v023
GamA102v022:=0.0824026*eVToHartree
GamA111v022:=0.0942032*eVToHartree
GamA120v022:=0.0508443*eVToHartree
GamATot022 :=GamA102v022+GamA111v022+GamA120v022
GamA101v021:=0.0990872*eVToHartree
GamA110v021:=0.0565844*eVToHartree
GamATot021 :=GamA101v021+GamA110v021
GamA100v020:=0.115419*eVToHartree
GamATot020 :=GamA100v020
GamA102v013:=0.0685416*eVToHartree
GamA111v013:=0.146191*eVToHartree
GamATot013 :=GamA102v013+GamA111v013
GamA101v012:=0.0554631*eVToHartree
GamA110v012:=0.0597858*eVToHartree
GamATot012 :=GamA101v012+GamA110v012
GamA100v011:=0.0331639*eVToHartree
GamATot011 :=GamA100v011
GamA101v003:=0.173741*eVToHartree
GamATot003 :=GamA101v003
GamA100v002:=0.0704786*eVToHartree
GamATot002 :=GamA100v002

```

## X-ray fluorescence

```
( * GamR122v023:=0.00180059*eVToHartree
GamR121v022:=0.00136778*eVToHartree
GamR120v021:=0.000773245*eVToHartree
GamR110v020:=8.20672*^-13*eVToHartree
GamR112v013:=0.00203422*eVToHartree
GamR111v012:=0.00153921*eVToHartree
GamR110v011:=0.000867332*eVToHartree *)
GamR100v010:=4.65738*^-13*eVToHartree
( * GamR102v003:=0.00232609*eVToHartree
GamR101v002:=0.00175835*eVToHartree *)
GamR100v001:=0.000989389*eVToHartree
```

## Terminate package

```
End [ ]
```

```
EndPackage [ ]
```

## References

- [1] Nina Rohringer, Robin Santra, Phys. Rev. A 76, 033416 (2007), <http://dx.doi.org/10.1103/PhysRevA.76.033416>
- [2] Los Alamos National Laboratory Atomic Physics Codes, <http://aphysics2.lanl.gov/cgi-bin/ION/runlanl08a.pl>
- [3] LCLS Parameter Index for X-RAY-OPTICS / RADIATION-SOURCE, [http://www-ssrl.slac.stanford.edu/htbin/rdbweb/LCLS\\_params\\_DB\\_public](http://www-ssrl.slac.stanford.edu/htbin/rdbweb/LCLS_params_DB_public)
- [4] M. G. Makris, P. Lambropoulos, A. Mihelič, Phys. Rev. Lett. 102, 033002 (2009), <http://dx.doi.org/10.1103/PhysRevLett.102.033002>
- [5] J. L. Campbell, Tibor Papp, Widths of the atomic K–N7 levels, At. Data Nucl. Data Tables 77, 1–56 (2001), <http://dx.doi.org/10.1006/adnd.2000.0848>

- [6] Ryan Coffee, John Bozek, Christian Buth, Marcus Hertlein, Markus Gühr, Nora Berrah, Ali Belkacem, Linda Young, Louis DiMauro, Hamed Merdji, Janos Hajdu, Philip H. Bucksbaum, X-ray multiple ionization of impulsively aligned molecules, Linac Coherent Light Source, Menlo Park, California, USA, 2009, research proposal for the first round of beam time at the Linac Coherent Light Source
- [7] Mau Hsiung Chen, Phys. Rev. A 44, 239-242 (1991), <http://dx.doi.org/10.1103/PhysRevA.44.239>
- [8] Albert C. Thompson et al., X-ray data booklet, Center for X-ray Optics and Advanced Light Source, Lawrence Berkeley National Laboratory, <http://xdb.lbl.gov>
- [9] Christian Buth, Robin Santra, Phys. Rev. A 78, 043409 (2008), <http://dx.doi.org/10.1103/PhysRevA.78.043409>
