# Supplementary material for: Nonlinearity in the sequential absorption of multiple photons
Source: arXiv:1612.07105 ancillary file (2017-09-13)
Supplement: Supplementary file 2 [file linearity_theorem.pdf]

```
Get["NitrogenRateEquations.m", Path -> NotebookDirectory[]]
```

```
HartreeToeV := 27.2113845  
eVToHartree := 1/HartreeToeV  
JouleToHartree := 2.29371269*^17  
MilliJouleToHartree := 1*^-3 * JouleToHartree  
BohrToAngstroem := 0.5291772083  
AngstroemToBohr := 1/BohrToAngstroem  
MicrometerToBohr := 1*^4 * AngstroemToBohr  
BohrToMicrometer := 1/MicrometerToBohr  
t0ToSecond := 24.18884326505*^-18  
t0ToFemtoSecond := 24.18884326505*^-3  
FemtoSecondTot0 := 1/t0ToFemtoSecond  
crossSectionAUtoBarn := 1*^8 * BohrToAngstroem^2  
crossSectionAUtocm2 := crossSectionAUtoBarn * 1*^-24  
crossSectioncm2toAU := 1/crossSectionAUtocm2
```

```
neginfinity := -10 000 * FemtoSecondTot0  
posinfinity := 10 000 * FemtoSecondTot0
```

# Ion yields from a nitrogen atom in LCLS radiation with the linearity theorem, decay equations, and successive approximation

Christian Buth, 13 September 2017

Theoretische Chemie, Physikalisch-Chemisches Institut, Ruprecht-Karls-Universität Heidelberg, Im  
Neuenheimer Feld 229, 69120 Heidelberg, Germany

---

## LCLS x-ray pulse

LCLS FWHM pulse duration:

```
tauX := 2*^-15 / t0ToSecond
```

LCLS photon energy:

```
omegaX := 840 * eVToHartree
```

LCLS around 900 eV (page 12) [1] produces a fluence of  $8^{*11}$  photons / shot /  $\mu\text{m}^2$

```
J0X := 2 * Sqrt[Log[2] / Pi] * 8*^11 / (1*^4 / BohrToAngstroem) ^2 / tauX
```

Gaussian x-ray flux pulse shape (See Eq. (7) in Ref. [2]):

```
jxgaussian[J0Xj_, tX_, t_] :=
  J0Xj * Exp[-4 * Log[2] * (t/tX) ^2] * UnitStep[t + 2 * tX] * UnitStep[2 * tX - t]
flux[t_] := jxgaussian[J0X, tauX, t]
```

```
Plot[{flux[t * FemtoSecondTot0], 1/2 * flux[0] *
  UnitStep[t * FemtoSecondTot0 + tauX/2] * UnitStep[tauX/2 - t * FemtoSecondTot0]},
{t, -3, 3}, PlotStyle -> {{Red, Thick}, {Green, Thick}}, PlotRange -> All]
```

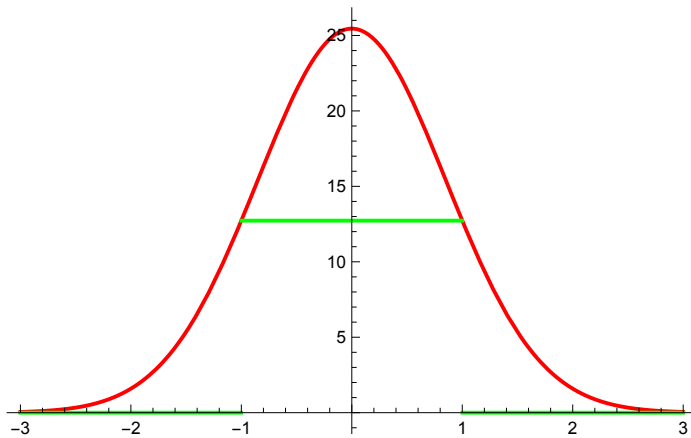

```
fluence[t_] = Integrate[jxgaussian[J0X, tauX, tp],
  {tp, -Infinity, t}, Assumptions -> {t ∈ Reals}] // Simplify
```

|                                                                                                                                                         |                                                                          |
|---------------------------------------------------------------------------------------------------------------------------------------------------------|--------------------------------------------------------------------------|
| <pre>0. 2240.22 1120.11 + 1120.11 Erf[0.0201385 t] 2240.22 + 1120.11 Erf[0.0201385 t] + 1120.11 Erf[(0.0201385 + 2.46626 × 10<sup>-18</sup> i) t]</pre> | <pre>t &lt; -165.365 t &gt; 165.365 -165.365 &lt; t ≤ 165.365 True</pre> |
|---------------------------------------------------------------------------------------------------------------------------------------------------------|--------------------------------------------------------------------------|

```
Plot[fluence[t * FemtoSecondTot0], {t, -3, 3},
  PlotStyle -> {{Red, Thick}, {Green, Thick}}, PlotRange -> All]
```

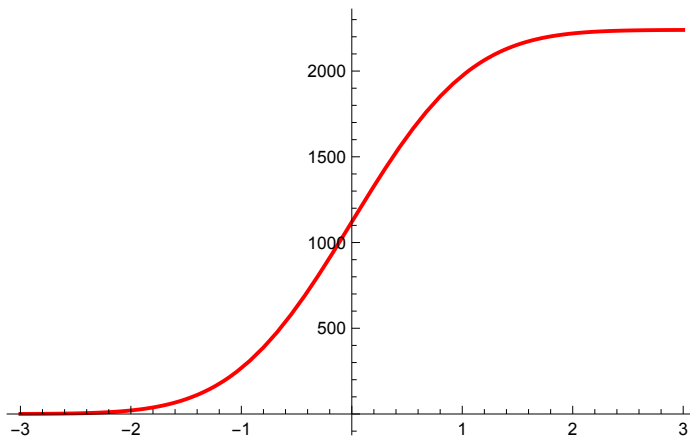

## Cross section matrix

```
idx = <|223 -> 1,
  123 -> 2, 213 -> 3, 222 -> 4,
  023 -> 5, 113 -> 6, 122 -> 7, 203 -> 8, 212 -> 9, 221 -> 10,
  013 -> 11, 022 -> 12, 103 -> 13,
  112 -> 14, 121 -> 15, 202 -> 16, 211 -> 17, 220 -> 18,
  003 -> 19, 012 -> 20, 021 -> 21, 102 -> 22, 111 -> 23,
  120 -> 24, 201 -> 25, 210 -> 26,
  002 -> 27, 011 -> 28, 020 -> 29, 101 -> 30, 110 -> 31, 200 -> 32,
  001 -> 33, 010 -> 34, 100 -> 35,
  000 -> 36|>;
```

```
matSig[en_] := SparseArray[{
  (* No core holes *)
  {idx[200], idx[200]} -> -fsigTot200[en],
  {idx[100], idx[200]} -> fsig100v200[en],
  {idx[201], idx[201]} -> -fsigTot201[en], {idx[200], idx[201]} -> fsig200v201[en],
  {idx[101], idx[201]} -> fsig101v201[en],
  {idx[202], idx[202]} -> -fsigTot202[en], {idx[201], idx[202]} -> fsig201v202[en],
  {idx[102], idx[202]} -> fsig102v202[en],
  {idx[203], idx[203]} -> -fsigTot203[en], {idx[202], idx[203]} -> fsig202v203[en],
  {idx[103], idx[203]} -> fsig103v203[en],
  {idx[210], idx[210]} -> -fsigTot210[en], {idx[200], idx[210]} -> fsig200v210[en],
  {idx[110], idx[210]} -> fsig110v210[en],
  {idx[211], idx[211]} -> -fsigTot211[en], {idx[201], idx[211]} -> fsig201v211[en],
  {idx[210], idx[211]} -> fsig210v211[en],
  {idx[111], idx[211]} -> fsig111v211[en],
  {idx[212], idx[212]} -> -fsigTot212[en], {idx[202], idx[212]} -> fsig202v212[en],
  {idx[211], idx[212]} -> fsig211v212[en],
  {idx[112], idx[212]} -> fsig112v212[en],
```

```

{idx[213], idx[213]} → -fsigTot213[en], {idx[212], idx[213]} → fsig212v213[en],
  {idx[203], idx[213]} → fsig203v213[en],
  {idx[113], idx[213]} → fsig113v213[en],
{idx[220], idx[220]} → -fsigTot220[en], {idx[210], idx[220]} → fsig210v220[en],
  {idx[120], idx[220]} → fsig120v220[en],
{idx[221], idx[221]} → -fsigTot221[en], {idx[220], idx[221]} → fsig220v221[en],
  {idx[121], idx[221]} → fsig121v221[en],
  {idx[211], idx[221]} → fsig211v221[en],
{idx[222], idx[222]} → -fsigTot222[en], {idx[212], idx[222]} → fsig212v222[en],
  {idx[221], idx[222]} → fsig221v222[en],
  {idx[122], idx[222]} → fsig122v222[en],
{idx[223], idx[223]} → -fsigTot223[en], {idx[123], idx[223]} → fsig123v223[en],
  {idx[213], idx[223]} → fsig213v223[en],
  {idx[222], idx[223]} → fsig222v223[en],

(* Single core holes *)
{idx[100], idx[100]} → -fsigTot100[en],
  {idx[000], idx[100]} → fsig000v100[en],
{idx[110], idx[110]} → -fsigTot110[en, True], {idx[100], idx[110]} →
  fsig100v110[en], {idx[010], idx[110]} → fsig010v110[en],
{idx[101], idx[101]} → -fsigTot101[en, True], {idx[100], idx[101]} →
  fsig100v101[en], {idx[001], idx[101]} → fsig001v101[en],
{idx[102], idx[102]} → -fsigTot102[en, True], {idx[101], idx[102]} →
  fsig101v102[en], {idx[002], idx[102]} → fsig002v102[en],
{idx[103], idx[103]} → -fsigTot103[en, True], {idx[102], idx[103]} →
  fsig102v103[en], {idx[003], idx[103]} → fsig003v103[en],
{idx[111], idx[111]} → -fsigTot111[en, True],
  {idx[101], idx[111]} → fsig101v111[en], {idx[110], idx[111]} →
  fsig110v111[en], {idx[011], idx[111]} → fsig011v111[en],
{idx[112], idx[112]} → -fsigTot112[en, True],
  {idx[102], idx[112]} → fsig102v112[en], {idx[111], idx[112]} →
  fsig111v112[en], {idx[012], idx[112]} → fsig012v112[en],
{idx[113], idx[113]} → -fsigTot113[en, True],
  {idx[103], idx[113]} → fsig103v113[en], {idx[112], idx[113]} →
  fsig112v113[en], {idx[013], idx[113]} → fsig013v113[en],
{idx[120], idx[120]} → -fsigTot120[en, True], {idx[110], idx[120]} →
  fsig110v120[en], {idx[020], idx[120]} → fsig020v120[en],
{idx[121], idx[121]} → -fsigTot121[en, True],
  {idx[111], idx[121]} → fsig111v121[en], {idx[120], idx[121]} →
  fsig120v121[en], {idx[021], idx[121]} → fsig021v121[en],
{idx[122], idx[122]} → -fsigTot122[en, True],
  {idx[112], idx[122]} → fsig112v122[en], {idx[121], idx[122]} →
  fsig121v122[en], {idx[022], idx[122]} → fsig022v122[en],
{idx[123], idx[123]} → -fsigTot123[en, True],
  {idx[113], idx[123]} → fsig113v123[en], {idx[122], idx[123]} →
  fsig122v123[en], {idx[023], idx[123]} → fsig023v123[en],

```

```

(* Double core holes *)
{idx[010], idx[010]} → -fsigTot010[en, True],
  {idx[000], idx[010]} → fsig000v010[en],
{idx[020], idx[020]} → -fsigTot020[en, True],
  {idx[010], idx[020]} → fsig010v020[en],
{idx[001], idx[001]} → -fsigTot001[en, True],
  {idx[000], idx[001]} → fsig000v001[en],
{idx[002], idx[002]} → -fsigTot002[en, True],
  {idx[001], idx[002]} → fsig001v002[en],
{idx[003], idx[003]} → -fsigTot003[en, True],
  {idx[002], idx[003]} → fsig002v003[en],
{idx[011], idx[011]} → -fsigTot011[en, True], {idx[010], idx[011]} →
  fsig010v011[en], {idx[001], idx[011]} → fsig001v011[en],
{idx[012], idx[012]} → -fsigTot012[en, True], {idx[011], idx[012]} →
  fsig011v012[en], {idx[002], idx[012]} → fsig002v012[en],
{idx[013], idx[013]} → -fsigTot013[en, True], {idx[003], idx[013]} →
  fsig003v013[en], {idx[012], idx[013]} → fsig012v013[en],
{idx[021], idx[021]} → -fsigTot021[en, True], {idx[011], idx[021]} →
  fsig011v021[en], {idx[020], idx[021]} → fsig020v021[en],
{idx[022], idx[022]} → -fsigTot022[en, True], {idx[012], idx[022]} →
  fsig012v022[en], {idx[021], idx[022]} → fsig021v022[en],
{idx[023], idx[023]} → -fsigTot023[en, True], {idx[013], idx[023]} →
  fsig013v023[en], {idx[022], idx[023]} → fsig022v023[en],

(* Electron-bare state *)
{idx[000], idx[000]} → 0}]

```

```
matSig[840/HartreeToeV] // MatrixForm
```

[illegible]

## Auger decay matrix

```

matAug := SparseArray[{
  (* Single core holes *)
  {idx[123], idx[123]} → -GamATot123, {idx[203], idx[123]} → GamA203v123,
    {idx[212], idx[123]} → GamA212v123, {idx[221], idx[123]} → GamA221v123,
  {idx[122], idx[122]} → -GamATot122, {idx[202], idx[122]} → GamA202v122,
    {idx[211], idx[122]} → GamA211v122, {idx[220], idx[122]} → GamA220v122,
  {idx[121], idx[121]} → -GamATot121, {idx[201], idx[121]} → GamA201v121,
    {idx[210], idx[121]} → GamA210v121,
  {idx[120], idx[120]} → -GamATot120, {idx[200], idx[120]} → GamA200v120,
  {idx[113], idx[113]} → -GamATot113,
    {idx[202], idx[113]} → GamA202v113, {idx[211], idx[113]} → GamA211v113,
  {idx[112], idx[112]} → -GamATot112, {idx[201], idx[112]} → GamA201v112,
    {idx[210], idx[112]} → GamA210v112,
  {idx[111], idx[111]} → -GamATot111, {idx[200], idx[111]} → GamA200v111,
  {idx[103], idx[103]} → -GamATot103, {idx[201], idx[103]} → GamA201v103,
  {idx[102], idx[102]} → -GamATot102, {idx[200], idx[102]} → GamA200v102,

  (* Double core holes *)
  {idx[023], idx[023]} → -GamATot023, {idx[103], idx[023]} → GamA103v023,
    {idx[112], idx[023]} → GamA112v023, {idx[121], idx[023]} → GamA121v023,
  {idx[022], idx[022]} → -GamATot022, {idx[102], idx[022]} → GamA102v022,
    {idx[111], idx[022]} → GamA111v022, {idx[120], idx[022]} → GamA120v022,
  {idx[021], idx[021]} → -GamATot021, {idx[101], idx[021]} → GamA101v021,
    {idx[110], idx[021]} → GamA110v021,
  {idx[020], idx[020]} → -GamATot020, {idx[100], idx[020]} → GamA100v020,
  {idx[013], idx[013]} → -GamATot013,
    {idx[102], idx[013]} → GamA102v013, {idx[111], idx[013]} → GamA111v013,
  {idx[012], idx[012]} → -GamATot012, {idx[101], idx[012]} → GamA101v012,
    {idx[110], idx[012]} → GamA110v012,
  {idx[011], idx[011]} → -GamATot011, {idx[100], idx[011]} → GamA100v011,
  {idx[003], idx[003]} → -GamATot003, {idx[101], idx[003]} → GamA101v003,
  {idx[002], idx[002]} → -GamATot002, {idx[100], idx[002]} → GamA100v002,

  (* Electron-bare state *)
  {idx[000], idx[000]} → 0}]

```

```
matAug // MatrixForm
```

[illegible]



## Radiative decay matrix

```

matRad := SparseArray[{
  (* No core holes *)
    {idx[213], idx[213]} → -GamR222v213, {idx[222], idx[213]} → GamR222v213,
    {idx[212], idx[212]} → -GamR221v212, {idx[221], idx[212]} → GamR221v212,
    {idx[211], idx[211]} → -GamR220v211, {idx[220], idx[211]} → GamR220v211,
    {idx[203], idx[203]} → -GamR212v203, {idx[212], idx[203]} → GamR212v203,
    {idx[202], idx[202]} → -GamR211v202, {idx[211], idx[202]} → GamR211v202,
    {idx[201], idx[201]} → -GamR210v201, {idx[210], idx[201]} → GamR210v201,

    (* Single core holes *)
    {idx[110], idx[110]} → -GamR200v110, {idx[200], idx[110]} → GamR200v110,
    {idx[101], idx[101]} → -GamR200v101, {idx[200], idx[101]} → GamR200v101,

    (* Double core holes *)
    {idx[010], idx[010]} → -GamR100v010, {idx[100], idx[010]} → GamR100v010,
    {idx[001], idx[001]} → -GamR100v001, {idx[100], idx[001]} → GamR100v001,

    (* Electron-bare state *)
    {idx[000], idx[000]} → 0}]

```

```
matRad // MatrixForm
```

# Commutators

```
matSig[omegaX].matAug - matAug.matSig[omegaX] // MatrixForm
```

[illegible]

```
matSig[omegaX].matRad - matRad.matSig[omegaX] // MatrixForm
```

[illegible]

```
matSig[omegaX].(matAug + matRad) - (matAug + matRad).matSig[omegaX] // MatrixForm
```

$$\begin{pmatrix} 0. & 0. & 0. & 0. & 0. & 0. \\ 0.0000149965 & 0. & 0. & 0. & 0. & 0. \\ 6.94082 \times 10^{-12} & 0. & 0. & 0. & 0. & 0. \\ -6.94082 \times 10^{-12} & 0. & -3.27273 \times 10^{-12} & 0. & 0. & 0. \\ 0. & 0.0000192503 & 0. & 0. & 0. & 0. \\ 0. & -2.7916 \times 10^{-7} & 0.0000104002 & 0. & 0. & 0. \\ 0. & -2.86648 \times 10^{-8} & 1.50609 \times 10^{-10} & 0.0000119651 & 0. & 0. \\ -3.87999 \times 10^{-6} & -1.17265 \times 10^{-6} & 7.14224 \times 10^{-12} & 0. & 0. & 0. \\ -5.73436 \times 10^{-6} & -1.88332 \times 10^{-6} & -4.00583 \times 10^{-12} & 2.92508 \times 10^{-12} & 0. & 0. \\ -5.38219 \times 10^{-6} & -1.90404 \times 10^{-6} & 2.42604 \times 10^{-13} & -2.92508 \times 10^{-12} & 0. & 0. \\ 0. & 0. & 0. & 0. & -1.15021 \times 10^{-6} & 0. \\ 0. & 0. & 0. & 0. & -2.22161 \times 10^{-7} & 0. \\ 0. & -2.5171 \times 10^{-6} & 0. & 0. & -5.2285 \times 10^{-6} & -6. \\ 0. & -5.15638 \times 10^{-6} & 0. & 0. & -9.58426 \times 10^{-6} & -5. \\ 0. & -6.05881 \times 10^{-6} & 0. & 0. & -0.0000107822 & 0. \\ 0. & -8.03165 \times 10^{-8} & -3.53368 \times 10^{-6} & -4.6991 \times 10^{-6} & 0. & -1. \\ 0. & -1.58353 \times 10^{-7} & -6.86662 \times 10^{-6} & -4.86098 \times 10^{-6} & 0. & -2. \\ 0. & -1.14809 \times 10^{-8} & 0. & -2.40503 \times 10^{-6} & 0. & 0. \\ 0. & 0. & 0. & 0. & 6.13584 \times 10^{-6} & 0. \\ 0. & 0. & 0. & 0. & 0.0000105386 & 0. \\ 0. & 0. & 0. & 0. & 0.0000111793 & 0. \\ 0. & 0. & 0. & 0. & -2.78236 \times 10^{-7} & -2. \\ 0. & 0. & 0. & 0. & -5.5088 \times 10^{-7} & -6. \\ 0. & 0. & 0. & 0. & -5.72157 \times 10^{-8} & 0. \\ 0. & 0. & 0. & 0. & 0. & -1. \\ 0. & 0. & 0. & 0. & 0. & -1. \\ 0. & 0. & 0. & 0. & 0. & 0. \\ 0. & 0. & 0. & 0. & 0. & 0. \\ 0. & 0. & 0. & 0. & 0. & 0. \\ 0. & 0. & 0. & 0. & 0. & 0. \\ 0. & 0. & 0. & 0. & 0. & 0. \\ 0. & 0. & 0. & 0. & 0. & 0. \\ 0. & 0. & 0. & 0. & 0. & 0. \\ 0. & 0. & 0. & 0. & 0. & 0. \\ 0. & 0. & 0. & 0. & 0. & 0. \\ 0. & 0. & 0. & 0. & 0. & 0. \\ 0. & 0. & 0. & 0. & 0. & 0. \\ 0. & 0. & 0. & 0. & 0. & 0. \end{pmatrix}$$

## Linearity theorem

```
sol = solveNitrogenRateEquations[
  omegaX, flux, neginfinity, posinfinity, 1/1000, True];
```

```
inivec := Join[{1}, Table[0, 35]]
```

```
linGround[t_] := MatrixExp[matSig[omegaX] * fluence[t], inivec][[idx[223]]]
```

```
linSingly[t_] := Total[MatrixExp[matSig[omegaX] * fluence[t], inivec][[
  {idx[123], idx[213], idx[222]}]]]
```

```
linDoubly[t_] := Total[MatrixExp[matSig[omegaX] * fluence[t], inivec][[
  {idx[212], idx[203], idx[221], idx[113], idx[122], idx[023]}]]]
```

```
linTriply[t_] :=
  Total[MatrixExp[matSig[omegaX] * fluence[t], inivec][[{idx[202], idx[211],
    idx[220], idx[103], idx[112], idx[121], idx[013], idx[022]}]]]
```

```
linQuadruply[t_] :=
  Total[MatrixExp[matSig[omegaX] * fluence[t], inivec][[{idx[201], idx[210],
    idx[102], idx[111], idx[120], idx[003], idx[012], idx[021]}]]]
```

```
linQuintuply[t_] := Total[MatrixExp[matSig[omegaX] * fluence[t], inivec][[
  {idx[200], idx[101], idx[110], idx[011], idx[020], idx[002]}]]]
```

```
linSextuply[t_] := Total[MatrixExp[matSig[omegaX] * fluence[t], inivec][[
  {idx[100], idx[010], idx[001]}]]]
```

```
linSeptuply[t_] := MatrixExp[matSig[omegaX] * fluence[t], inivec][[idx[000]]]
```

```
Plot[{solGround[sol, t1 * FemtoSecondTot0], linGround[t1 * FemtoSecondTot0]},
  {t1, -5, 5}, PlotStyle -> {{Black, Thick}, {Red, Thick, Dashed}},
  PlotRange -> {-0.01, 1.2}, AxesLabel -> {"t [fs]", "W0(t)"},
  LabelStyle -> {FontFamily -> "Helvetica", FontSize -> 14},
  AxesStyle -> Arrowheads[Automatic]]
```

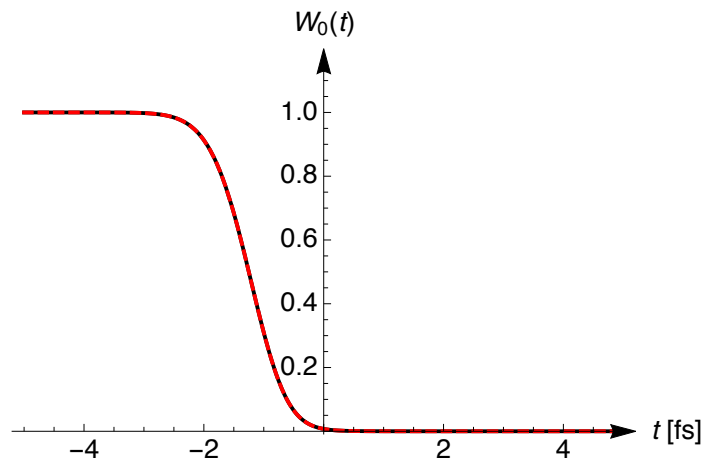

```
Plot[{solSingly[sol, t1 * FemtoSecondTot0], linSingly[t1 * FemtoSecondTot0]},
  {t1, -4, 4}, PlotStyle -> {{Black, Thick}, {Red, Thick, Dashed}},
  PlotRange -> {-0.01, 0.55}, AxesLabel -> {"t [fs]", " $W_1(t)$ "},
  LabelStyle -> {FontFamily -> "Helvetica", FontSize -> 14},
  AxesStyle -> Arrowheads[Automatic]]
```

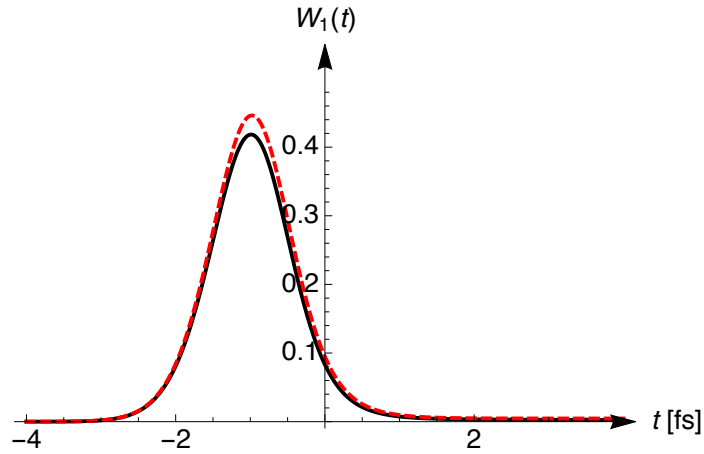

```
Plot[{solDoubly[sol, t1 * FemtoSecondTot0], linDoubly[t1 * FemtoSecondTot0]},
  {t1, -5, 12}, PlotRange -> {-0.01, 0.7},
  PlotStyle -> {{Black, Thick}, {Red, Thick, Dashed}},
  AxesLabel -> {"t [fs]", " $W_2(t)$ "},
  LabelStyle -> {FontFamily -> "Helvetica", FontSize -> 14},
  AxesStyle -> Arrowheads[Automatic]]
```

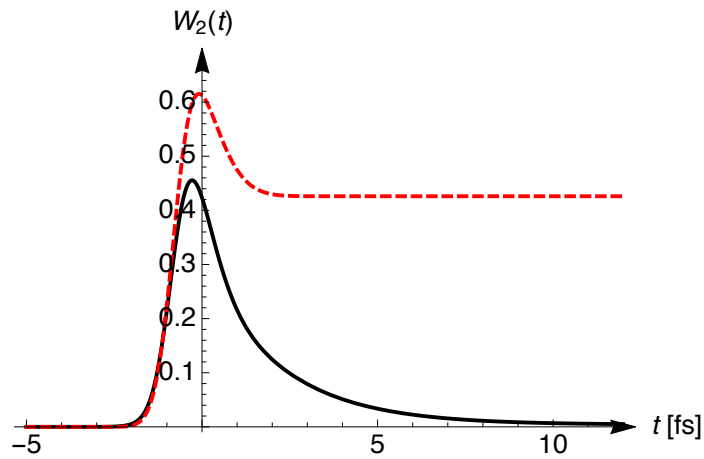

```

Plot[{solTriply[sol, t1 * FemtoSecondTot0], linTriply[t1 * FemtoSecondTot0]},
  {t1, -20, 80}, PlotRange → {-0.01, 0.5},
  PlotStyle → {{Black, Thick}, {Red, Thick, Dashed}},
  AxesLabel → {"t [fs]", " $W_3(t)$ "},
  LabelStyle → {FontFamily → "Helvetica", FontSize → 14},
  AxesStyle → Arrowheads[Automatic]]

```

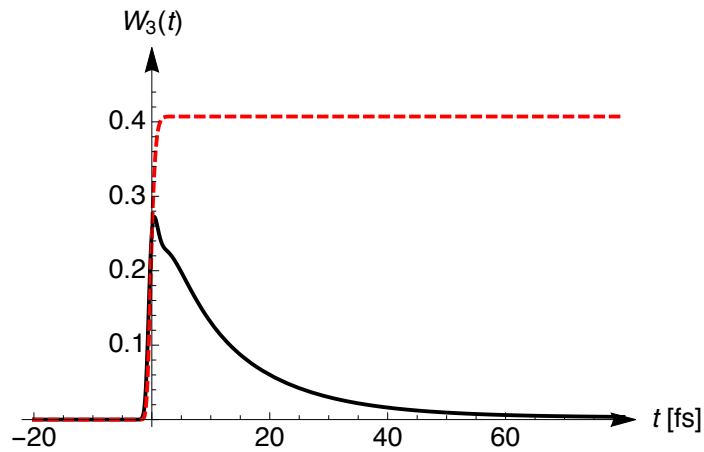

```

Plot[{solQuadruply[sol, t1 * FemtoSecondTot0],
  linQuadruply[t1 * FemtoSecondTot0]}, {t1, -20, 200},
  PlotRange → {-0.01, 0.35}, PlotStyle → {{Black, Thick}, {Red, Thick, Dashed}},
  AxesLabel → {"t [fs]", " $W_4(t)$ "},
  LabelStyle → {FontFamily → "Helvetica", FontSize → 14},
  AxesStyle → Arrowheads[Automatic]]

```

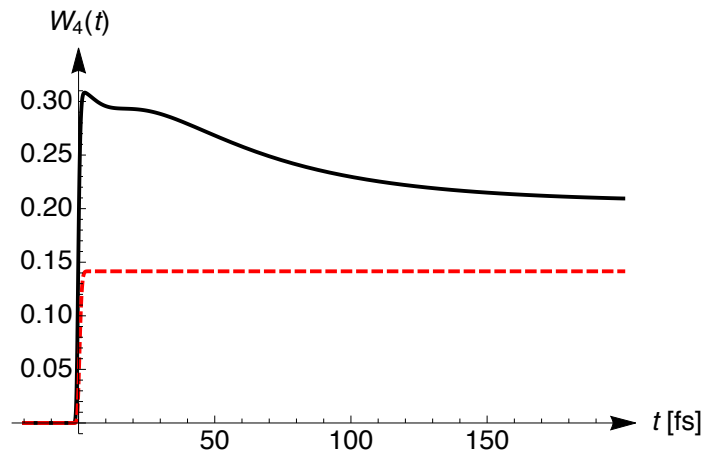



```

Plot[{solQuintuply[sol, t1 * FemtoSecondTot0],
  linQuintuply[t1 * FemtoSecondTot0]}, {t1, -20, 200},
PlotRange → {-0.01, 0.55}, PlotStyle → {{Black, Thick}, {Red, Thick, Dashed}},
AxesLabel → {"t [fs]", " $W_5(t)$ "},
LabelStyle → {FontFamily → "Helvetica", FontSize → 14},
AxesStyle → Arrowheads[Automatic]]

```

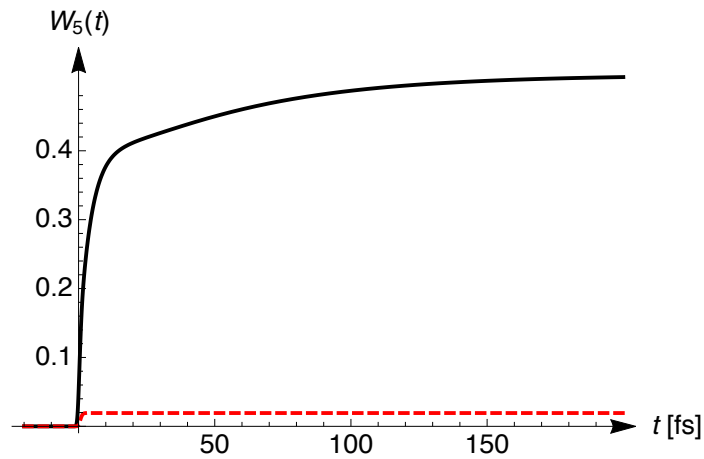

```

Plot[{solSextuply[sol, t1 * FemtoSecondTot0], linSextuply[t1 * FemtoSecondTot0]},
{t1, -20, 100}, PlotRange → {-0.01, 0.3},
PlotStyle → {{Black, Thick}, {Red, Thick, Dashed}},
AxesLabel → {"t [fs]", " $W_6(t)$ "},
LabelStyle → {FontFamily → "Helvetica", FontSize → 14},
AxesStyle → Arrowheads[Automatic]]

```

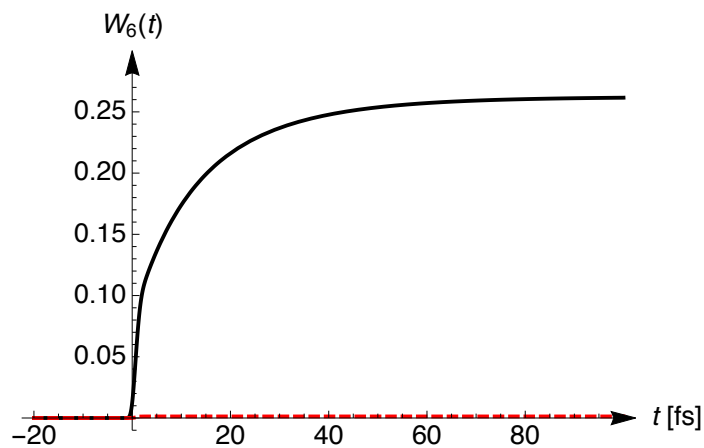

```
Plot[{solSeptuply[sol, t1 * FemtoSecondTot0], linSeptuply[t1 * FemtoSecondTot0]},
  {t1, -10, 10}, PlotRange → {-0.001, 0.02},
  PlotStyle → {{Black, Thick}, {Red, Thick, Dashed}},
  AxesLabel → {"t [fs]", " $W_7(t)$ "},
  LabelStyle → {FontFamily → "Helvetica", FontSize → 14},
  AxesStyle → Arrowheads[Automatic]]
```

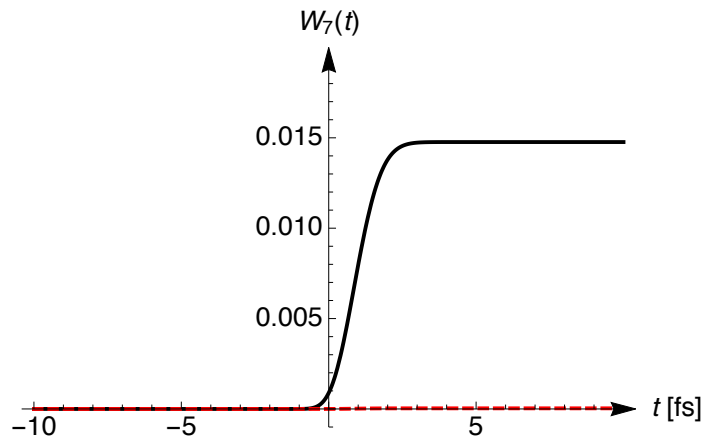

## Decay equations

```
matGam = matAug + matRad;
```

```
decGround[t_] := UnitStep[t - tauX] * MatrixExp[matGam * If[t > tauX, t - tauX, 0],
  MatrixExp[matSig[omegaX] * fluence[posinfinity], inivec]][[idx[223]]]
```

```
decSingly[t_] :=
  Total[UnitStep[t - tauX] * MatrixExp[matGam * If[t > tauX, t - tauX, 0],
    MatrixExp[matSig[omegaX] * fluence[posinfinity], inivec]][[
      {idx[123], idx[213], idx[222]}]]]
```

```
decDoubly[t_] :=
  Total[UnitStep[t - tauX] * MatrixExp[matGam * If[t > tauX, t - tauX, 0],
    MatrixExp[matSig[omegaX] * fluence[posinfinity], inivec]][[
      {idx[212], idx[203], idx[221], idx[113], idx[122], idx[023]}]]]
```

```
decTriply[t_] :=
  Total[UnitStep[t - tauX] * MatrixExp[matGam * If[t > tauX, t - tauX, 0],
    MatrixExp[matSig[omegaX] * fluence[posinfinity], inivec]][{idx[202],
    idx[211], idx[220], idx[103], idx[112], idx[121], idx[013], idx[022]}]]]
```

```
decQuadruply[t_] :=
  Total[UnitStep[t - tauX] * MatrixExp[matGam * If[t > tauX, t - tauX, 0],
    MatrixExp[matSig[omegaX] * fluence[posinfinity], inivec]][{idx[201],
    idx[210], idx[102], idx[111], idx[120], idx[003], idx[012], idx[021]}]]]
```

```
decQuintuply[t_] :=
  Total[UnitStep[t - tauX] * MatrixExp[matGam * If[t > tauX, t - tauX, 0],
    MatrixExp[matSig[omegaX] * fluence[posinfinity], inivec]][{
    {idx[200], idx[101], idx[110], idx[011], idx[020], idx[002]}]]]
```

```
decSextuply[t_] :=
  Total[UnitStep[t - tauX] * MatrixExp[matGam * If[t > tauX, t - tauX, 0],
    MatrixExp[matSig[omegaX] * fluence[posinfinity], inivec]][{
    {idx[100], idx[010], idx[001]}]]]
```

```
decSeptuply[t_] := UnitStep[t - tauX] * MatrixExp[matGam * If[t > tauX, t - tauX, 0],
  MatrixExp[matSig[omegaX] * fluence[posinfinity], inivec]][{idx[000]}]
```

## LCLS 2 fs pulse

```
tauX := 2 * FemtoSecondTot0
```

```
fluence[t_] = Integrate[jxgaussian[J0X, tauX, tp],
  {tp, -Infinity, t}, Assumptions → {t ∈ Reals}] // Simplify
```

|                                                                                                           |                             |
|-----------------------------------------------------------------------------------------------------------|-----------------------------|
| 0.                                                                                                        | $t < -165.365$              |
| 2240.22                                                                                                   | $t > 165.365$               |
| $1120.11 + 1120.11 \operatorname{Erf}[0.0201385 t]$                                                       | $-165.365 < t \leq 165.365$ |
| $2240.22 + 1120.11 \operatorname{Erf}\left[\left(0.0201385 + 2.46626 \times 10^{-18} i\right) t\right] +$ | True                        |
| $1120.11 \operatorname{Erf}[0.0201385 t]$                                                                 |                             |

```
sol = solveNitrogenRateEquations[
  omegaX, flux, neginfinity, posinfinity, 1/1000, True];
```

```

Plot[{solGround[sol, t1 * FemtoSecondTot0],
  linGround[t1 * FemtoSecondTot0], decGround[t1 * FemtoSecondTot0]}, {t1, -5, 5},
PlotStyle → {{Black, Thick}, {Red, Thick, Dashed}, {Green, Thick, DotDashed}},
PlotRange → {-0.01, 1.1}, AxesLabel → {"t [fs]", " $W_0(t)$ "},
LabelStyle → {FontFamily → "Helvetica", FontSize → 14},
AxesStyle → Arrowheads[Automatic]]

```

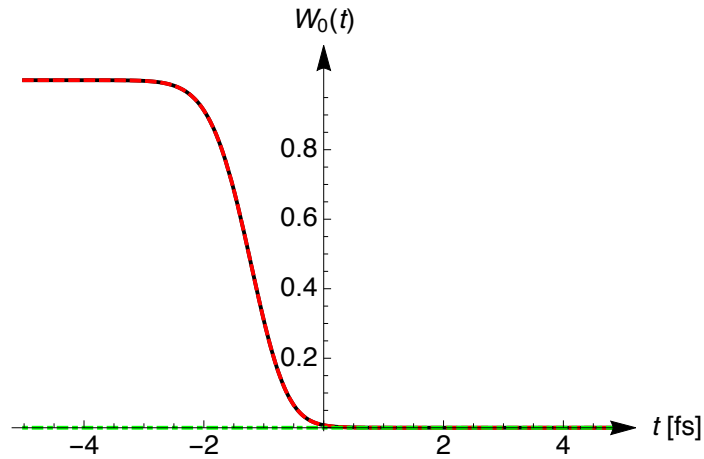

```

Plot[{solSingly[sol, t1 * FemtoSecondTot0], linSingly[t1 * FemtoSecondTot0],
  decSingly[t1 * FemtoSecondTot0]}, {t1, -4, 4}, PlotRange → {-0.01, 0.55},
PlotStyle → {{Black, Thick}, {Red, Thick, Dashed}, {Green, Thick, DotDashed}},
AxesLabel → {"t [fs]", " $W_1(t)$ "},
LabelStyle → {FontFamily → "Helvetica", FontSize → 14},
AxesStyle → Arrowheads[Automatic]]

```

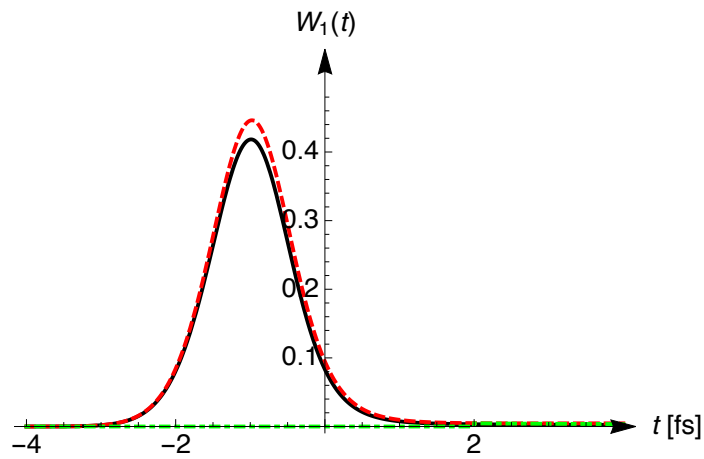

```

Plot[{solDoubly[sol, t1 * FemtoSecondTot0], linDoubly[t1 * FemtoSecondTot0],
  decDoubly[t1 * FemtoSecondTot0]}, {t1, -4, 10}, PlotRange → {-0.01, 0.7},
PlotStyle → {{Black, Thick}, {Red, Thick, Dashed}, {Green, Thick, DotDashed}},
AxesLabel → {"t [fs]", " $W_2(t)$ "},
LabelStyle → {FontFamily → "Helvetica", FontSize → 14},
AxesStyle → Arrowheads[Automatic]]

```

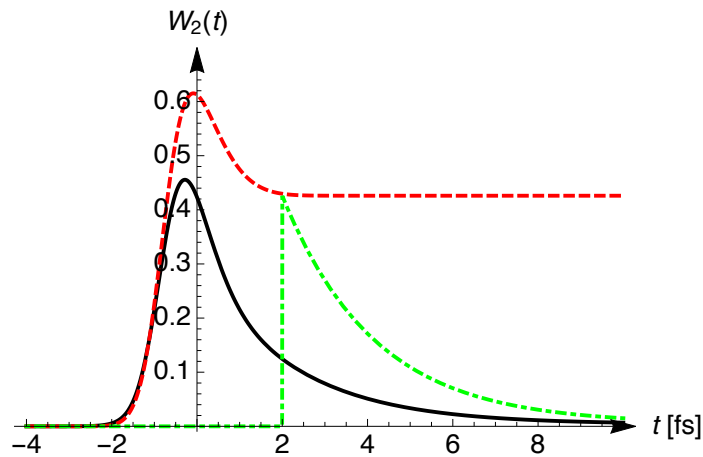

```

Plot[{solTriply[sol, t1 * FemtoSecondTot0], linTriply[t1 * FemtoSecondTot0],
  decTriply[t1 * FemtoSecondTot0]}, {t1, -20, 100}, PlotRange → {-0.01, 0.55},
PlotStyle → {{Black, Thick}, {Red, Thick, Dashed}, {Green, Thick, DotDashed}},
AxesLabel → {"t [fs]", " $W_3(t)$ "},
LabelStyle → {FontFamily → "Helvetica", FontSize → 14},
AxesStyle → Arrowheads[Automatic]]

```

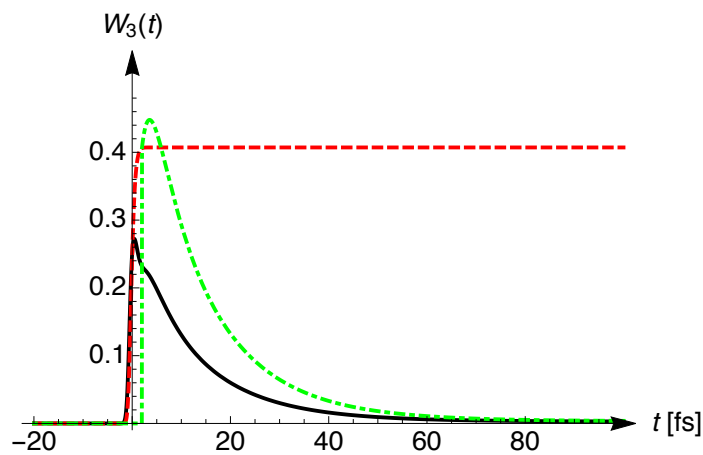

```

Plot[{solQuadruply[sol, t1 * FemtoSecondTot0], linQuadruply[t1 * FemtoSecondTot0],
  decQuadruply[t1 * FemtoSecondTot0]}, {t1, -20, 100}, PlotRange -> All,
PlotStyle -> {{Black, Thick}, {Red, Thick, Dashed}, {Green, Thick, DotDashed}},
AxesLabel -> {"t [fs]", " $W_4(t)$ "},
LabelStyle -> {FontFamily -> "Helvetica", FontSize -> 14},
AxesStyle -> Arrowheads[Automatic]]

```

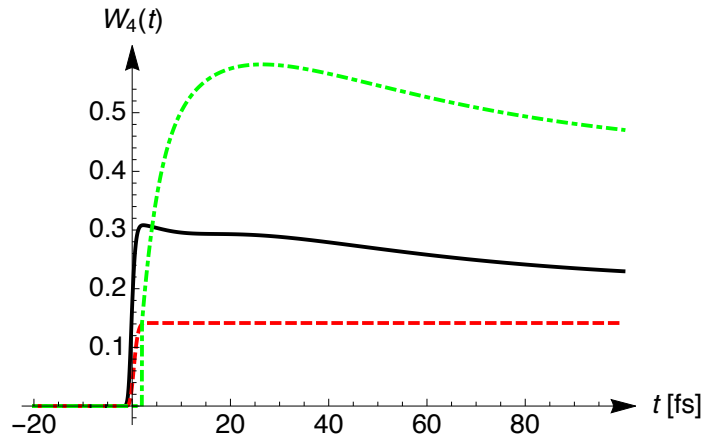

```

Plot[{solQuintuply[sol, t1 * FemtoSecondTot0], linQuintuply[t1 * FemtoSecondTot0],
  decQuintuply[t1 * FemtoSecondTot0]}, {t1, -20, 200}, PlotRange -> All,
PlotStyle -> {{Black, Thick}, {Red, Thick, Dashed}, {Green, Thick, DotDashed}},
AxesLabel -> {"t [fs]", " $W_5(t)$ "},
LabelStyle -> {FontFamily -> "Helvetica", FontSize -> 14},
AxesStyle -> Arrowheads[Automatic]]

```

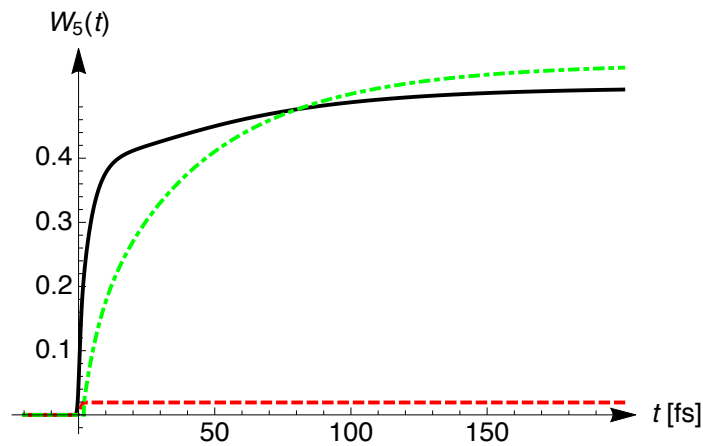

```
Plot[{solSextuply[sol, t1 * FemtoSecondTot0], linSextuply[t1 * FemtoSecondTot0],
  decSextuply[t1 * FemtoSecondTot0]}, {t1, -20, 100}, PlotRange → All,
PlotStyle → {{Black, Thick}, {Red, Thick, Dashed}, {Green, Thick, DotDashed}},
AxesLabel → {"t [fs]", " $W_6(t)$ "},
LabelStyle → {FontFamily → "Helvetica", FontSize → 14},
AxesStyle → Arrowheads[Automatic]]
```

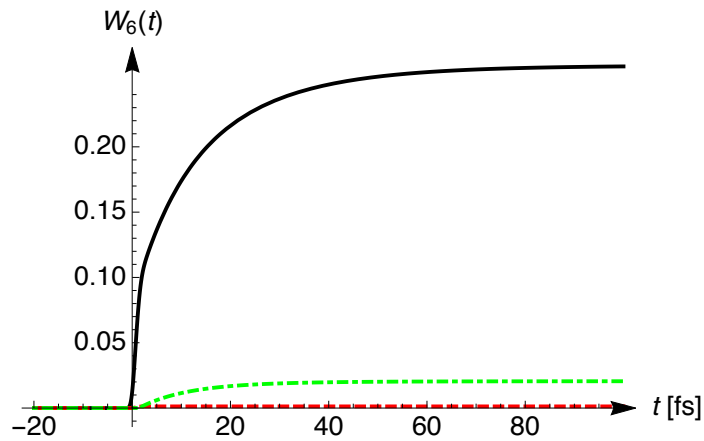

```
Plot[{solSeptuply[sol, t1 * FemtoSecondTot0], linSeptuply[t1 * FemtoSecondTot0],
  decSeptuply[t1 * FemtoSecondTot0]}, {t1, -10, 10}, PlotRange → All,
PlotStyle → {{Black, Thick}, {Red, Thick, Dashed}, {Green, Thick, DotDashed}},
AxesLabel → {"t [fs]", " $W_7(t)$ "},
LabelStyle → {FontFamily → "Helvetica", FontSize → 14},
AxesStyle → Arrowheads[Automatic]]
```

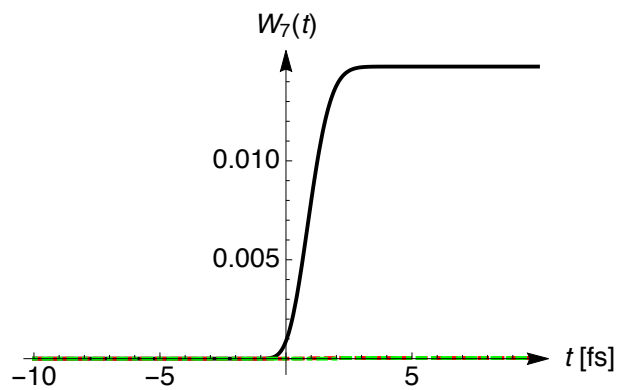

## LCLS 200 as pulse

```

tauX := 200*^-18/t0ToSecond

fluence[t_] = Integrate[jxgaussian[J0X, tauX, tp],
  {tp, -Infinity, t}, Assumptions -> {t ∈ Reals}] // Simplify

```

$$\begin{cases} 0. & t < -16.5365 \\ 2240.22 & t > 16.5365 \\ 1120.11 + 1120.11 \operatorname{Erf}[0.201385 t] & -16.5365 < t \leq 16.5365 \\ 2240.22 + 1120.11 \operatorname{Erf}[0.201385 t] + \\ \quad (1120.11 - 2.5099 \times 10^{-29} i) & \text{True} \\ \quad \operatorname{Erf}[(0.201385 + 2.46626 \times 10^{-17} i) t] & \end{cases}$$

```

sol = solveNitrogenRateEquations[
  omegaX, flux, neginfinity, posinfinity, 1/2000, True];

Plot[{solGround[sol, t1 * FemtoSecondTot0],
  linGround[t1 * FemtoSecondTot0], decGround[t1 * FemtoSecondTot0]}, {t1, -5, 5},
PlotStyle -> {{Black, Thick}, {Red, Thick, Dashed}, {Green, Thick, DotDashed}},
PlotRange -> All, AxesLabel -> {"t [fs]", "W_0(t)"},
LabelStyle -> {FontFamily -> "Helvetica", FontSize -> 14},
AxesStyle -> Arrowheads[Automatic]]

```

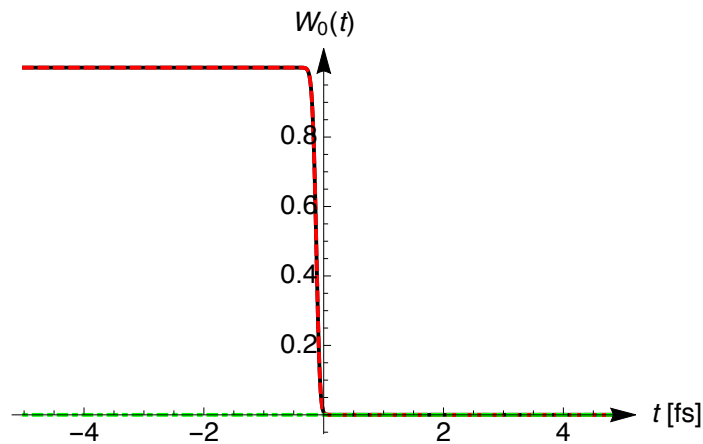



```

Plot[{solSingly[sol, t1 * FemtoSecondTot0], linSingly[t1 * FemtoSecondTot0],
  decSingly[t1 * FemtoSecondTot0]}, {t1, -0.5, 0.5}, PlotRange → All,
PlotStyle → {{Black, Thick}, {Red, Thick, Dashed}, {Green, Thick, DotDashed}},
AxesLabel → {"t [fs]", " $W_1(t)$ "},
LabelStyle → {FontFamily → "Helvetica", FontSize → 14},
AxesStyle → Arrowheads[Automatic]]

```

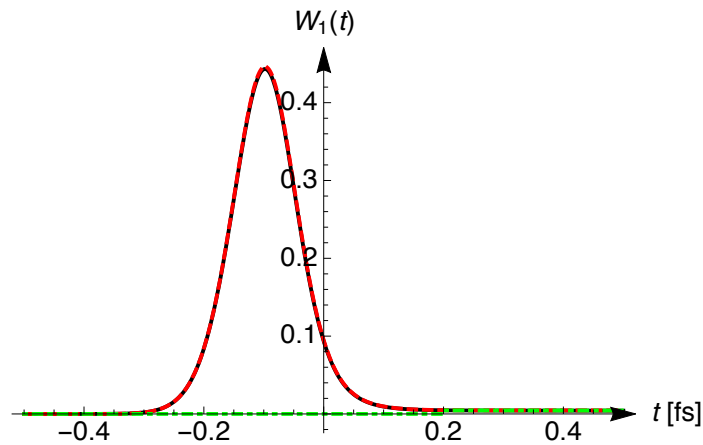

```

Plot[{solDoubly[sol, t1 * FemtoSecondTot0], linDoubly[t1 * FemtoSecondTot0],
  decDoubly[t1 * FemtoSecondTot0]}, {t1, -4, 10}, PlotRange → {-0.01, 0.7},
PlotStyle → {{Black, Thick}, {Red, Thick, Dashed}, {Green, Thick, DotDashed}},
AxesLabel → {"t [fs]", " $W_2(t)$ "},
LabelStyle → {FontFamily → "Helvetica", FontSize → 14},
AxesStyle → Arrowheads[Automatic]]

```

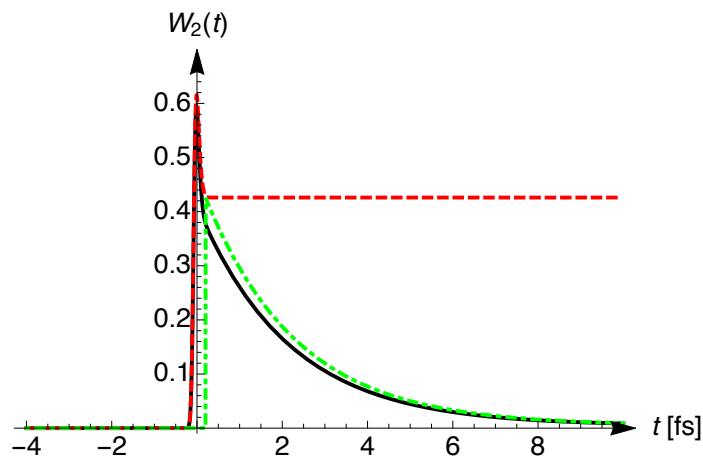

```

Plot[{solTriply[sol, t1 * FemtoSecondTot0], linTriply[t1 * FemtoSecondTot0],
  decTriply[t1 * FemtoSecondTot0]}, {t1, -20, 100}, PlotRange → All,
PlotStyle → {{Black, Thick}, {Red, Thick, Dashed}, {Green, Thick, DotDashed}},
AxesLabel → {"t [fs]", " $W_3(t)$ "},
LabelStyle → {FontFamily → "Helvetica", FontSize → 14},
AxesStyle → Arrowheads[Automatic]]

```

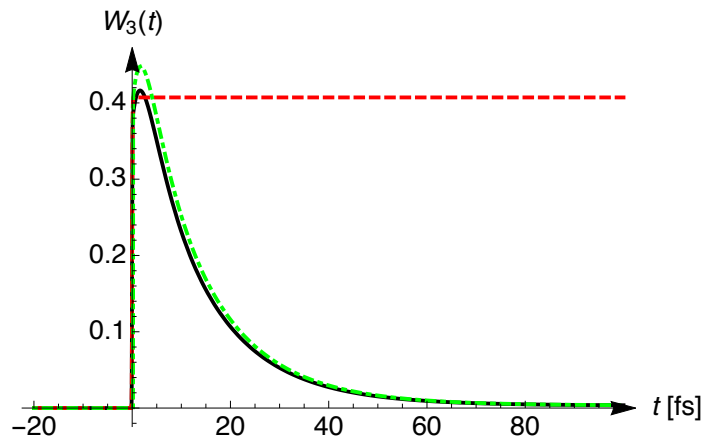

```

Plot[{solQuadruply[sol, t1 * FemtoSecondTot0], linQuadruply[t1 * FemtoSecondTot0],
  decQuadruply[t1 * FemtoSecondTot0]}, {t1, -20, 100}, PlotRange → All,
PlotStyle → {{Black, Thick}, {Red, Thick, Dashed}, {Green, Thick, DotDashed}},
AxesLabel → {"t [fs]", " $W_4(t)$ "},
LabelStyle → {FontFamily → "Helvetica", FontSize → 14},
AxesStyle → Arrowheads[Automatic]]

```

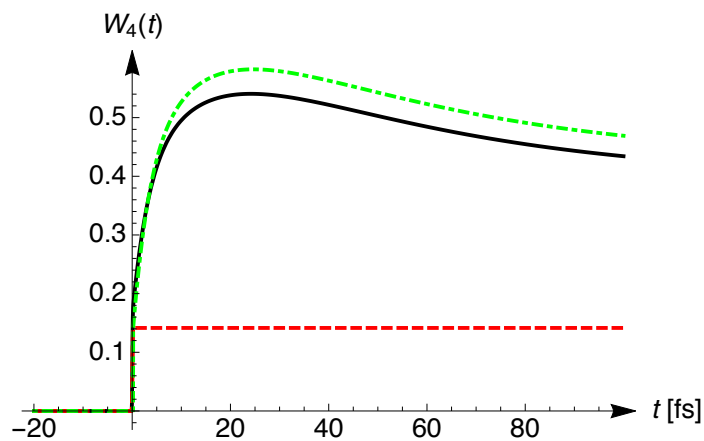

```
Plot[{solQuintuply[sol, t1 * FemtoSecondTot0], linQuintuply[t1 * FemtoSecondTot0],
  decQuintuply[t1 * FemtoSecondTot0]}, {t1, -20, 200}, PlotRange -> All,
  PlotStyle -> {{Black, Thick}, {Red, Thick, Dashed}, {Green, Thick, DotDashed}},
  AxesLabel -> {"t [fs]", " $W_5(t)$ "},
  LabelStyle -> {FontFamily -> "Helvetica", FontSize -> 14},
  AxesStyle -> Arrowheads[Automatic]]
```

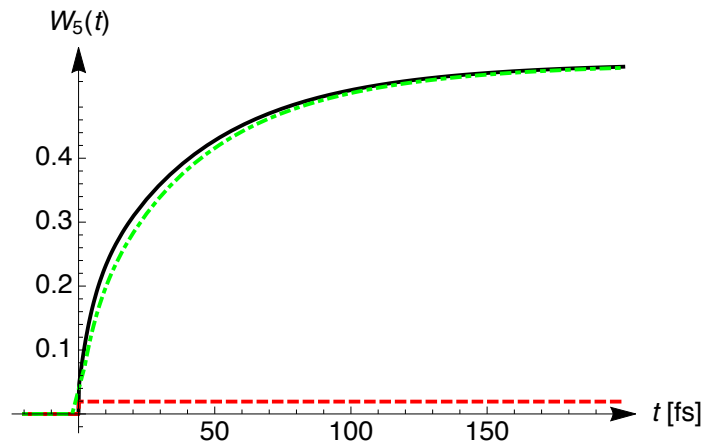

```
Plot[{solSextuply[sol, t1 * FemtoSecondTot0], linSextuply[t1 * FemtoSecondTot0],
  decSextuply[t1 * FemtoSecondTot0]}, {t1, -20, 100}, PlotRange -> All,
  PlotStyle -> {{Black, Thick}, {Red, Thick, Dashed}, {Green, Thick, DotDashed}},
  AxesLabel -> {"t [fs]", " $W_6(t)$ "},
  LabelStyle -> {FontFamily -> "Helvetica", FontSize -> 14},
  AxesStyle -> Arrowheads[Automatic]]
```

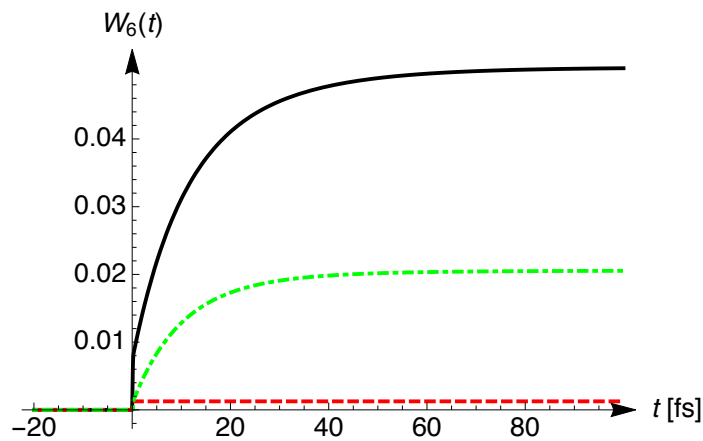

```
Plot[{solSeptuply[sol, t1 * FemtoSecondTot0], linSeptuply[t1 * FemtoSecondTot0],
  decSeptuply[t1 * FemtoSecondTot0]}, {t1, -3, 10}, PlotRange → {0, 0.00058},
  PlotStyle → {{Black, Thick}, {Red, Thick, Dashed}, {Green, Thick, DotDashed}},
  AxesLabel → {"t [fs]", " $W_7(t)$ "},
  LabelStyle → {FontFamily → "Helvetica", FontSize → 14}]
```

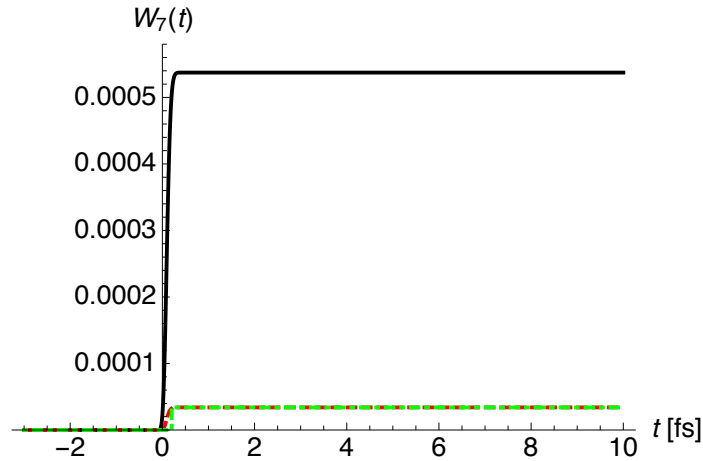

## LCLS 50 as pulse

```
tauX := 50*^-18 / t0ToSecond
```

```
fluence[t_] = Integrate[jxgaussian[J0X, tauX, tp],
  {tp, -Infinity, t}, Assumptions → {t ∈ Reals}] // Simplify
```

|                                                                                                                                                                                                                                                   |                                                                        |
|---------------------------------------------------------------------------------------------------------------------------------------------------------------------------------------------------------------------------------------------------|------------------------------------------------------------------------|
| $\begin{cases} 0. \\ 2240.22 \\ 1120.11 + 1120.11 \operatorname{Erf}[0.805541 t] \\ 2240.22 + 1120.11 \operatorname{Erf}[0.805541 t] + \\ 1120.11 \operatorname{Erf}\left[\left(0.805541 + 9.86504 \times 10^{-17} i\right) t\right] \end{cases}$ | $t < -4.13414$<br>$t > 4.13414$<br>$-4.13414 < t \leq 4.13414$<br>True |
|---------------------------------------------------------------------------------------------------------------------------------------------------------------------------------------------------------------------------------------------------|------------------------------------------------------------------------|

```
sol = solveNitrogenRateEquations[
  omegaX, flux, neginfinity, posinfinity, 1/10000, True];
```

```

Plot[{solGround[sol, t1 * FemtoSecondTot0], linGround[t1 * FemtoSecondTot0],
  decGround[t1 * FemtoSecondTot0]}, {t1, -0.1, 0.1},
PlotStyle → {{Black, Thick}, {Red, Thick, Dashed}, {Green, Thick, DotDashed}},
PlotRange → {-0.01, 1.1}, AxesLabel → {"t [fs]", " $W_0(t)$ "},
LabelStyle → {FontFamily → "Helvetica", FontSize → 14},
AxesStyle → Arrowheads[Automatic]]

```

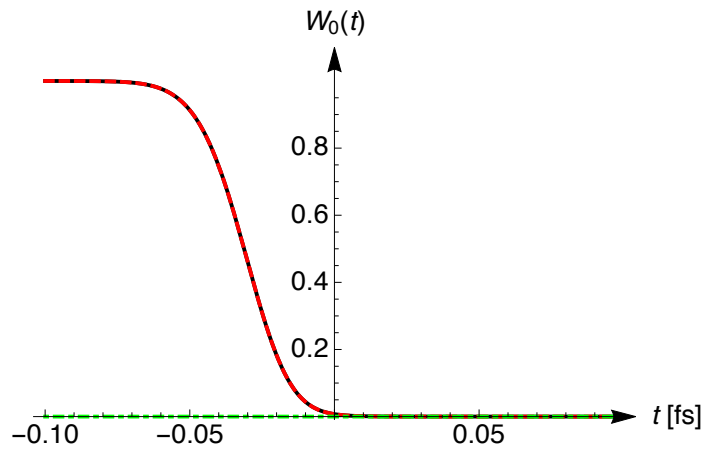

```

Plot[{solSingly[sol, t1 * FemtoSecondTot0], linSingly[t1 * FemtoSecondTot0],
  decSingly[t1 * FemtoSecondTot0]}, {t1, -0.1, 0.1}, PlotRange → All,
PlotStyle → {{Black, Thick}, {Red, Thick, Dashed}, {Green, Thick, DotDashed}},
AxesLabel → {"t [fs]", " $W_1(t)$ "},
LabelStyle → {FontFamily → "Helvetica", FontSize → 14},
AxesStyle → Arrowheads[Automatic]]

```

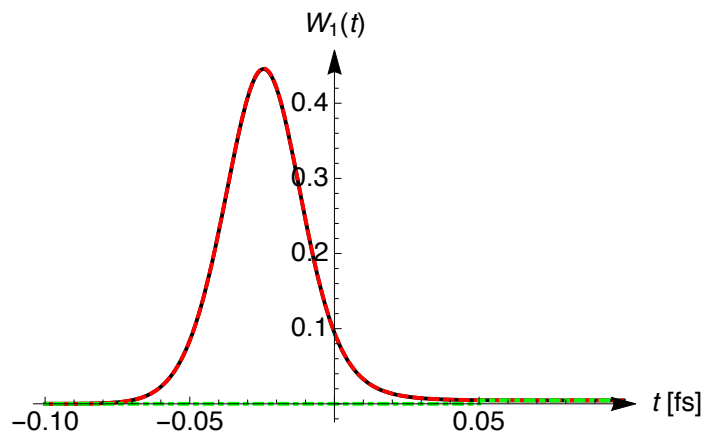

```

Plot[{solDoubly[sol, t1 * FemtoSecondTot0], linDoubly[t1 * FemtoSecondTot0],
  decDoubly[t1 * FemtoSecondTot0]}, {t1, -2, 10}, PlotRange → All,
PlotStyle → {{Black, Thick}, {Red, Thick, Dashed}, {Green, Thick, DotDashed}},
AxesLabel → {"t [fs]", " $W_2(t)$ "},
LabelStyle → {FontFamily → "Helvetica", FontSize → 14},
AxesStyle → Arrowheads[Automatic]]

```

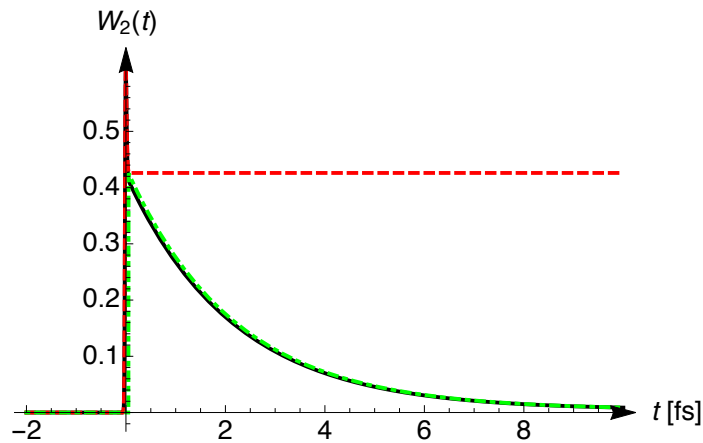

```

Plot[{solTriply[sol, t1 * FemtoSecondTot0], linTriply[t1 * FemtoSecondTot0],
  decTriply[t1 * FemtoSecondTot0]}, {t1, -20, 100}, PlotRange → All,
PlotStyle → {{Black, Thick}, {Red, Thick, Dashed}, {Green, Thick, DotDashed}},
AxesLabel → {"t [fs]", " $W_3(t)$ "},
LabelStyle → {FontFamily → "Helvetica", FontSize → 14},
AxesStyle → Arrowheads[Automatic]]

```

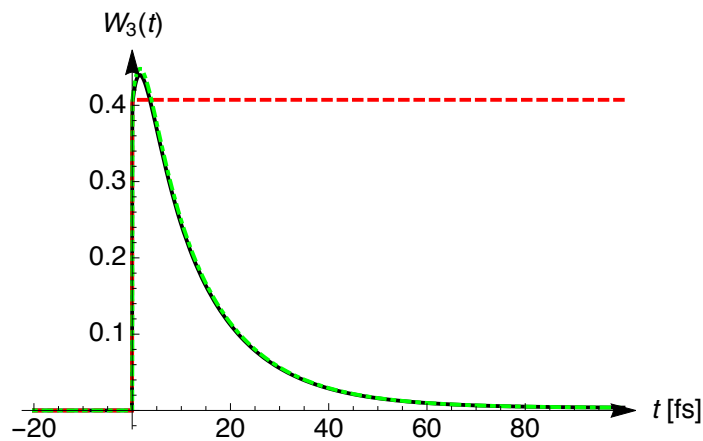

```
Plot[{solQuadruply[sol, t1 * FemtoSecondTot0], linQuadruply[t1 * FemtoSecondTot0],
  decQuadruply[t1 * FemtoSecondTot0]}, {t1, -20, 100}, PlotRange → All,
PlotStyle → {{Black, Thick}, {Red, Thick, Dashed}, {Green, Thick, DotDashed}},
AxesLabel → {"t [fs]", " $W_4(t)$ "},
LabelStyle → {FontFamily → "Helvetica", FontSize → 14},
AxesStyle → Arrowheads[Automatic]]
```

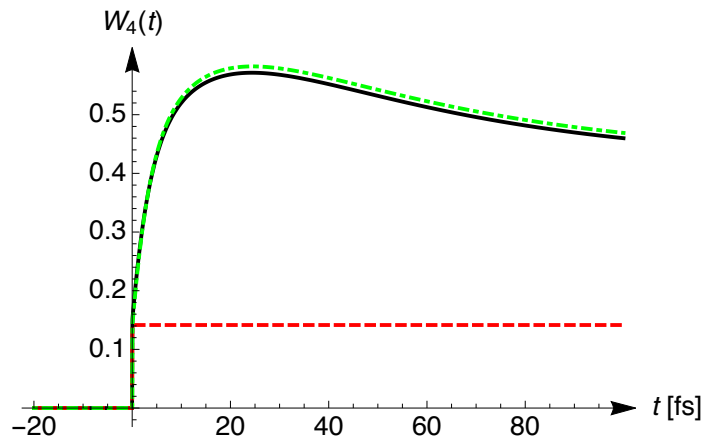

```
Plot[{solQuintuply[sol, t1 * FemtoSecondTot0], linQuintuply[t1 * FemtoSecondTot0],
  decQuintuply[t1 * FemtoSecondTot0]}, {t1, -20, 200}, PlotRange → All,
PlotStyle → {{Black, Thick}, {Red, Thick, Dashed}, {Green, Thick, DotDashed}},
AxesLabel → {"t [fs]", " $W_5(t)$ "},
LabelStyle → {FontFamily → "Helvetica", FontSize → 14},
AxesStyle → Arrowheads[Automatic]]
```

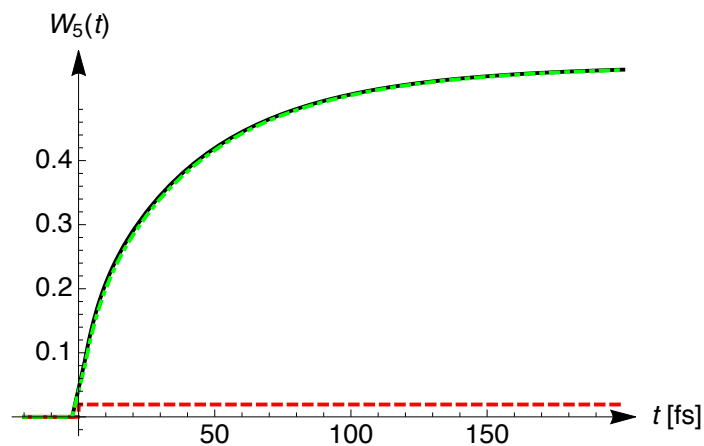

```
Plot[{solSextuply[sol, t1 * FemtoSecondTot0], linSextuply[t1 * FemtoSecondTot0],
  decSextuply[t1 * FemtoSecondTot0]}, {t1, -20, 100}, PlotRange → All,
PlotStyle → {{Black, Thick}, {Red, Thick, Dashed}, {Green, Thick, DotDashed}},
AxesLabel → {"t [fs]", " $W_6(t)$ "},
LabelStyle → {FontFamily → "Helvetica", FontSize → 14},
AxesStyle → Arrowheads[Automatic]]
```

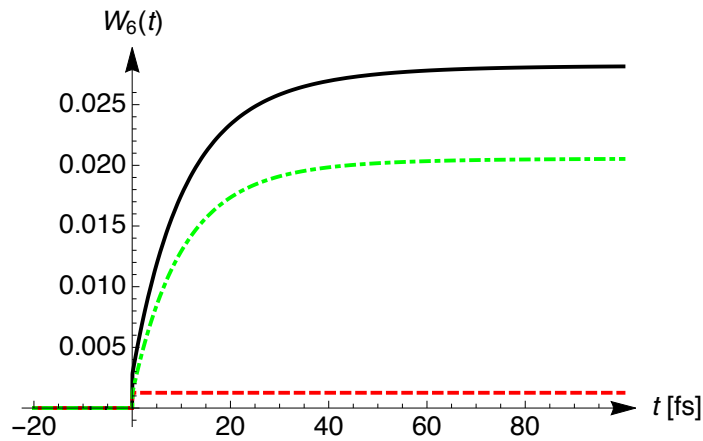

```
Plot[{solSeptuply[sol, t1 * FemtoSecondTot0], linSeptuply[t1 * FemtoSecondTot0],
  decSeptuply[t1 * FemtoSecondTot0]}, {t1, -2, 10}, PlotRange → All,
PlotStyle → {{Black, Thick}, {Red, Thick, Dashed}, {Green, Thick, DotDashed}},
AxesLabel → {"t [fs]", " $W_7(t)$ "},
LabelStyle → {FontFamily → "Helvetica", FontSize → 14}]
```

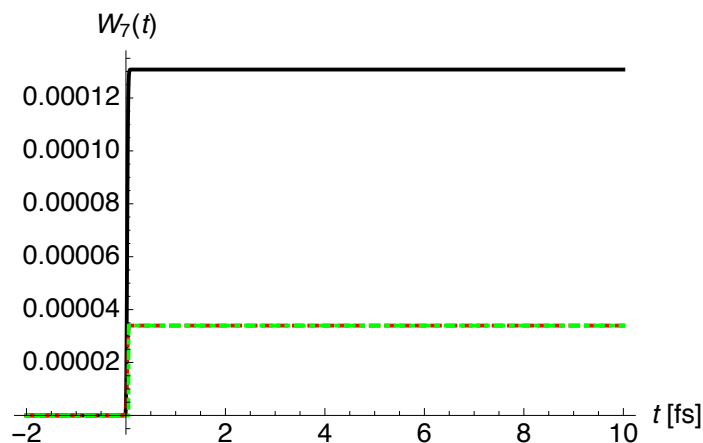

## Successive approximation

```
tauX := 2 * FemtoSecondTot0
```



```

fluence[t_] = Integrate[jxgaussian[J0X, tauX, tp],
  {tp, -Infinity, t}, Assumptions → {t ∈ Reals}] // Simplify
{
  0.
  2240.22
  1120.11 + 1120.11 Erf[0.0201385 t]
  2240.22 + 1120.11 Erf[(0.0201385 + 2.46626 × 10-18 i) t] +
  1120.11 Erf[0.0201385 t]
}
t < -165.365
t > 165.365
-165.365 < t ≤ 165.365
True

sol = solveNitrogenRateEquations[
  omegaX, flux, neginfinity, posinfinity, 1/1000, True];

zerothOrderIntegral[t_] := inivec

successiveKernel[prevIntegral_, t_] := MatrixExp[-matSig[omegaX] * fluence[t],
  matGam.MatrixExp[matSig[omegaX] * fluence[t], prevIntegral[t]]];

successiveApproximation[prevIntegral_] := Module[
  {appKernelVal, appKernelPos, kernelInterpolation, successiveIntegral, i, j},
  appKernelVal = Table[Re[successiveKernel[prevIntegral, i * FemtoSecondTot0]],
    {i, -20, 20, 0.5}];
  appKernelPos = Table[i * FemtoSecondTot0, {i, -20, 20, 0.5}];
  kernelInterpolation = Table[
    ListInterpolation[appKernelVal[;;, j]], {appKernelPos}], {j, 1, 36}]
]

successiveIntegral[kernelInterpolation_, t_] :=
  NIntegrate[Through[kernelInterpolation[tp]], {tp, -20 * FemtoSecondTot0, t}]

kernelInterpolationsFirst = successiveApproximation[zerothOrderIntegral];
successiveIntegralFirst[t_] := successiveIntegral[kernelInterpolationsFirst, t]

kernelInterpolationsSecond = successiveApproximation[successiveIntegralFirst];
successiveIntegralSecond[t_] :=
  successiveIntegral[kernelInterpolationsSecond, t]

kernelInterpolationsThird = successiveApproximation[successiveIntegralSecond];
successiveIntegralThird[t_] := successiveIntegral[kernelInterpolationsThird, t]

kernelInterpolationsFourth = successiveApproximation[successiveIntegralThird];
successiveIntegralFourth[t_] :=
  successiveIntegral[kernelInterpolationsFourth, t]

kernelInterpolationsFifth = successiveApproximation[successiveIntegralFourth];
successiveIntegralFifth[t_] := successiveIntegral[kernelInterpolationsFifth, t]

kernelInterpolationsSixth = successiveApproximation[successiveIntegralFifth];
successiveIntegralSixth[t_] := successiveIntegral[kernelInterpolationsSixth, t]

```

```
kernelInterpolationsSeventh = successiveApproximation[successiveIntegralSixth];
successiveIntegralSeventh[t_] :=
  successiveIntegral[kernelInterpolationsSeventh, t]
```

```
kernelInterpolationsEighth =
  successiveApproximation[successiveIntegralSeventh];
successiveIntegralEighth[t_] :=
  successiveIntegral[kernelInterpolationsEighth, t]
```

```
successiveProbabilityFirst[t_] :=
  MatrixExp[matSig[omegaX] * fluence[t], inivec + successiveIntegralFirst[t]]
```

```
successiveProbabilityEighth[t_] := MatrixExp[matSig[omegaX] * fluence[t],
  inivec + successiveIntegralFirst[t] + successiveIntegralSecond[t] +
  successiveIntegralThird[t] + successiveIntegralFourth[t] +
  successiveIntegralFifth[t] + successiveIntegralSixth[t] +
  successiveIntegralSeventh[t] + successiveIntegralEighth[t]]
```

```
nonGround[successiveProbability_, t_] := successiveProbability[t][[idx[223]]]
```

```
nonSingly[successiveProbability_, t_] :=
  Total[successiveProbability[t][[{idx[213], idx[222], idx[123]}]]]
```

```
nonDoubly[successiveProbability_, t_] := Total[successiveProbability[t][[
  {idx[212], idx[203], idx[221], idx[113], idx[122], idx[023]}]]]
```

```
nonTriply[successiveProbability_, t_] :=
  Total[successiveProbability[t][[{idx[202], idx[211],
  idx[220], idx[103], idx[112], idx[121], idx[013], idx[022]}]]]
```

```
nonQuadruply[successiveProbability_, t_] :=
  Total[successiveProbability[t][[{idx[201], idx[210],
  idx[102], idx[111], idx[120], idx[003], idx[012], idx[021]}]]]
```

```
nonQuintuply[successiveProbability_, t_] := Total[successiveProbability[t][[
  {idx[200], idx[101], idx[110], idx[011], idx[020], idx[002]}]]]
```

```
nonSextuply[successiveProbability_, t_] :=
  Total[successiveProbability[t][[{idx[100], idx[010], idx[001]}]]]
```

```
nonSeptuply[successiveProbability_, t_] :=
  successiveProbability[t][[idx[000]]]
```

```
Plot[{solGround[sol, t1 * FemtoSecondTot0], linGround[t1 * FemtoSecondTot0],
  nonGround[successiveProbabilityFirst, t1 * FemtoSecondTot0],
  nonGround[successiveProbabilityEighth, t1 * FemtoSecondTot0]}, {t1, -4, 4},
PlotStyle -> {{Black, Thick}, {Red, Thick, Dashed}, {Green, Thick, DotDashed},
  {Blue, Thick, Dotted}}, PlotRange -> All, AxesLabel -> {"t [fs]", " $W_0(t)$ "},
LabelStyle -> {FontFamily -> "Helvetica", FontSize -> 14},
AxesStyle -> Arrowheads[Automatic]]
```

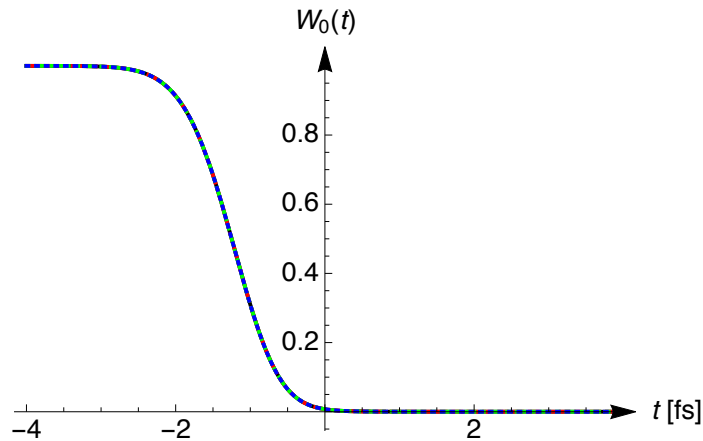

```
Plot[{solSingly[sol, t1 * FemtoSecondTot0], linSingly[t1 * FemtoSecondTot0],
  nonSingly[successiveProbabilityFirst, t1 * FemtoSecondTot0],
  nonSingly[successiveProbabilityEighth, t1 * FemtoSecondTot0]}, {t1, -4, 4},
PlotStyle -> {{Black, Thick}, {Red, Thick, Dashed},
  {Green, Thick, DotDashed}, {Blue, Thick, Dotted}},
PlotRange -> {0, 0.55}, AxesLabel -> {"t [fs]", " $W_1(t)$ "},
LabelStyle -> {FontFamily -> "Helvetica", FontSize -> 14},
AxesStyle -> Arrowheads[Automatic]]
```

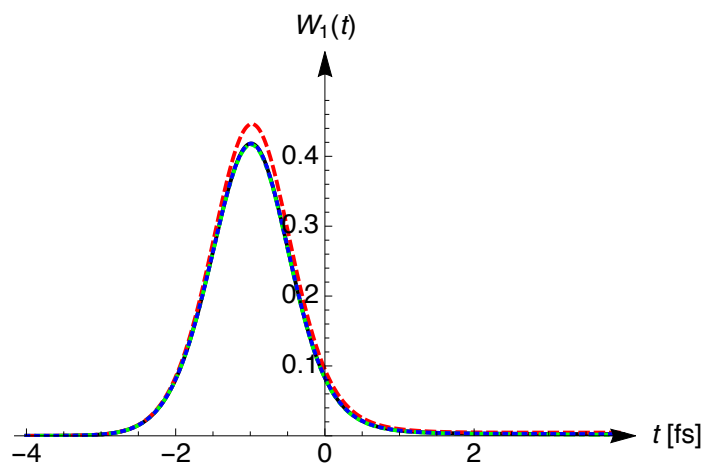

```

Plot[{solDoubly[sol, t1 * FemtoSecondTot0], linDoubly[t1 * FemtoSecondTot0],
  nonDoubly[successiveProbabilityFirst, t1 * FemtoSecondTot0],
  nonDoubly[successiveProbabilityEighth, t1 * FemtoSecondTot0]},
{t1, -4, 8}, PlotStyle -> {{Black, Thick}, {Red, Thick, Dashed},
  {Green, Thick, DotDashed}, {Blue, Thick, Dotted}},
PlotRange -> {0, 0.75}, AxesLabel -> {"t [fs]", " $W_2(t)$ "},
LabelStyle -> {FontFamily -> "Helvetica", FontSize -> 14},
AxesStyle -> Arrowheads[Automatic]]

```

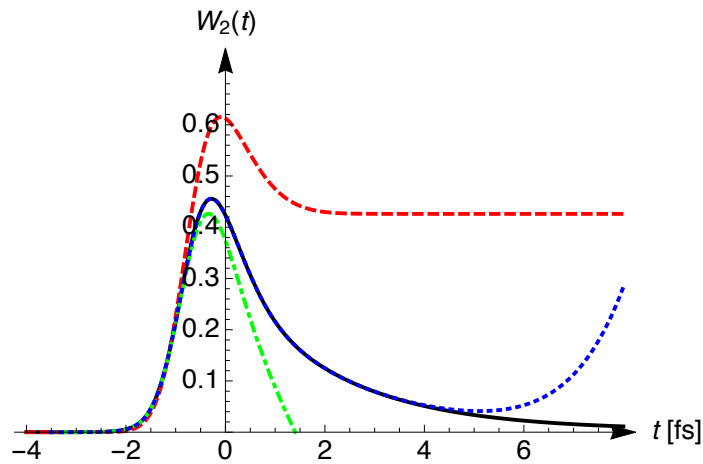

```

Plot[{solTriply[sol, t1 * FemtoSecondTot0], linTriply[t1 * FemtoSecondTot0],
  nonTriply[successiveProbabilityFirst, t1 * FemtoSecondTot0],
  nonTriply[successiveProbabilityEighth, t1 * FemtoSecondTot0]}, {t1, -4, 7},
PlotStyle -> {{Black, Thick}, {Red, Thick, Dashed}, {Green, Thick, DotDashed},
  {Blue, Thick, Dotted}}, PlotRange -> All, AxesLabel -> {"t [fs]", " $W_3(t)$ "},
LabelStyle -> {FontFamily -> "Helvetica", FontSize -> 14},
AxesStyle -> Arrowheads[Automatic]]

```

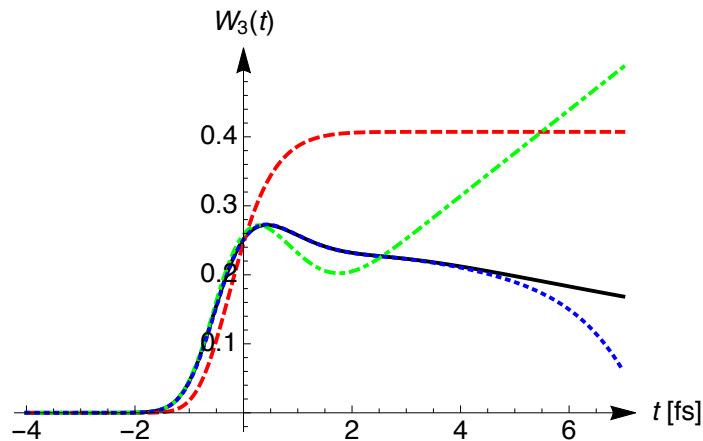

```
Plot[{solQuadruply[sol, t1 * FemtoSecondTot0], linQuadruply[t1 * FemtoSecondTot0],
  nonQuadruply[successiveProbabilityFirst, t1 * FemtoSecondTot0],
  nonQuadruply[successiveProbabilityEighth, t1 * FemtoSecondTot0]},
{t1, -4, 10}, PlotStyle -> {{Black, Thick}, {Red, Thick, Dashed},
  {Green, Thick, DotDashed}, {Blue, Thick, Dotted}},
PlotRange -> {0, 0.4}, AxesLabel -> {"t [fs]", " $W_4(t)$ "},
LabelStyle -> {FontFamily -> "Helvetica", FontSize -> 14},
AxesStyle -> Arrowheads[Automatic]]
```

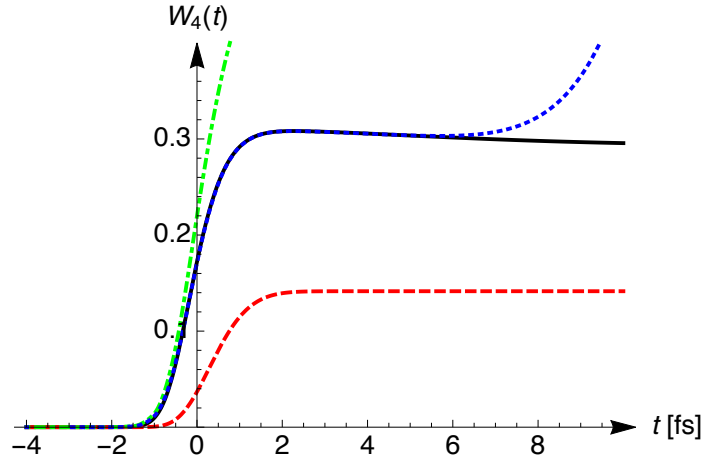

```
Plot[{solQuintuply[sol, t1 * FemtoSecondTot0], linQuintuply[t1 * FemtoSecondTot0],
  nonQuintuply[successiveProbabilityFirst, t1 * FemtoSecondTot0],
  nonQuintuply[successiveProbabilityEighth, t1 * FemtoSecondTot0]},
{t1, -4, 10}, PlotStyle -> {{Black, Thick}, {Red, Thick, Dashed},
  {Green, Thick, DotDashed}, {Blue, Thick, Dotted}},
PlotRange -> {0, 0.5}, AxesLabel -> {"t [fs]", " $W_5(t)$ "},
LabelStyle -> {FontFamily -> "Helvetica", FontSize -> 14},
AxesStyle -> Arrowheads[Automatic]]
```

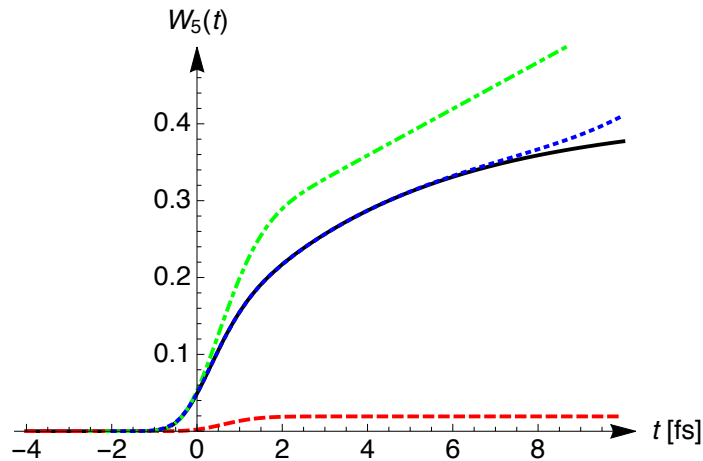

```

Plot[{solSextuply[sol, t1 * FemtoSecondTot0], linSextuply[t1 * FemtoSecondTot0],
  nonSextuply[successiveProbabilityFirst, t1 * FemtoSecondTot0],
  nonSextuply[successiveProbabilityEighth, t1 * FemtoSecondTot0]},
{t1, -4, 20}, PlotStyle -> {{Black, Thick}, {Red, Thick, Dashed},
  {Green, Thick, DotDashed}, {Blue, Thick, Dotted}},
PlotRange -> {0, 0.3}, AxesLabel -> {"t [fs]", " $W_6(t)$ "},
LabelStyle -> {FontFamily -> "Helvetica", FontSize -> 14},
AxesStyle -> Arrowheads[Automatic]]

```

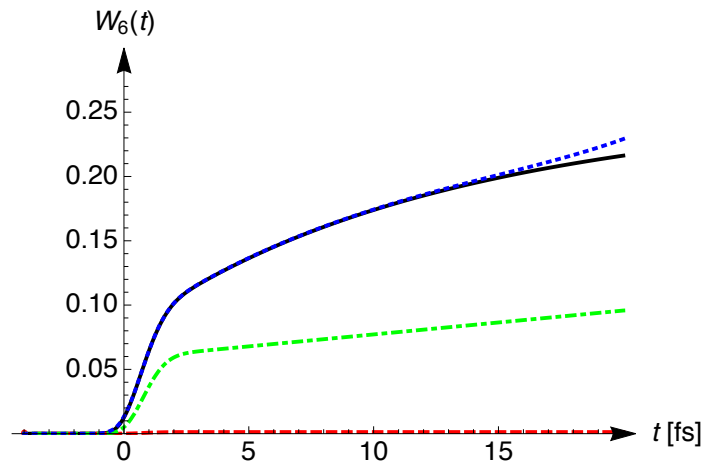

```
Plot[{solSeptuply[sol, t1 * FemtoSecondTot0], linSeptuply[t1 * FemtoSecondTot0],
  nonSeptuply[successiveProbabilityFirst, t1 * FemtoSecondTot0],
  nonSeptuply[successiveProbabilityEighth, t1 * FemtoSecondTot0]},
{t1, -4, 20}, PlotStyle -> {{Black, Thick}, {Red, Thick, Dashed},
  {Green, Thick, DotDashed}, {Blue, Thick, Dotted}},
PlotRange -> {0, 0.02}, AxesLabel -> {"t [fs]", " $W_7(t)$ "},
LabelStyle -> {FontFamily -> "Helvetica", FontSize -> 14},
AxesStyle -> Arrowheads[Automatic]]
```

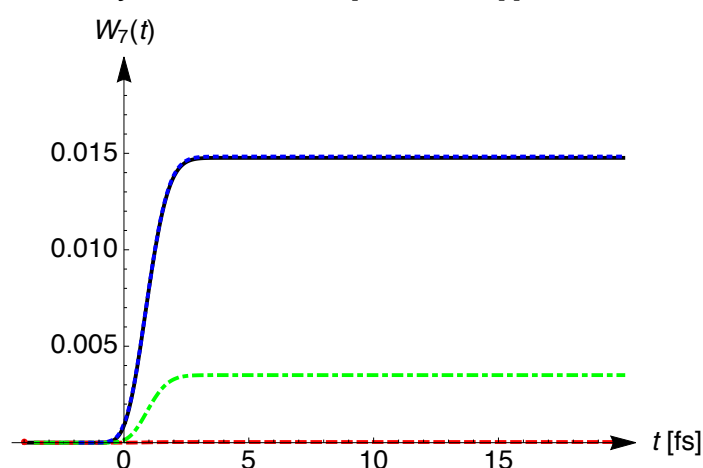

## References

- [1] Ryan Coffee, John Bozek, Christian Buth, Marcus Hertlein, Markus Gühr, Nora Berrah, Ali Belkacem, Linda Young, Lou DiMauro, Hamed Merdji, Hajdu, Philip H. Bucksbaum, *Xray multiple ionization of impulsively aligned molecules*, Linac Coherent Light Source, Menlo Park, California, USA, 2009, research proposal for beamtime at Linac Coherent Light Source.
- [2] Christian Buth, Ji-Cai Liu, Mau Hsiung Chen, James P. Cryan, Li Fang, James M. Glownia, Matthias Hoener, Ryan N. Coffee, Nora Berrah, *Ultrafast absorption of intense x rays by nitrogen molecules*, J. Chem. Phys. **136**, 214310 (2012), <http://dx.doi.org/10.1063/1.4722756>.
